# Supplementary material for: A dynamic extreme value model with applications to volcanic eruption forecasting
Source: arXiv:2208.10724 source file (2022-08-23)
Supplement: Supplementary file 1 [file SupplementaryInformation.tex]

\documentclass[journal]{IEEEtran}
%
% If IEEEtran.cls has not been installed into the LaTeX system files,
% manually specify the path to it like:
% \documentclass[journal]{../sty/IEEEtran}

% Some very useful LaTeX packages include:
% (uncomment the ones you want to load)

% *** MISC UTILITY PACKAGES ***
%
%\usepackage{ifpdf}
% Heiko Oberdiek's ifpdf.sty is very useful if you need conditional
% compilation based on whether the output is pdf or dvi.
% usage:
% \ifpdf
%   % pdf code
% \else
%   % dvi code
% \fi
% The latest version of ifpdf.sty can be obtained from:
% http://www.ctan.org/pkg/ifpdf
% Also, note that IEEEtran.cls V1.7 and later provides a builtin
% \ifCLASSINFOpdf conditional that works the same way.
% When switching from latex to pdflatex and vice-versa, the compiler may
% have to be run twice to clear warning/error messages.

% *** CITATION PACKAGES ***
%
\usepackage{cite}
% cite.sty was written by Donald Arseneau
% V1.6 and later of IEEEtran pre-defines the format of the cite.sty package
% \cite{} output to follow that of the IEEE. Loading the cite package will
% result in citation numbers being automatically sorted and properly
% "compressed/ranged". e.g., [1], [9], [2], [7], [5], [6] without using
% cite.sty will become [1], [2], [5]--[7], [9] using cite.sty. cite.sty's
% \cite will automatically add leading space, if needed. Use cite.sty's
% noadjust option (cite.sty V3.8 and later) if you want to turn this off
% such as if a citation ever needs to be enclosed in parenthesis.
% cite.sty is already installed on most LaTeX systems. Be sure and use
% version 5.0 (2009-03-20) and later if using hyperref.sty.
% The latest version can be obtained at:
% http://www.ctan.org/pkg/cite
% The documentation is contained in the cite.sty file itself.

% *** GRAPHICS RELATED PACKAGES ***
%
%\ifCLASSINFOpdf
  \usepackage[pdftex]{graphicx}
\usepackage{amsmath}
% A popular package from the American Mathematical Society that provides
% many useful and powerful commands for dealing with mathematics.
%
% Note that the amsmath package sets \interdisplaylinepenalty to 10000
% thus preventing page breaks from occurring within multiline equations. Use:
\interdisplaylinepenalty=2500
\usepackage[caption=false,font=normalsize,labelfont=sf,textfont=sf, position=top]{subfig}
\usepackage[utf8]{inputenc}
\usepackage{epsf, amssymb}
\usepackage{amsthm}
\usepackage{xcolor, booktabs}
\usepackage{pdflscape}
\usepackage{hyperref, enumitem, rotating}
\usepackage{mathtools}
\usepackage{multicol, multirow}
\usepackage{algpseudocode}
\usepackage{accents}
\usepackage[export]{adjustbox}

% *** Do not adjust lengths that control margins, column widths, etc. ***
% *** Do not use packages that alter fonts (such as pslatex).         ***
% There should be no need to do such things with IEEEtran.cls V1.6 and later.
% (Unless specifically asked to do so by the journal or conference you plan
% to submit to, of course. )

% correct bad hyphenation here
\hyphenation{op-tical net-works semi-conduc-tor}

\begin{document}
%
% paper title
% Titles are generally capitalized except for words such as a, an, and, as,
% at, but, by, for, in, nor, of, on, or, the, to and up, which are usually
% not capitalized unless they are the first or last word of the title.
% Linebreaks \\ can be used within to get better formatting as desired.
% Do not put math or special symbols in the title.
\title{Supplementary information for \\ `A dynamic extreme value model \\ with applications to volcanic eruption forecasting'}
%
%
% author names and IEEE memberships
% note positions of commas and nonbreaking spaces ( ~ ) LaTeX will not break
% a structure at a ~ so this keeps an author's name from being broken across
% two lines.
% use \thanks{} to gain access to the first footnote area
% a separate \thanks must be used for each paragraph as LaTeX2e's \thanks
% was not built to handle multiple paragraphs
% Use e.g. \IEEEmembership{Life~Fellow,~IEEE} if needed.

\author{Michele~Nguyen,~Almut~E.~D.~Veraart,~Benoit~Taisne,~Tan~Chiou~Ting,~and~David~Lallemant~% <-this % stops a space
\thanks{M. Nguyen is with the Asian School of the Environment, Nanyang Technological University (NTU), Singapore 637459 (email: michele.nguyen@ntu.edu.sg).}% <-this % stops a space
\thanks{A. E. D. Veraart is with the Department of Mathematics, Imperial College London, London SW7 2AZ, United Kingdom.}
\thanks{B. Taisne and D. Lallemant are with the Asian School of Environment and also with the Earth Observatory of Singapore, NTU.}% <-this % stops a space
\thanks{Tan Chiou Ting was with the Earth Observatory of Singapore, NTU.}
%\thanks{Manuscript received April 19, 2005; revised August 26, 2015.}
}

% note the % following the last \IEEEmembership and also \thanks - 
% these prevent an unwanted space from occurring between the last author name
% and the end of the author line. i.e., if you had this:
% 
% \author{....lastname \thanks{...} \thanks{...} }
%                     ^------------^------------^----Do not want these spaces!
%
% a space would be appended to the last name and could cause every name on that
% line to be shifted left slightly. This is one of those "LaTeX things". For
% instance, "\textbf{A} \textbf{B}" will typeset as "A B" not "AB". To get
% "AB" then you have to do: "\textbf{A}\textbf{B}"
% \thanks is no different in this regard, so shield the last } of each \thanks
% that ends a line with a % and do not let a space in before the next \thanks.
% Spaces after \IEEEmembership other than the last one are OK (and needed) as
% you are supposed to have spaces between the names. For what it is worth,
% this is a minor point as most people would not even notice if the said evil
% space somehow managed to creep in.

% The paper headers
% E.g. Journal of \LaTeX\ Class Files,~Vol.~14, No.~8, August~2015
\markboth{}%
{Nguyen \MakeLowercase{\textit{et al.}}: Supplementary information for `A dynamic extreme value model for volcanic eruption forecasting'}
% The only time the second header will appear is for the odd numbered pages
% after the title page when using the twoside option.
% 
% *** Note that you probably will NOT want to include the author's ***
% *** name in the headers of peer review papers.                   ***
% You can use \ifCLASSOPTIONpeerreview for conditional compilation here if
% you desire.

% If you want to put a publisher's ID mark on the page you can do it like
% this:
%\IEEEpubid{0000--0000/00\$00.00~\copyright~2015 IEEE}
% Remember, if you use this you must call \IEEEpubidadjcol in the second
% column for its text to clear the IEEEpubid mark.

% use for special paper notices
%\IEEEspecialpapernotice{(Invited Paper)}

% make the title area
\maketitle

% As a general rule, do not put math, special symbols or citations
% in the abstract or keywords.
%\begin{abstract}
%The abstract goes here.
%\end{abstract}

% Note that keywords are not normally used for peerreview papers.
%\begin{IEEEkeywords}
%Extreme value theory, high frequency data, forecasting.
%\end{IEEEkeywords}

% For peer review papers, you can put extra information on the cover
% page as needed:
% \ifCLASSOPTIONpeerreview
% \begin{center} \bfseries EDICS Category: 3-BBND \end{center}
% \fi
%
% For peerreview papers, this IEEEtran command inserts a page break and
% creates the second title. It will be ignored for other modes.
\IEEEpeerreviewmaketitle

\section{A review of short-term eruption forecasting methods}
% The very first letter is a 2 line initial drop letter followed
% by the rest of the first word in caps.
% 
% form to use if the first word consists of a single letter:
% \IEEEPARstart{A}{demo} file is ....
% 
% form to use if you need the single drop letter followed by
% normal text (unknown if ever used by the IEEE):
% \IEEEPARstart{A}{}demo file is ....
% 
% Some journals put the first two words in caps:
% \IEEEPARstart{T}{his demo} file is ....
% 
% Here we have the typical use of a "T" for an initial drop letter
% and "HIS" in caps to complete the first word.
\IEEEPARstart{A}{} volcanic eruption can be defined as ``the explosive ejection of fragmented new magma or older solidified material and/or the effusion of liquid lava" \cite{sigurdsson2015}. Seismic signals, gas emissions, ground deformation, thermal anomalies, ground water, lake or river chemistry, levels and temperature as well as variations in gravitational potential fields can help point towards an impeding eruption \cite{eggers1987, mcnutt1996, battaglia2003, burton2009, segall2013, takahashi2015, demoor2016, poland2020}. Short-term forecasting based on data for these are typically conducted hours to months before an eruption and can provide information on eruption occurrence (i.e. the onset time), location, size, initial style or phase, phase duration and/or the associated hazards \cite{marzocchi2012, whitehead2021}. Thus, short-term forecasting has important implications on evacuation strategies, exclusion zones and deciding upon safe return. 
\\
A recent review paper by \cite{whitehead2021} categorises the many short-term eruption forecasting methods in six broad categories: expert interpretation, event trees, belief networks, process/source models, failure forecasting and machine learning.
\\
Expert interpretation relies on an expert or group of experts to directly interpret the data and give their best estimates of, for example, eruption size, within stated certainty levels \cite{cooke1991, aspinall2010, colson2020}. This is inherently dependent on the skill and knowledge of the experts, who experience high stress levels preceding a possible eruption. Since the estimates are also somewhat subjective, it is difficult to assess their associated uncertainty. Nevertheless, this method is commonly used for volcanoes worldwide.
\\
The second category of methods, event trees, use a tree-like framework to describe how triggering conditions lead to possible outcomes such as eruption size, location and style (see for example, \cite{newhall2002, marzocchi2004, newhall2015}). The probability of moving from one node of the tree to a subsequent one, known as a branch probability, are estimated via empirical data and/or theoretical models. Belief networks have a similar set-up where each node is associated with discrete states for which we estimate probabilities; however, these models are more flexible than event trees: we can incorporate unobservable or latent nodes as well as more interactions between processes \cite{aspinall2003}. A Bayesian approach can be applied to both event trees and belief networks to embed prior information as well as facilitate updating with new data. While associating tree or network nodes with meaningful phenomena and factors influencing an eruption is useful for interpretation, apriori decisions need to be made to decide what these factors should be. There is a need to consciously tailor the models to each volcanic and monitoring system. In addition, many of these models define thresholds at each node to turn continuous parameters into discrete states, losing the richness of the input data. 
\\
Process/source models also make assumptions about unknown subsurface properties and volcanic processes which can differ between volcanoes \cite{hill1977, chouet2003, fournier2007, salvage2016, white2019}. By grouping similar signals from time series data and associating them with source mechanisms, we can track the evolution through the stages of volcanic activity and hence forecast e.g. eruption time. 
\\
Another well-established method is failure forecasting \cite{voight1988, sparks2003, bell2011, bell2013, bevilacqua2019}. For any acceleratory geophysical precursor such as deformation or seismicity, we can fit a curve to the plot of its rate against time based on an empirical law of material failure. This enables us to estimate failure time as the time at which acceleration reaches infinity. While failure forecasting is relatively easy to implement, one needs to choose appropriate signals to monitor and relate their failure time to the eruption onset time. This would depend on for example, sensor location and depth. It can also be difficult to accurately quantify the uncertainty associated with the estimated onset time because the non-Gaussian model residuals which result are in conflict with the normality assumption underlying the regression used to fit the model. Other limitations include sensitivity to data truncation and signal fluctuations or deceleration which could occur in the immediate period before an eruption. 
\\
The method we propose in this paper falls under the category of machine learning. By using mathematical algorithms, we can learn patterns from data, including complex associations which we may not identify by eye or have imagined beforehand. While machine learning methods such as multi-layer perception, neural networks, radial basis functions, CART regression or decision trees and support vector regression have been applied to eruption forecasting, their full and varied potential have not yet been realised \cite{Malfante2018, carniel2020, whitehead2021}. 

\section{Examining the sufficiency of a constant GPD model}

\begin{figure*}[!t]
\centering
\subfloat[Autocorrelation of Pearson residuals]{
\includegraphics[width=3.5in,valign=t]{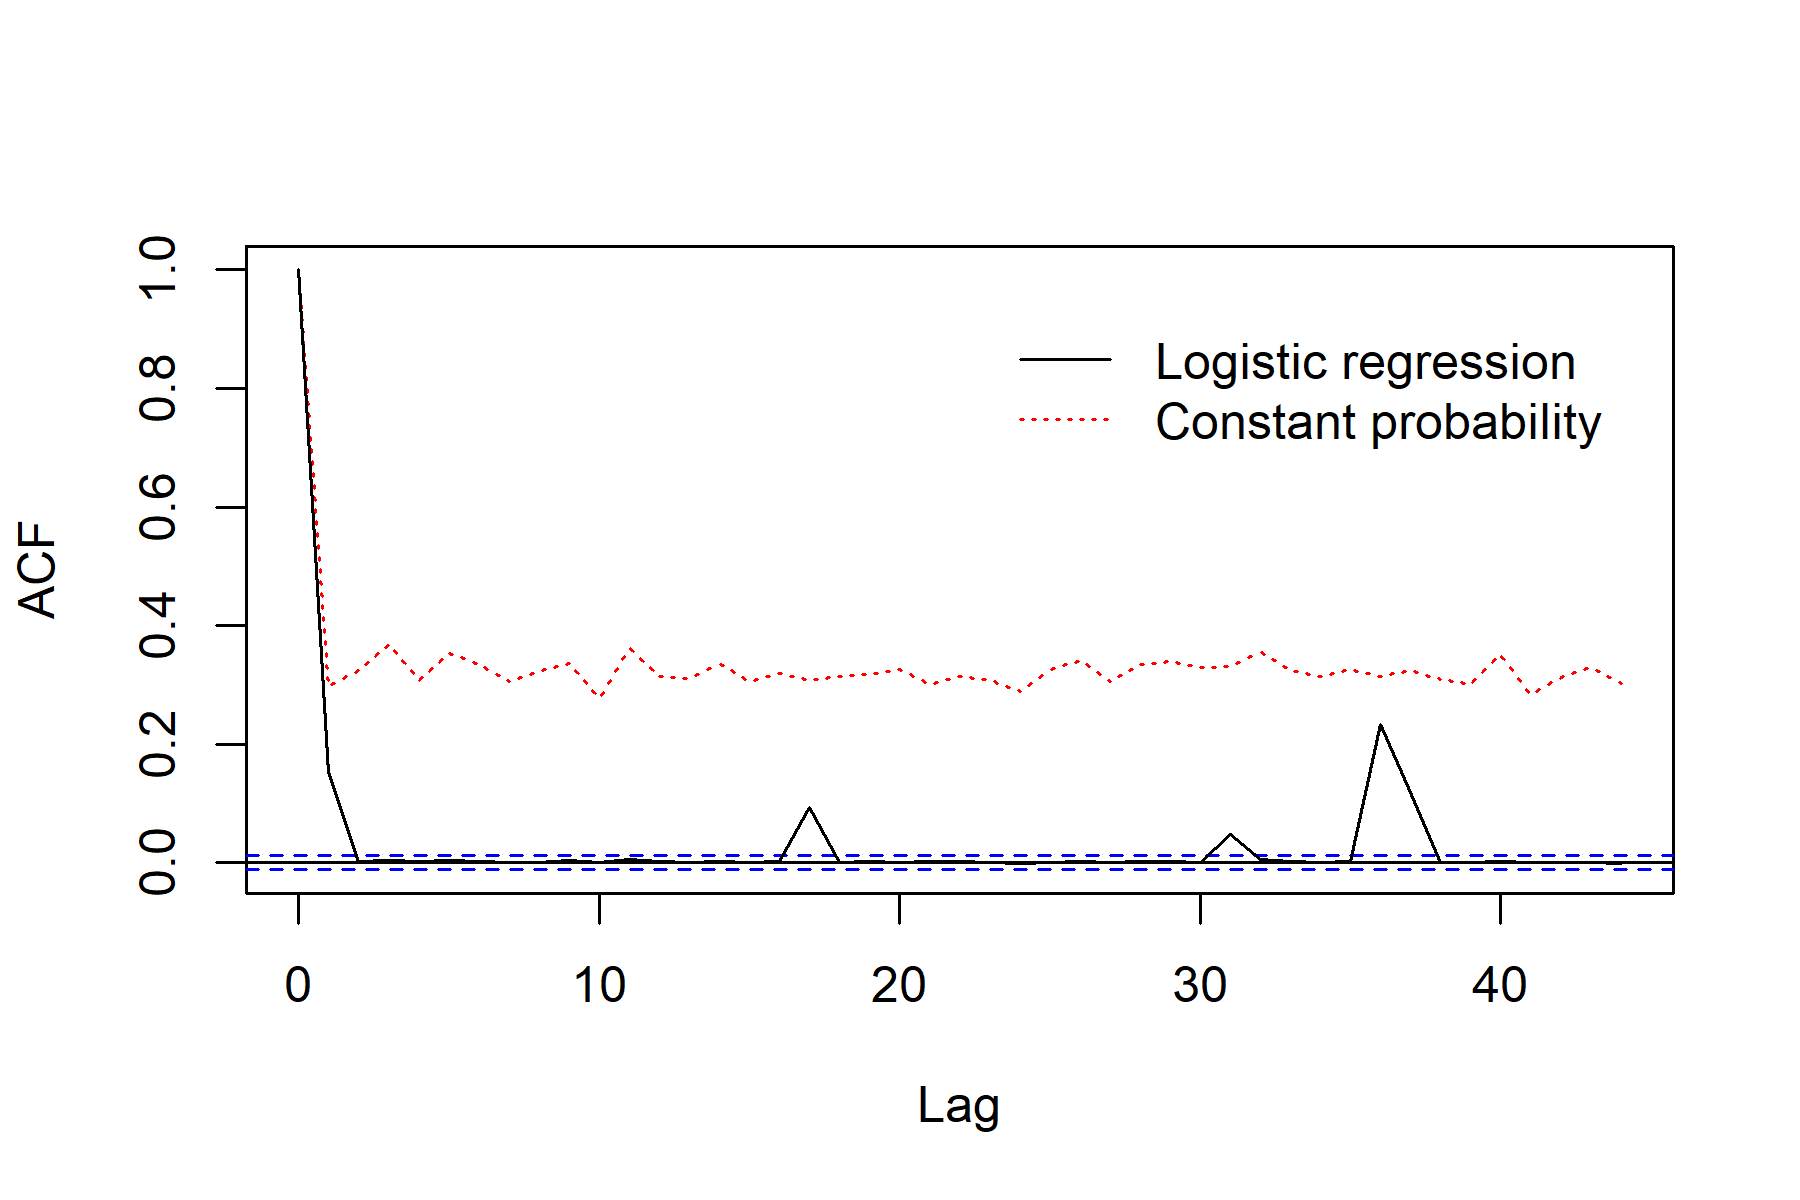}%
\label{fig:acf_exceed_15_1}}
\hfil
\subfloat[Autocorrelation of excess residuals]{\includegraphics[width=3.5in,valign=t]{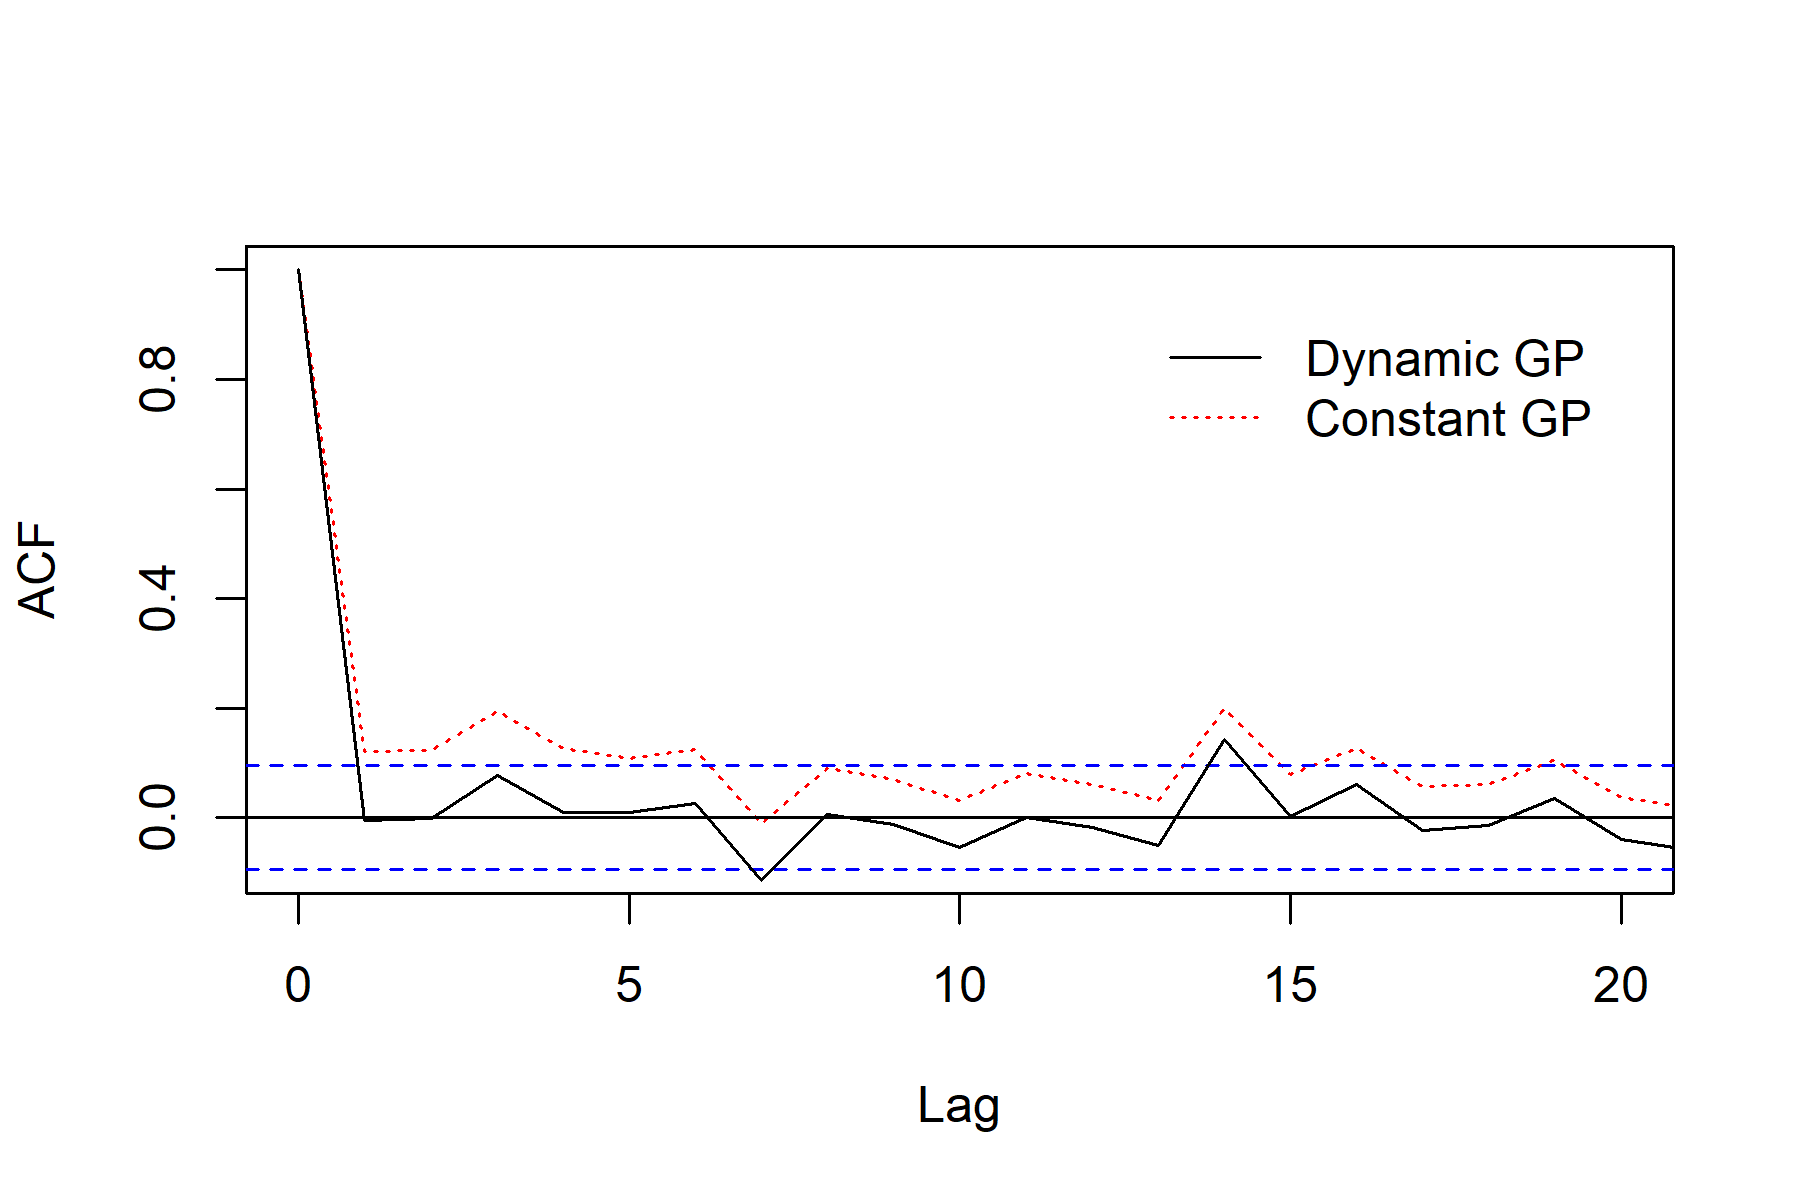}%
\label{fig:acf_excess_15_1}}
\caption{(a) Estimated autocorrelation function (ACF) for the Pearson residuals from the fitted logistic regression (black) and the constant probability model (red dotted); (b) Estimated autocorrelation function (ACF) for the residuals from the fitted GPD regression (black) and the constant GP model (red dotted). In the ACF plots, the blue dashed lines denote the 95\% Barlett confidence intervals for white noise.}
\label{fig_acf_15}
\end{figure*}

\begin{figure*}[!t]
\centering
\subfloat[Training event 1: ACF of Pearson residuals]{\includegraphics[width=3.5in,valign=t]{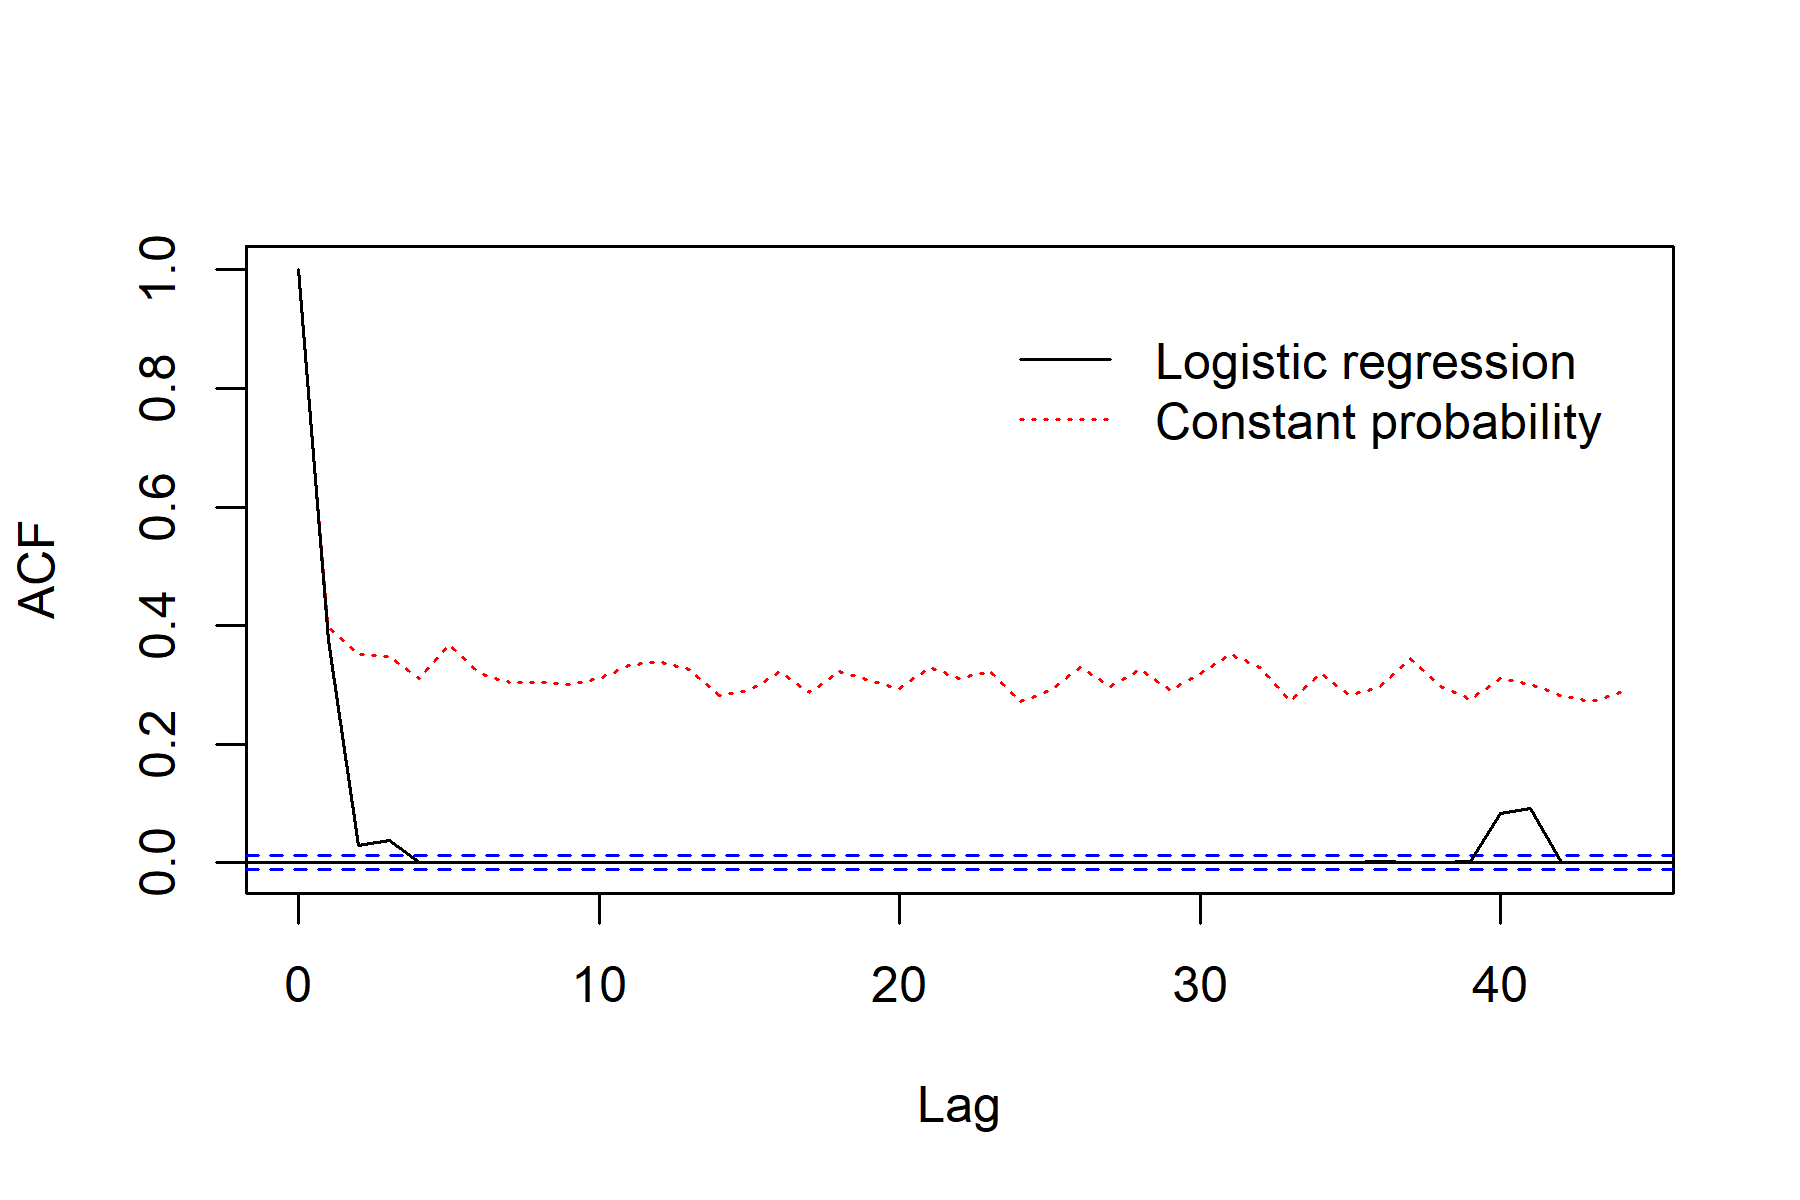}%
}
\hfil
\subfloat[Training event 1: ACF of excess residuals]{\includegraphics[width=3.5in,valign=t]{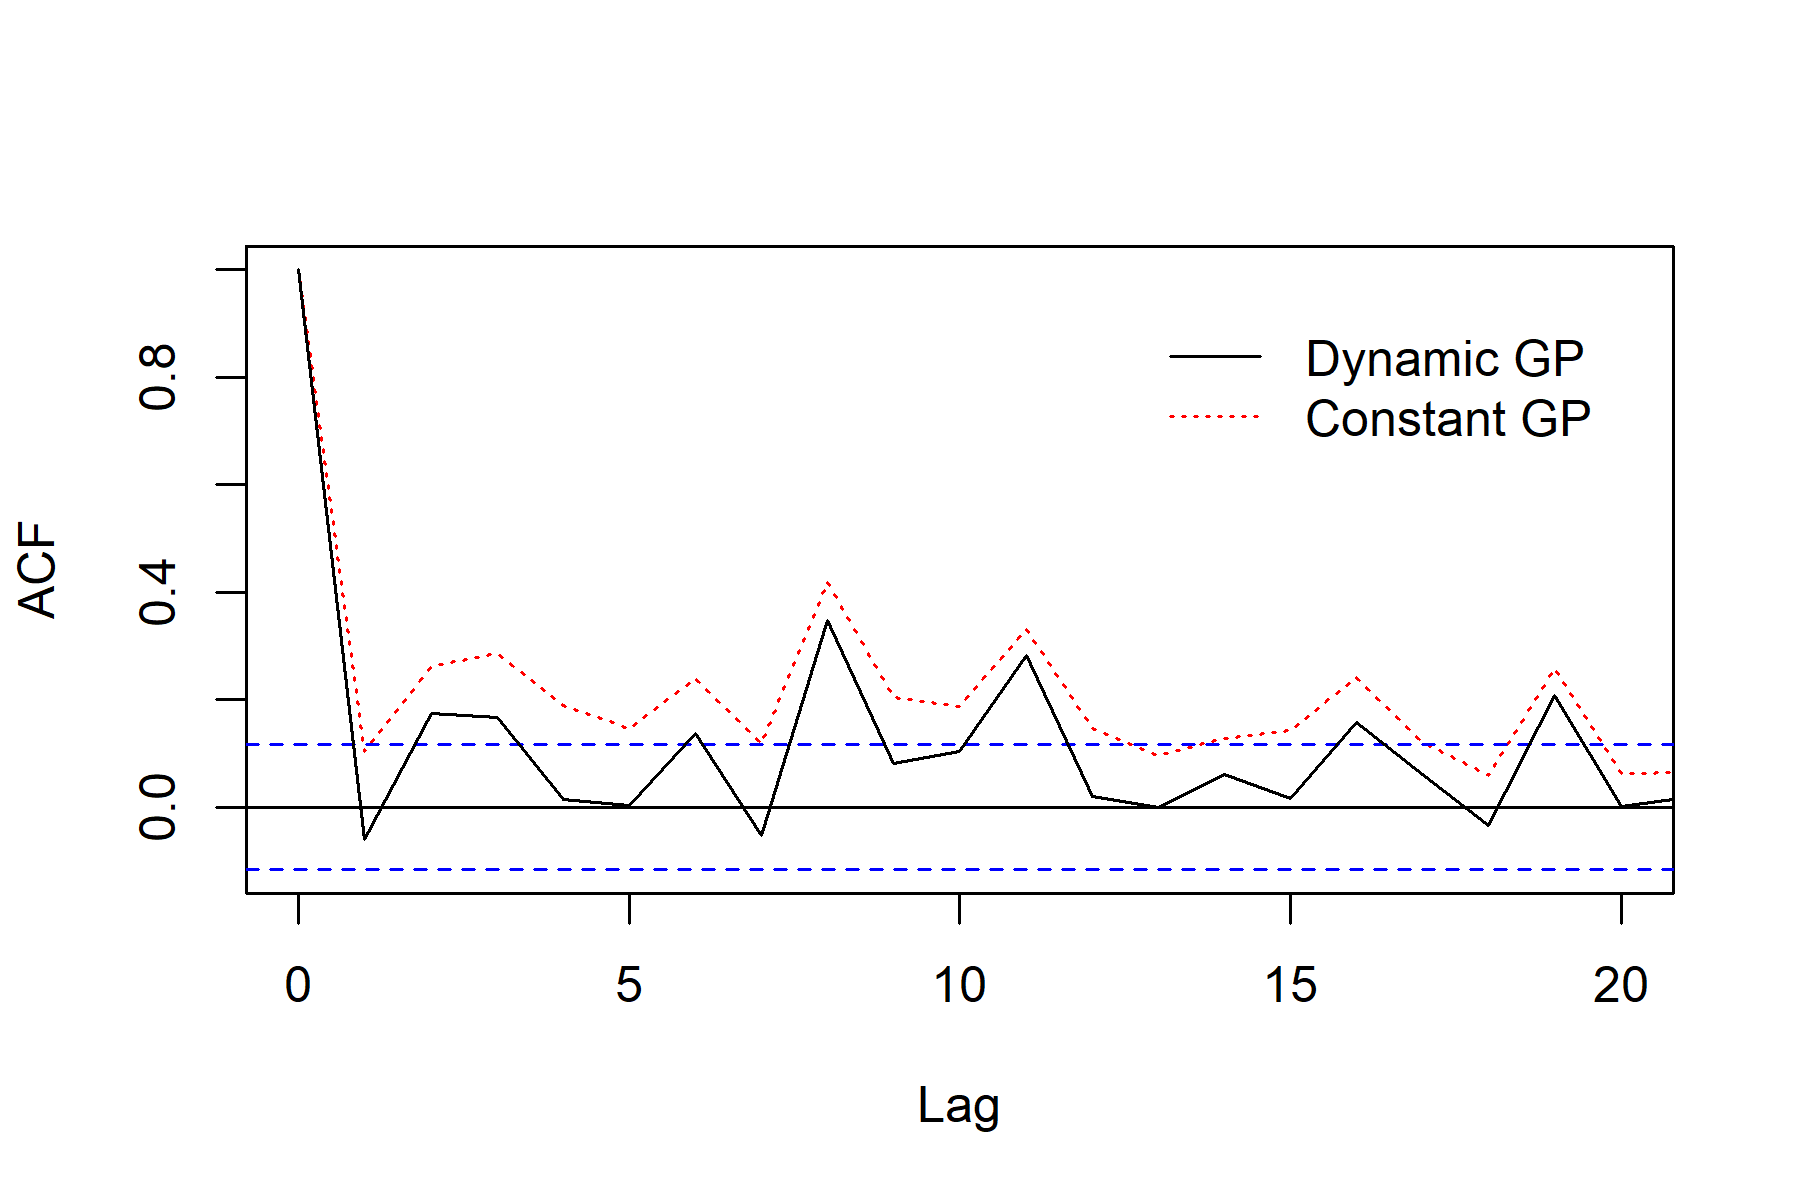}%
}
\\
\subfloat[Training event 2: ACF of Pearson residuals]{\includegraphics[width=3.5in,valign=t]{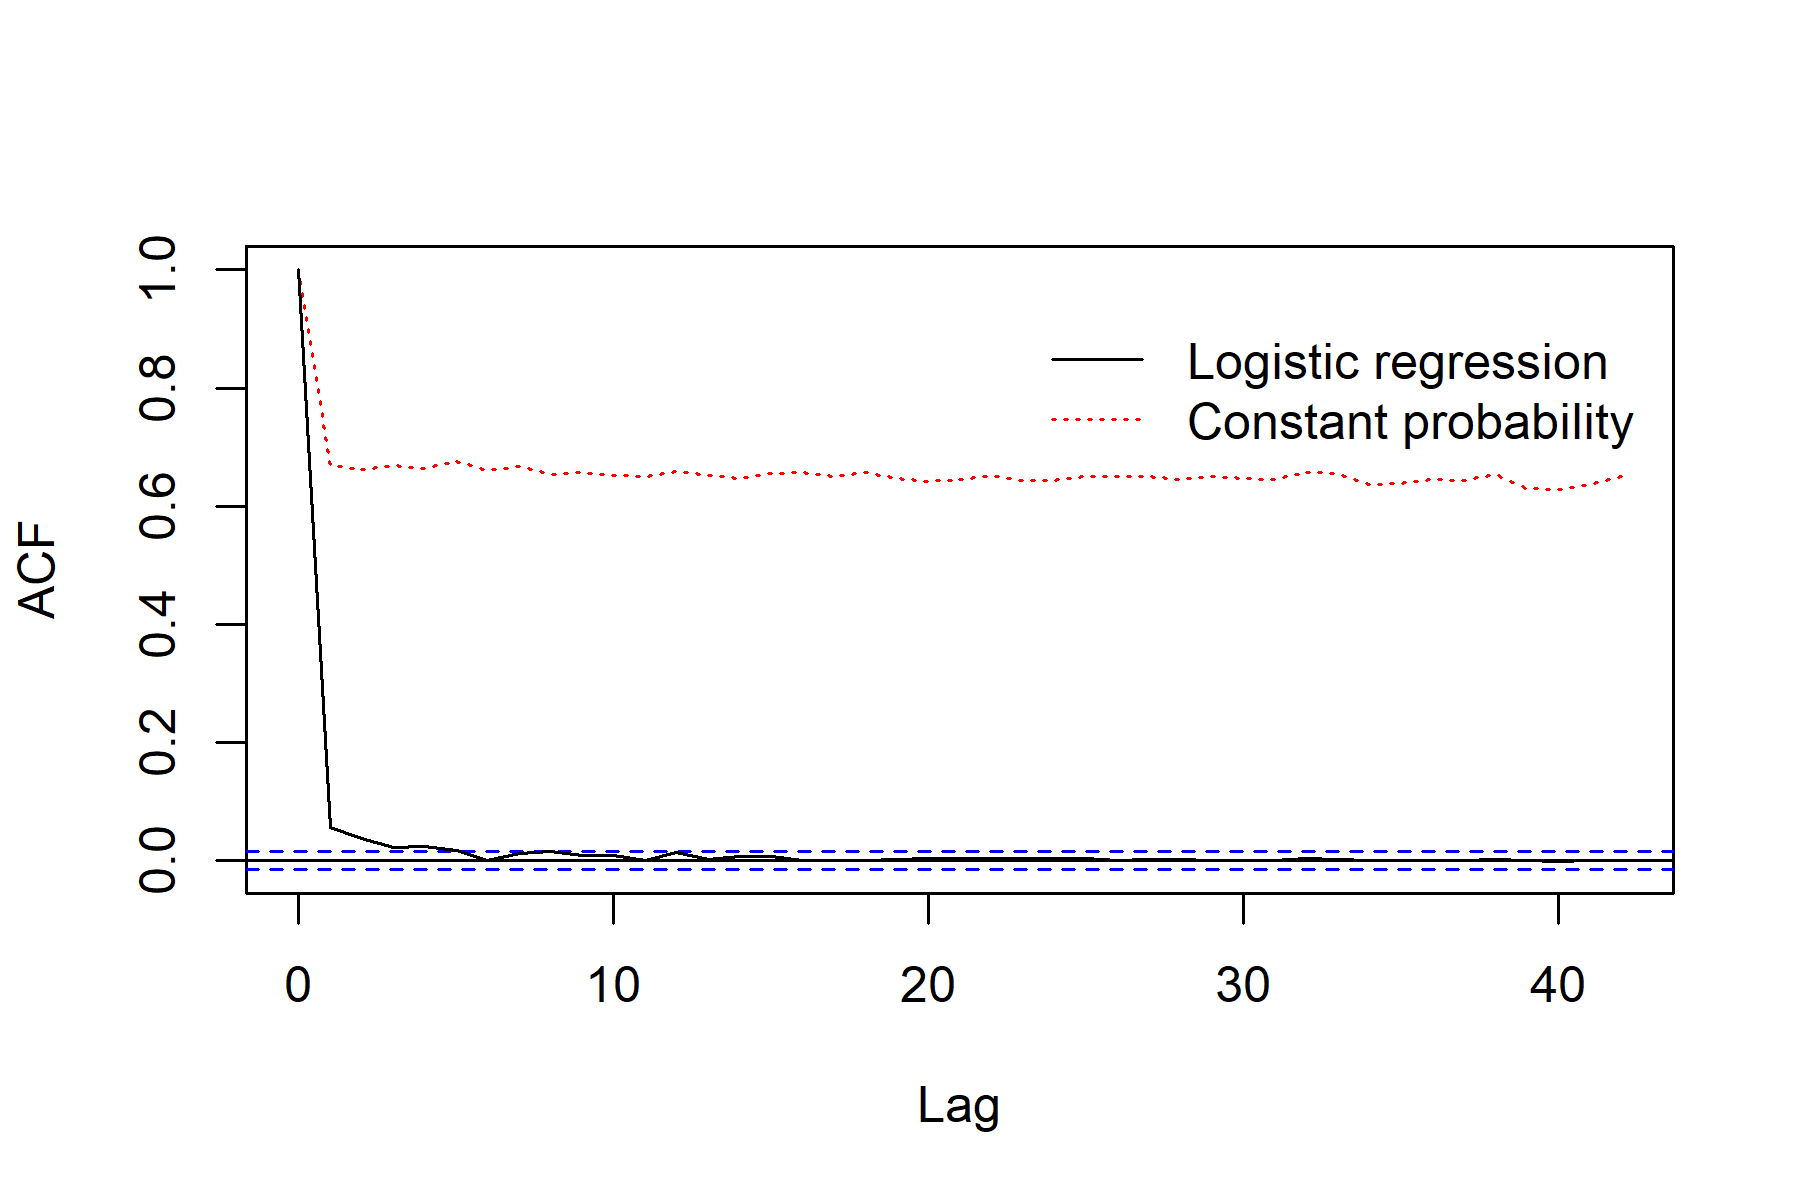}%
}
\hfil
\subfloat[Training event 2: ACF of excess residuals]{\includegraphics[width=3.5in,valign=t]{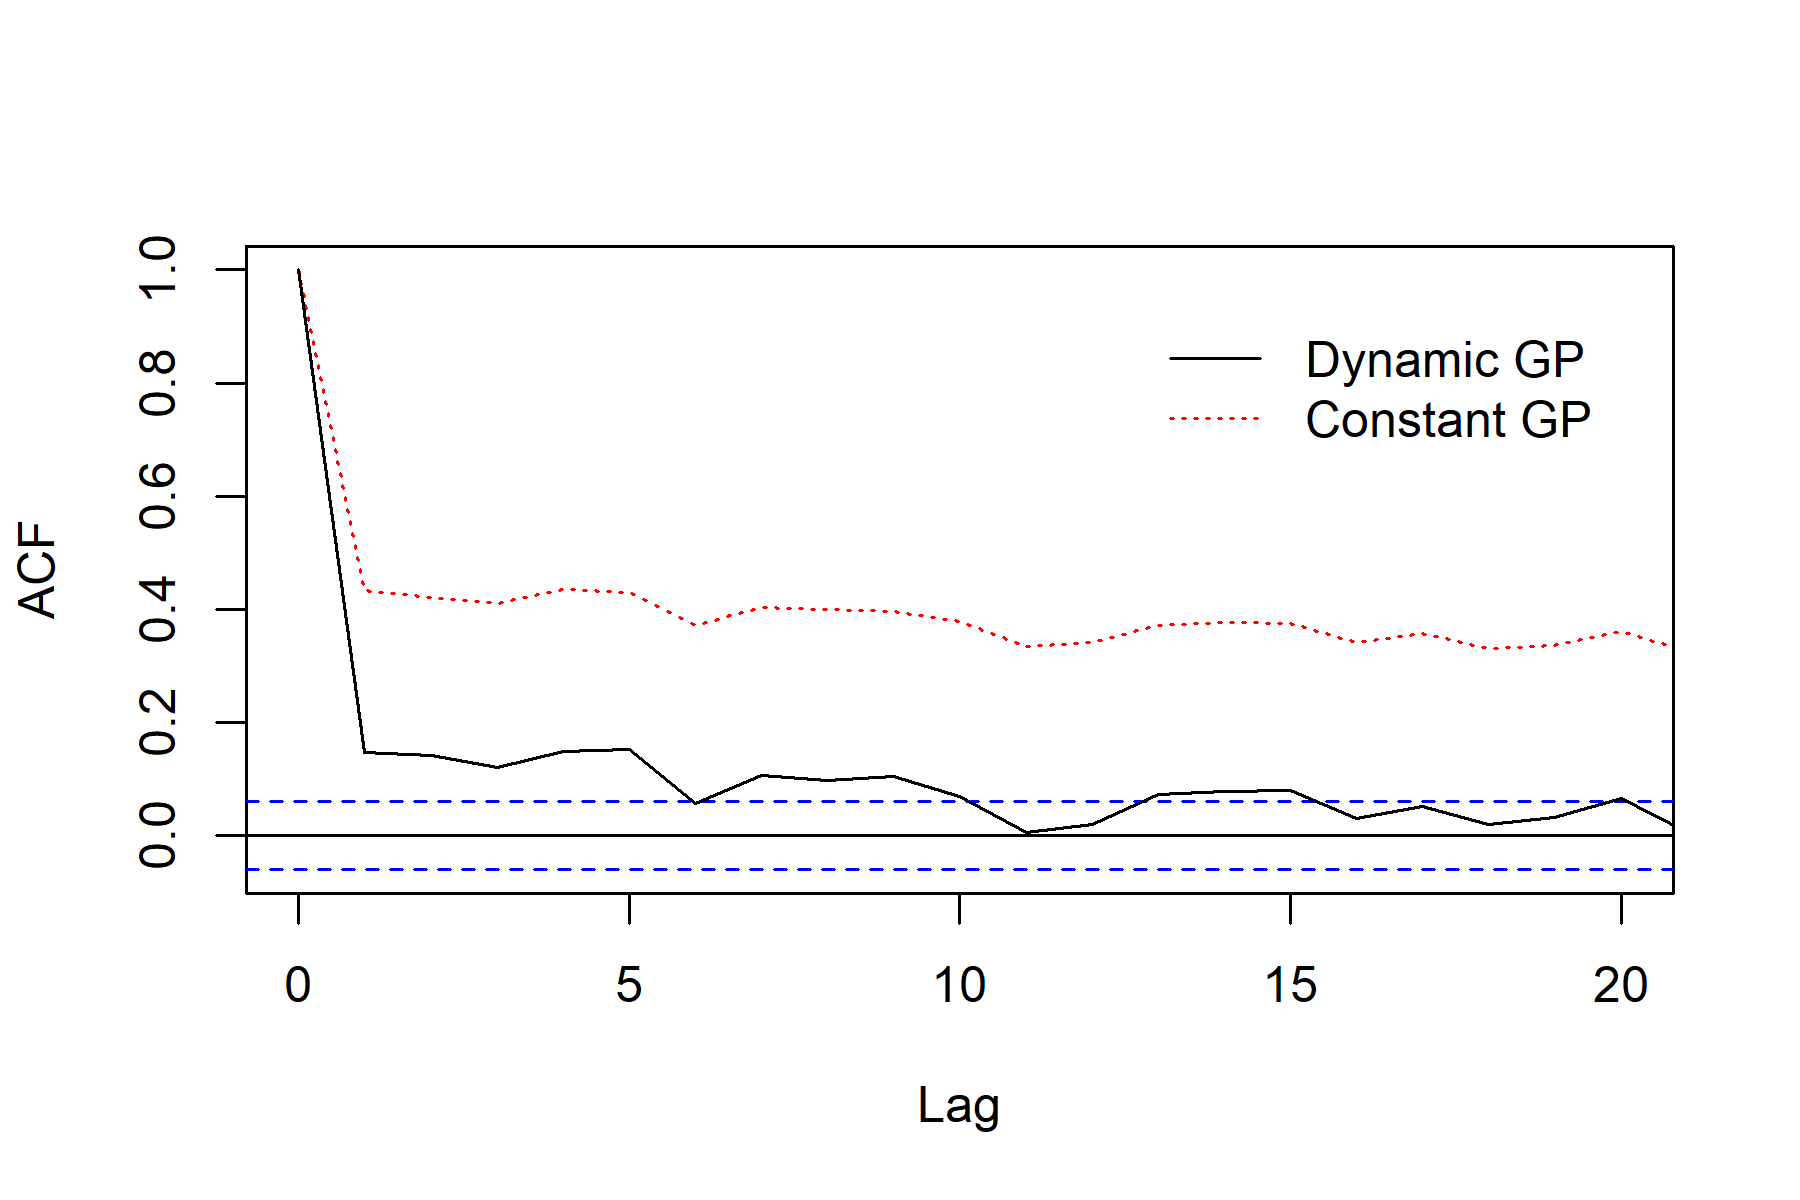}%
}
\\
\subfloat[Training event 3: ACF of Pearson residuals]{\includegraphics[width=3.5in,valign=t]{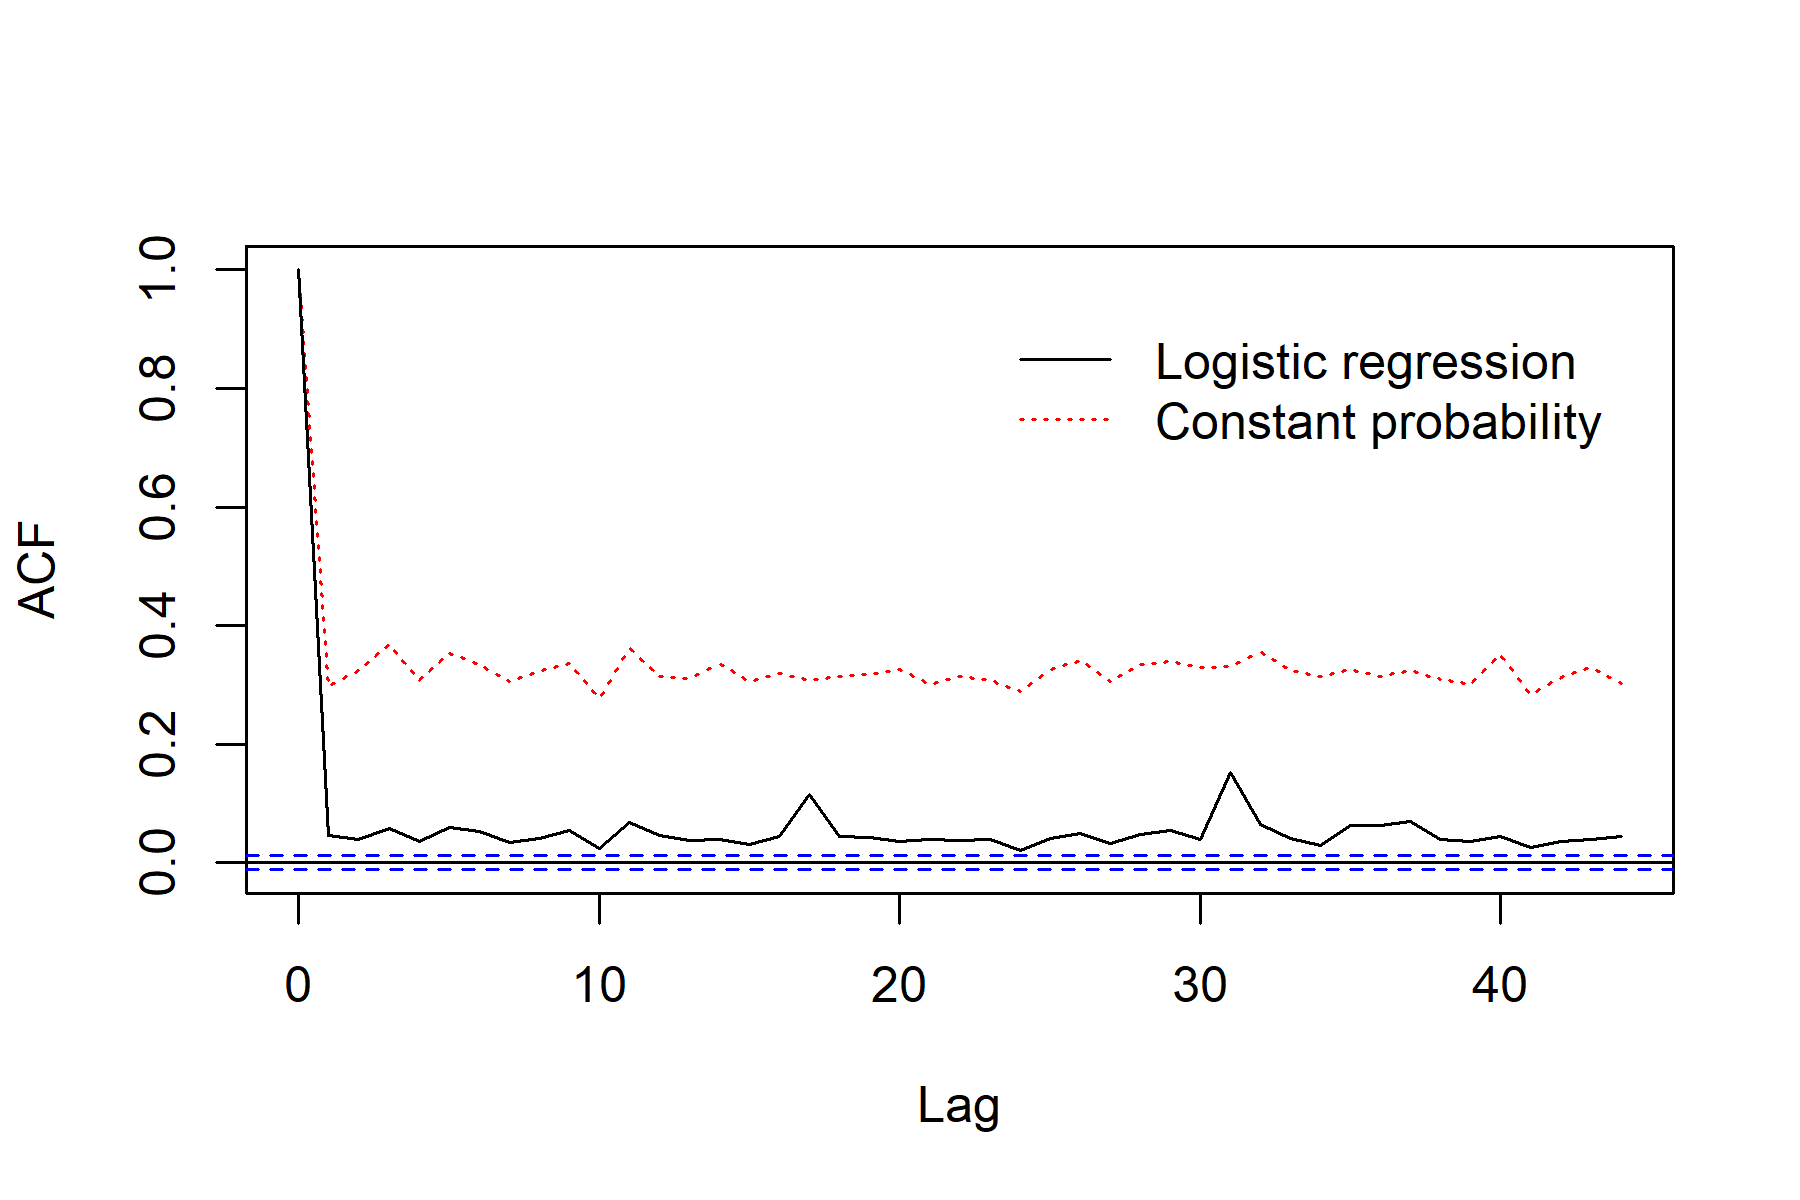}%
}
\hfil
\subfloat[Training event 3: ACF of excess residuals]{\includegraphics[width=3.5in,valign=t]{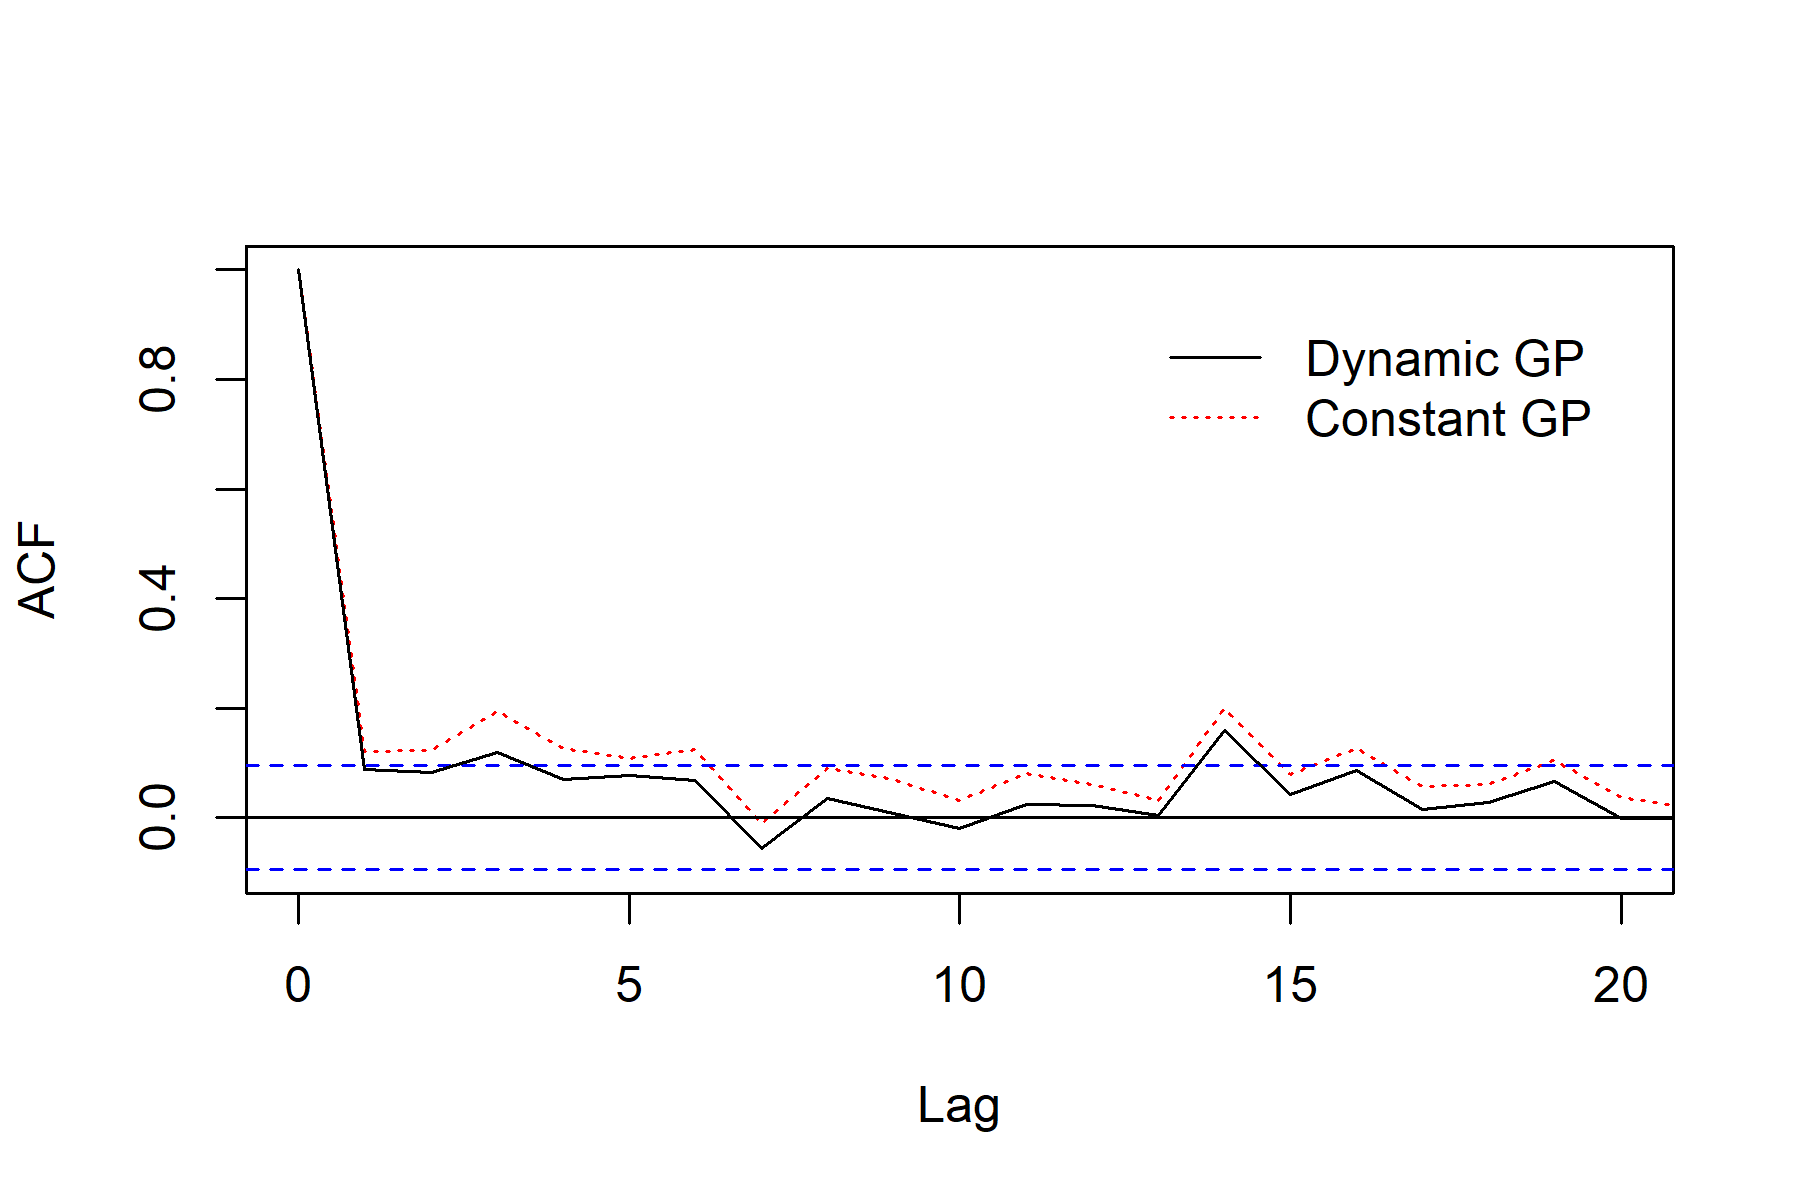}%
}
\caption{For model fitted using all three training events and using the lowest threshold estimate: Estimated autocorrelation function (ACF) for the Pearson residuals from the fitted logistic regression (black) and the constant probability model (red dotted) in Plots (a), (c) and (e). Estimated autocorrelation function (ACF) for the residuals from the fitted GPD regression (black) and the constant GP model (red dotted) in Plots (b), (d) and (f). In the ACF plots, the blue dashed lines denote the 95\% Barlett confidence intervals for white noise.}
\label{fig_acf_15_lbound}
\end{figure*}

In Section III of the main paper, we showed how we can use the dynamic extreme model to forecast volcanic eruptions using data from the January 2010 eruption event (Training set 3). For this dataset, we concluded that while the computed covariates were useful for explaining the temporal dependence in threshold exceedances, there was less temporal dependence in the excesses. Hence, there was no benefit of using covariates to inform a dynamic Generalised Pareto Distribution (GPD) for the excesses and a constant GPD would have sufficed. This was not the case when we later trained the model on multiple events. Here, we provide the plots to support these conclusions.
\\
Figure \ref{fig:acf_exceed_15_1} shows the estimated autocorrelation against temporal lag for the Pearson residuals from the fitted logistic regression and the constant probability model. Since the black line is generally lower than the red line, the residuals exhibit less correlation when conditioned on the chosen covariates. This indicates that the conditional independence assumption in the logistic regression is better adhered to than in the constant probability model. 
\\
In contrast, Figure \ref{fig:acf_excess_15_1} shows the estimated autocorrelations of the excess residuals from the dynamic GPD regression and the constant GPD model. The excess residuals are defined as the differences between the observed excesses and the predicted means. The plot shows that the residuals from a constant GPD model do not exhibit much autocorrelation so there is no incentive to model it dynamically. This is despite the fact that the AIC for the constant GPD model is higher than that for the dynamic GPD model (1663.599 versus 1614.226). 
\\
When we train the model on multiple events, we see that there is autocorrelation in the Pearson residuals prior to fitting the logistic regression as well as autocorrelation in the excess residuals prior to modelling the excesses with the GPD regression (seen most strongly for Training events 1 and 2). The corresponding plots showing the benefits of modelling these autocorrelations with the logistic regression and GPD regressions are shown in Figure \ref{fig_acf_15_lbound}. These dynamic models reduce the residual autocorrelations substantially (the black lines generally lie much lower than the red lines).

\section{Signal and envelope indices for training events and test non-events}

The time series plots for the raw signal and 1-5Hz envelope indices for Training events 1 and 2, Test event and Test non-events 1, 2 and 3 are given in Figures \ref{fig_train1}-\ref{fig_nonevent3}.

\begin{figure*}[!t]
\centering
\subfloat[Signal]{\includegraphics[width=3.5in,valign=t, trim = {0.8cm 0 0cm 0}]{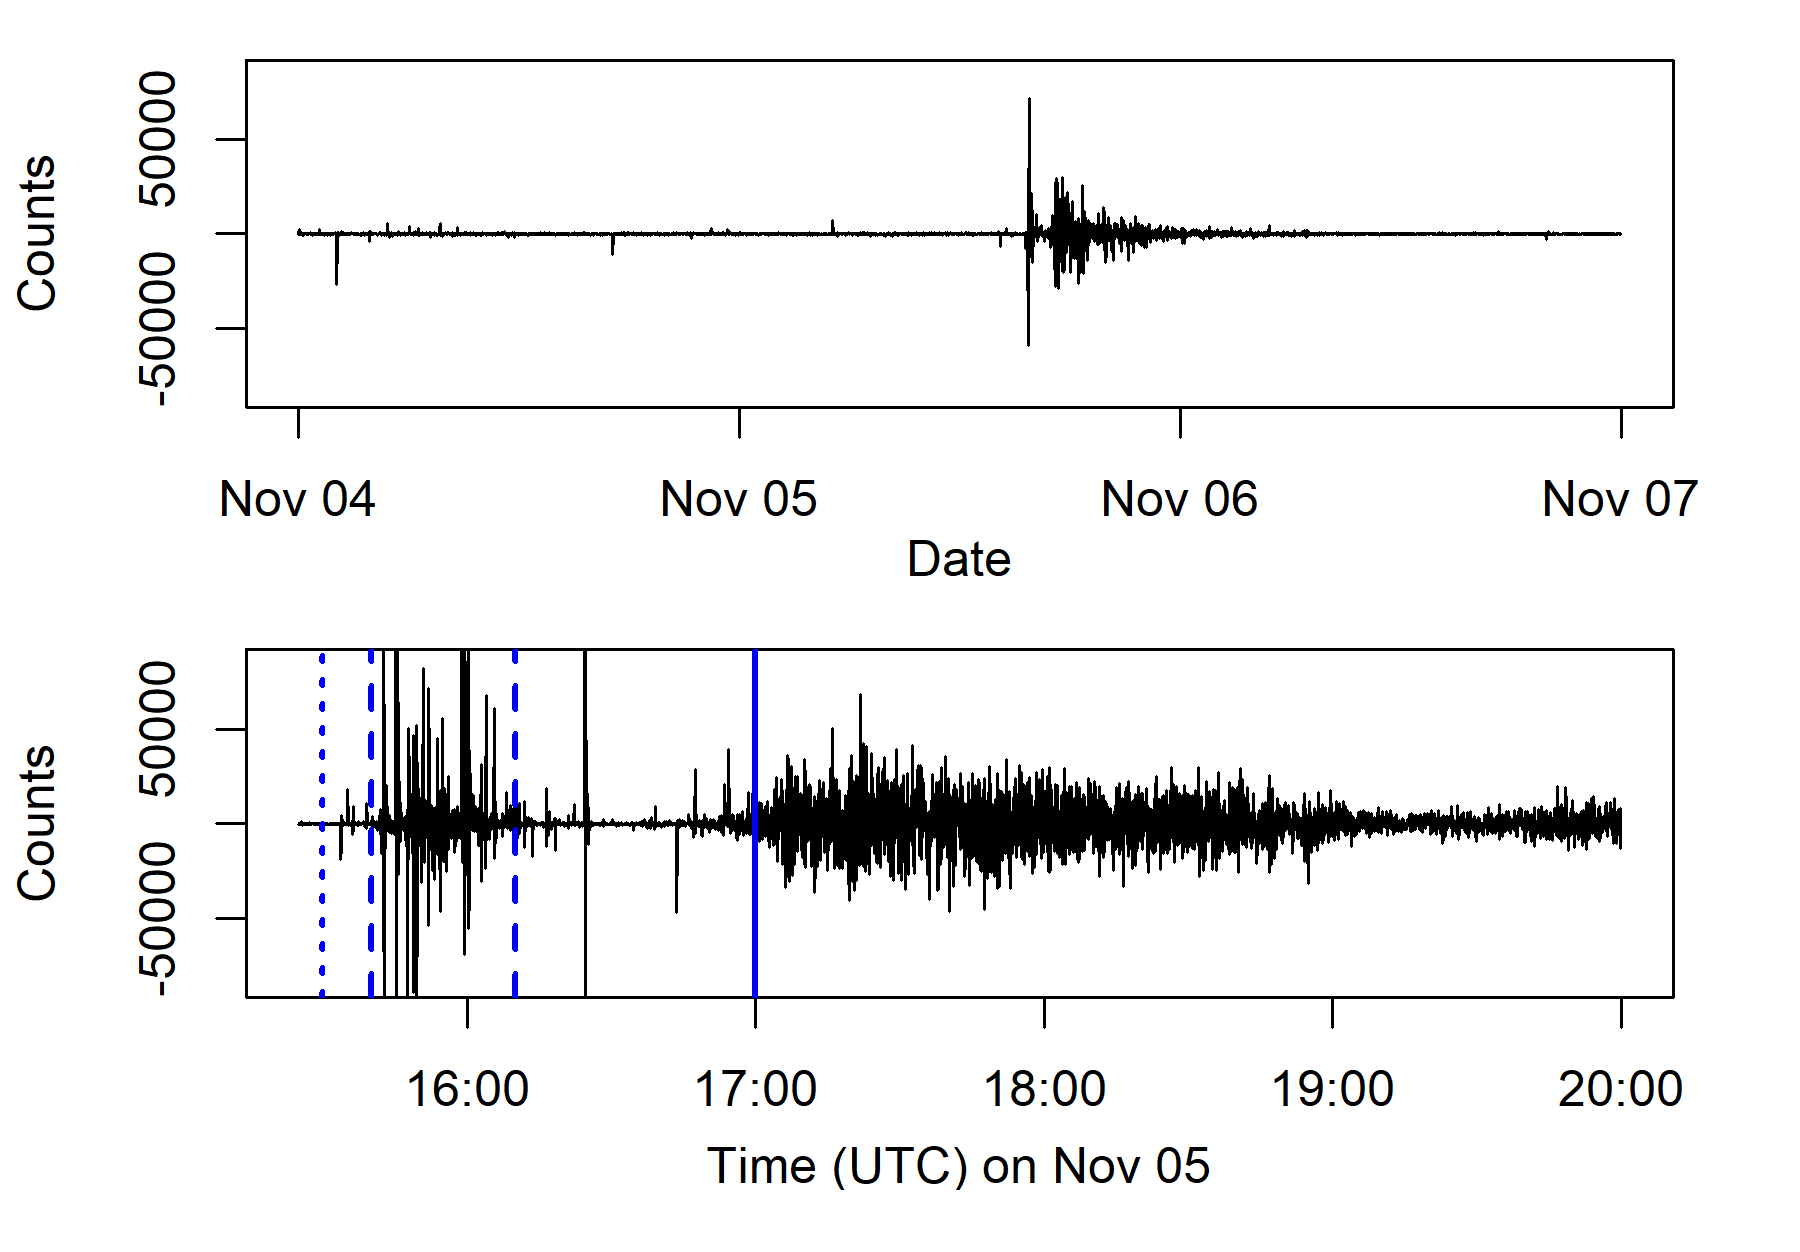}%
\label{fig:train1_signal}}
\hfil
\subfloat[Envelope index]{\includegraphics[width=3.5in,valign=t, trim = {0cm 0 0.8cm 0}]{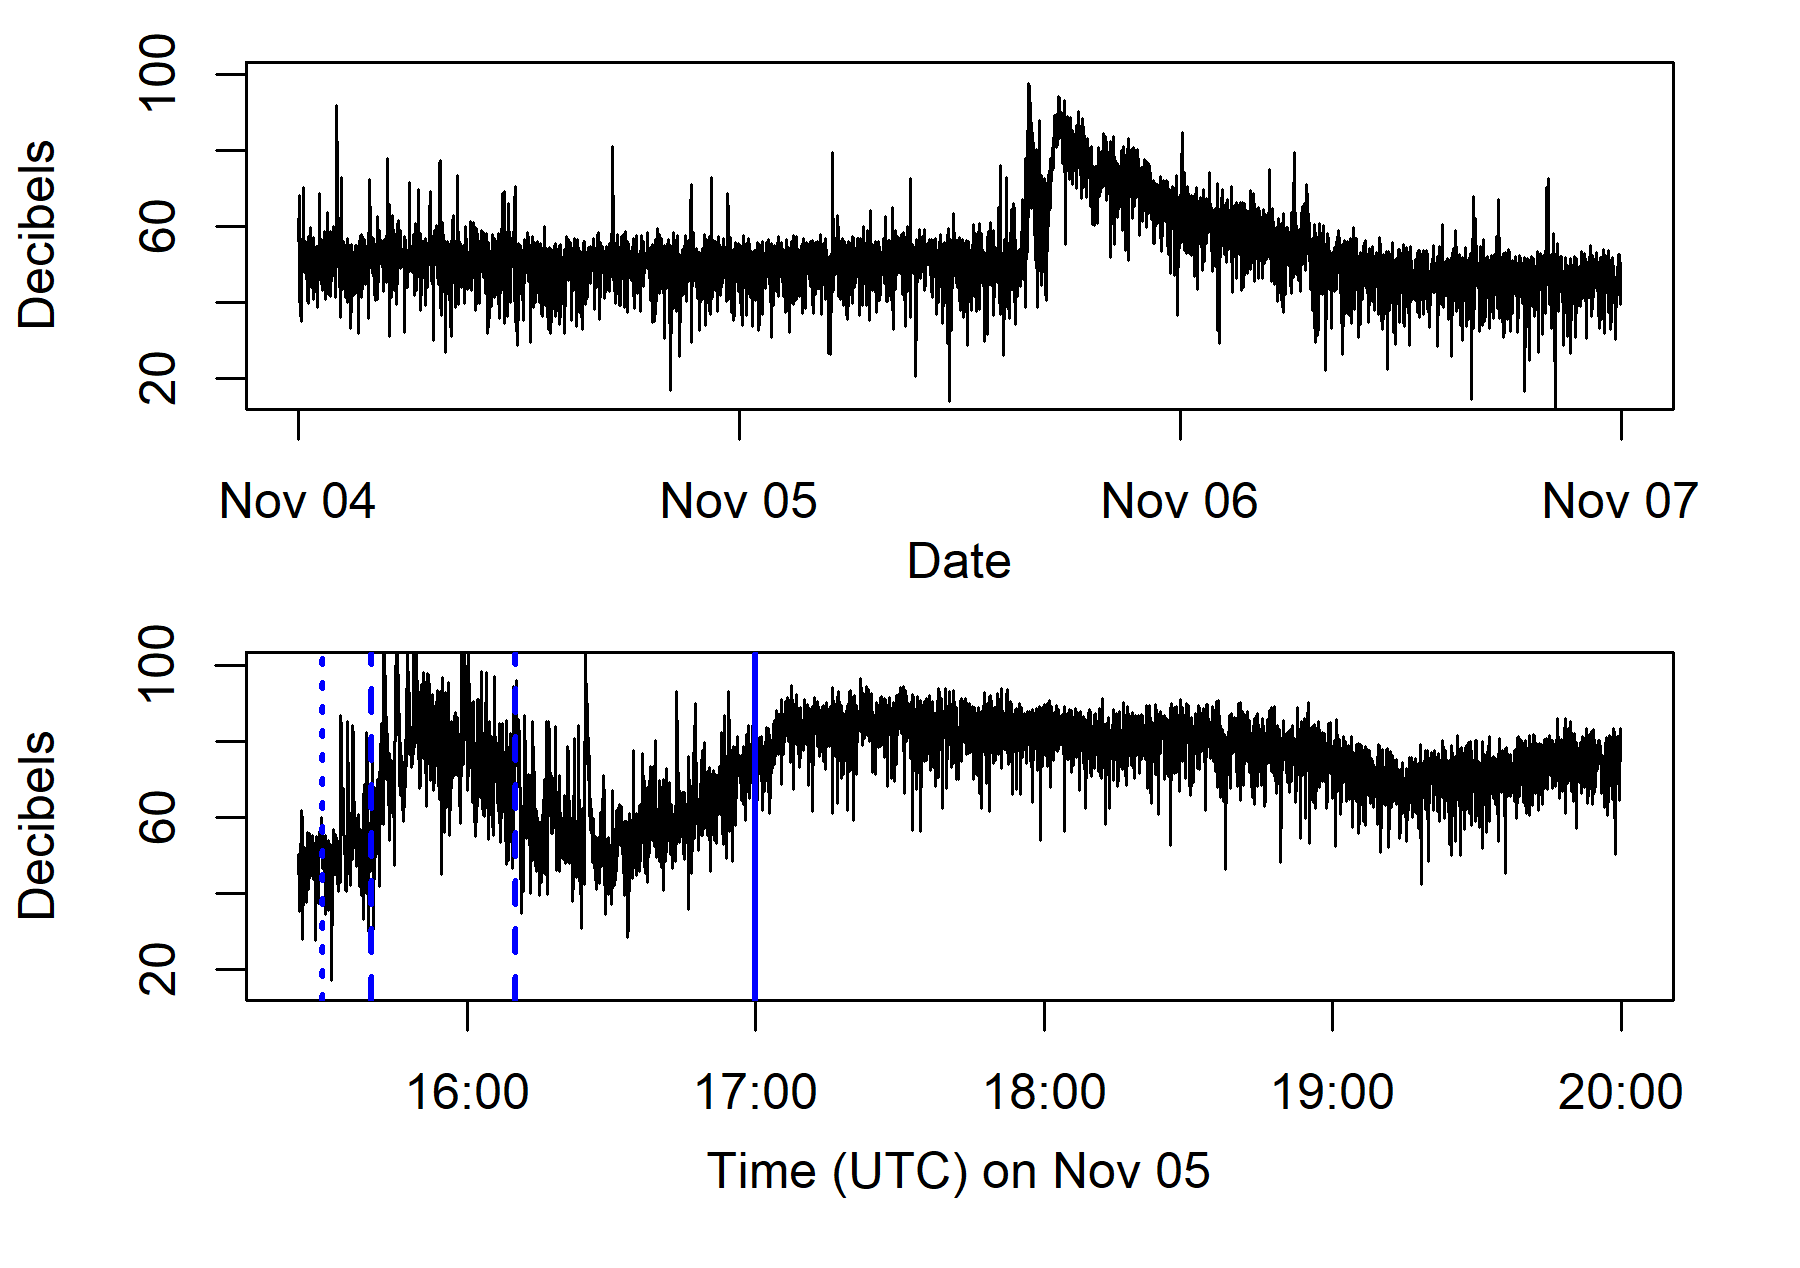}%
\label{fig:train1_envelope}}

\caption{Training set 1: (a) Seismic signal for the 1-5Hz frequency band and (b) the corresponding envelope index in decibels (dB) for the November 2009 eruption event. The dotted, dashed and bold blue vertical lines denote the start of the seismic crisis, the start and end of the seismic swarm and the eruption onset respectively. Note that the time series are deciminated such as every 5184th reading and every 330th reading are shown for the top and bottom plots respectively.}
\label{fig_train1}
\end{figure*}

\begin{figure*}[!t]
\centering
\subfloat[Signal]{\includegraphics[width=3.5in,valign=t, trim = {0.8cm 0 0cm 0}]{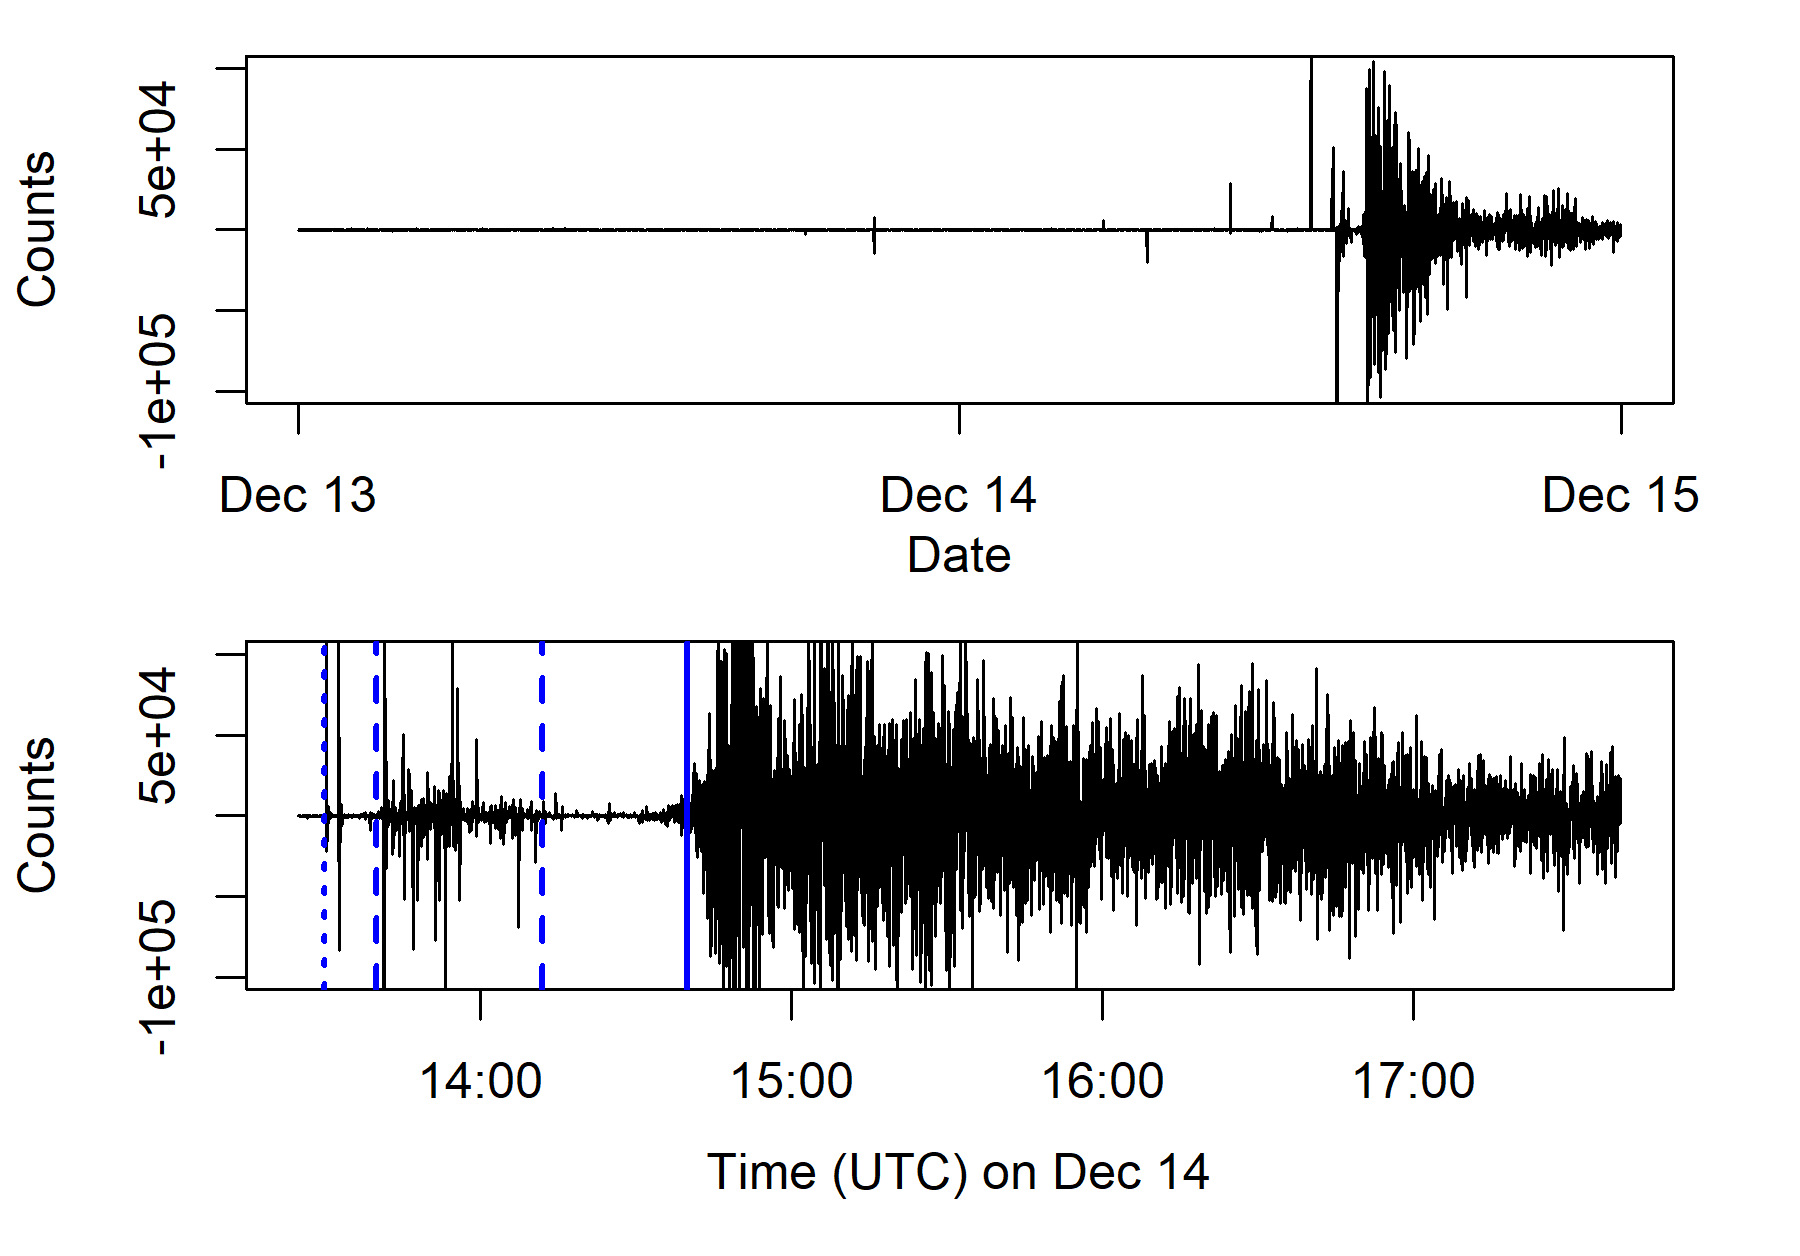}%
\label{fig:train2_signal}}
\hfil
\subfloat[Envelope index]{\includegraphics[width=3.5in,valign=t, trim = {0cm 0 0.8cm 0}]{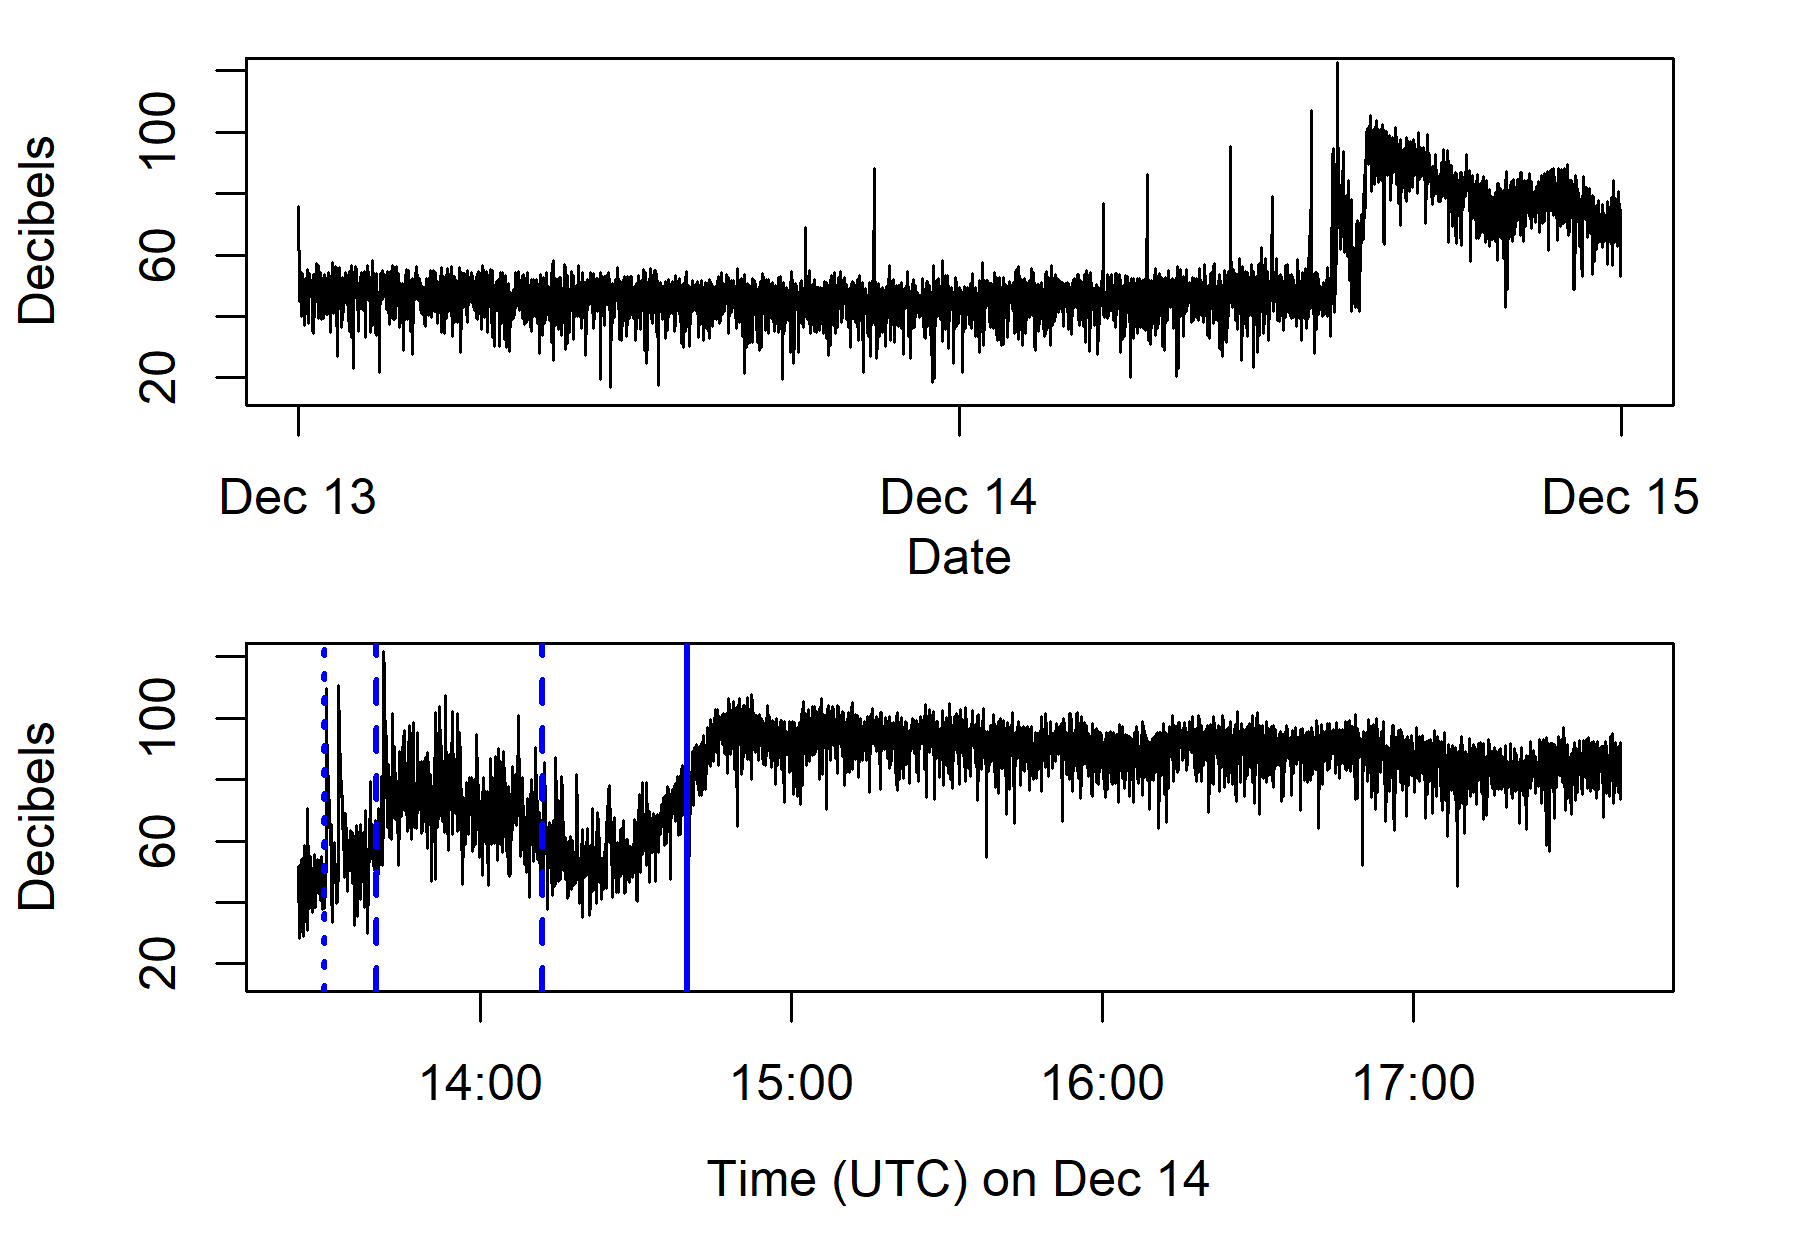}%
\label{fig:train2_envelope}}

\caption{Training set 2: (a) Seismic signal for the 1-5Hz frequency band and (b) the corresponding envelope index in decibels (dB) for the December 2009 eruption event. The dotted, dashed and bold blue vertical lines denote the start of the seismic crisis, the start and end of the seismic swarm and the eruption onset respectively. Note that the time series are deciminated such as every 3456th reading and every 306th reading are shown for the top and bottom plots respectively.}
\label{fig_train2}
\end{figure*}

\begin{figure*}[!t]
\centering
\subfloat[Signal]{\includegraphics[width=3.5in,valign=t, trim = {0.8cm 0 0cm 0}]{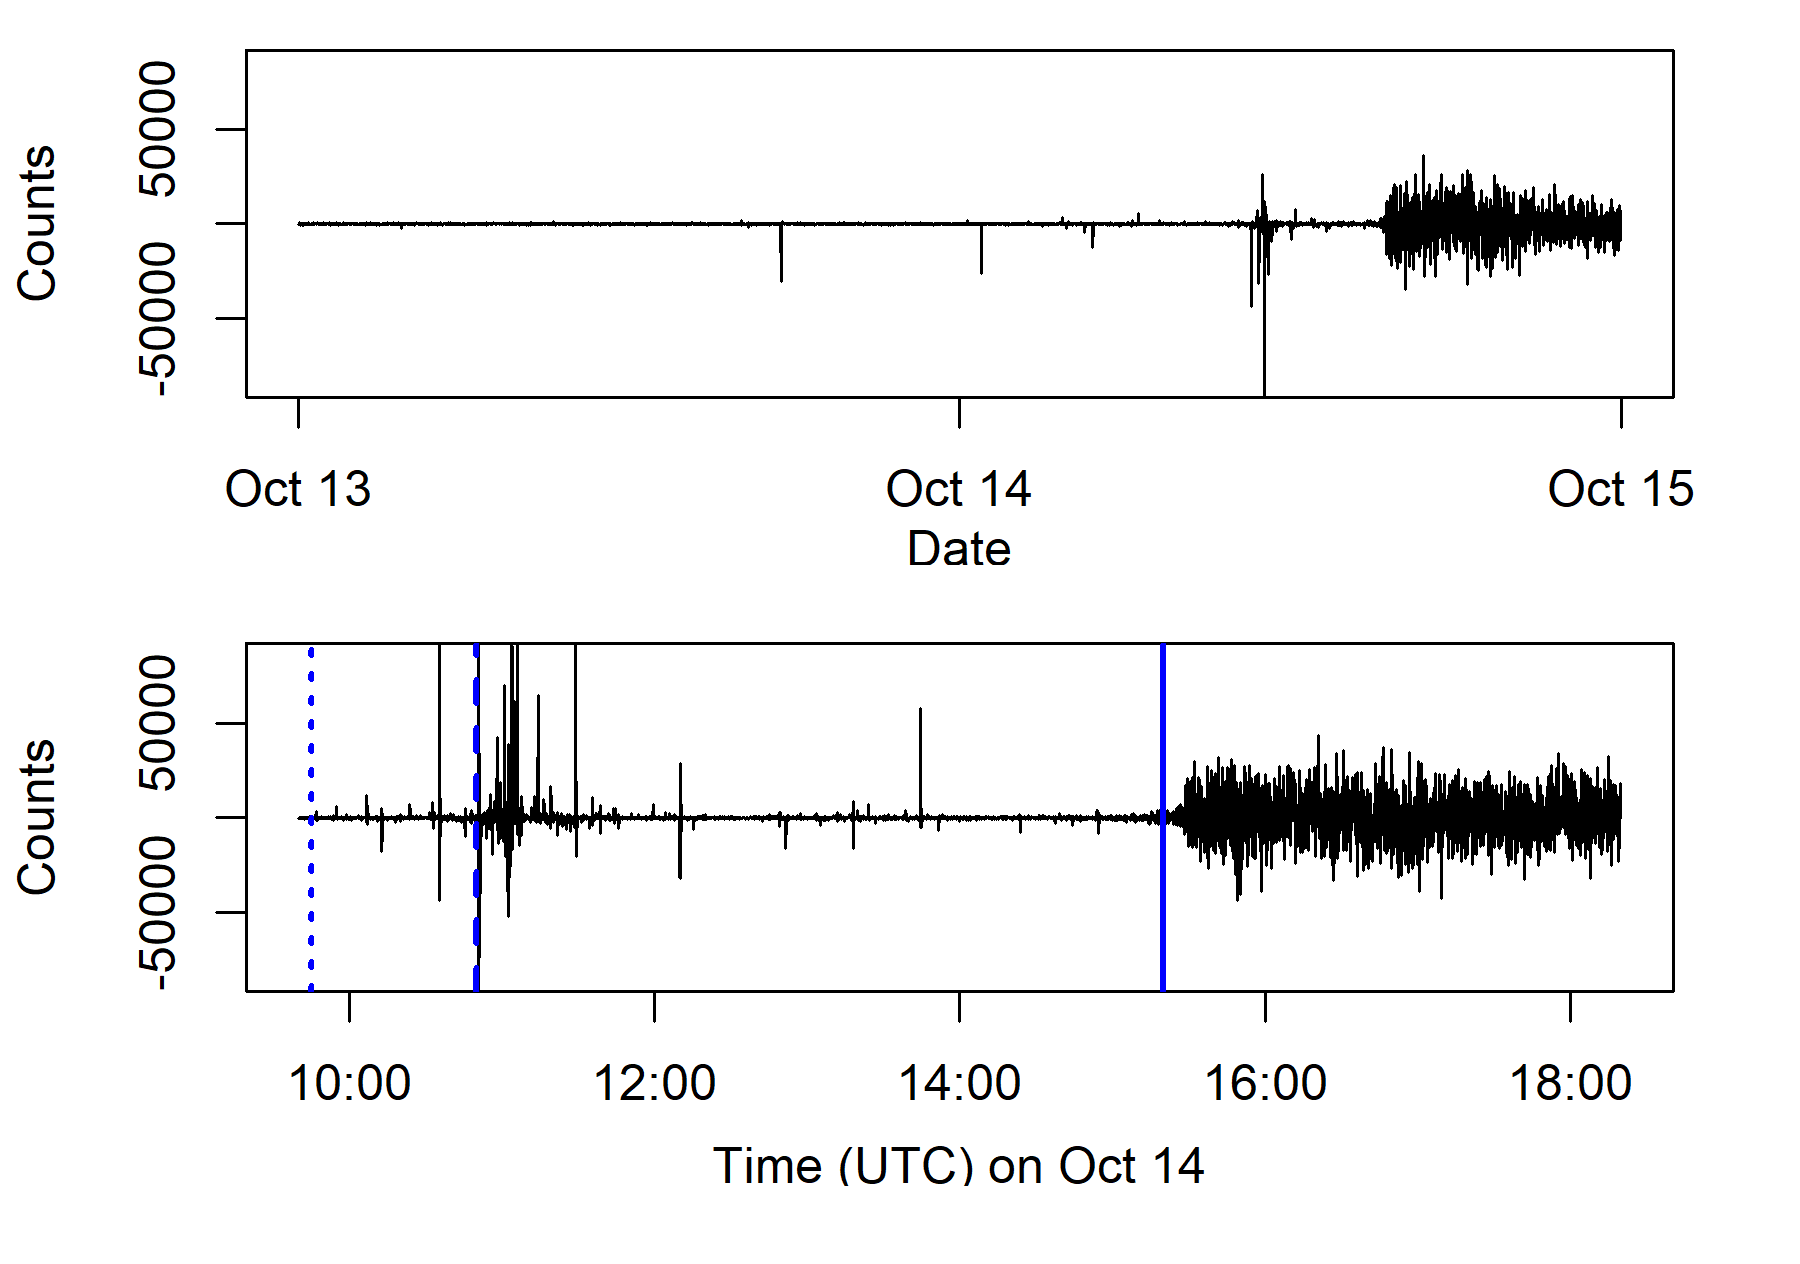}%
\label{fig:test_signal}}
\hfil
\subfloat[Envelope index]{\includegraphics[width=3.5in,valign=t, trim = {0cm 0 0.8cm 0}]{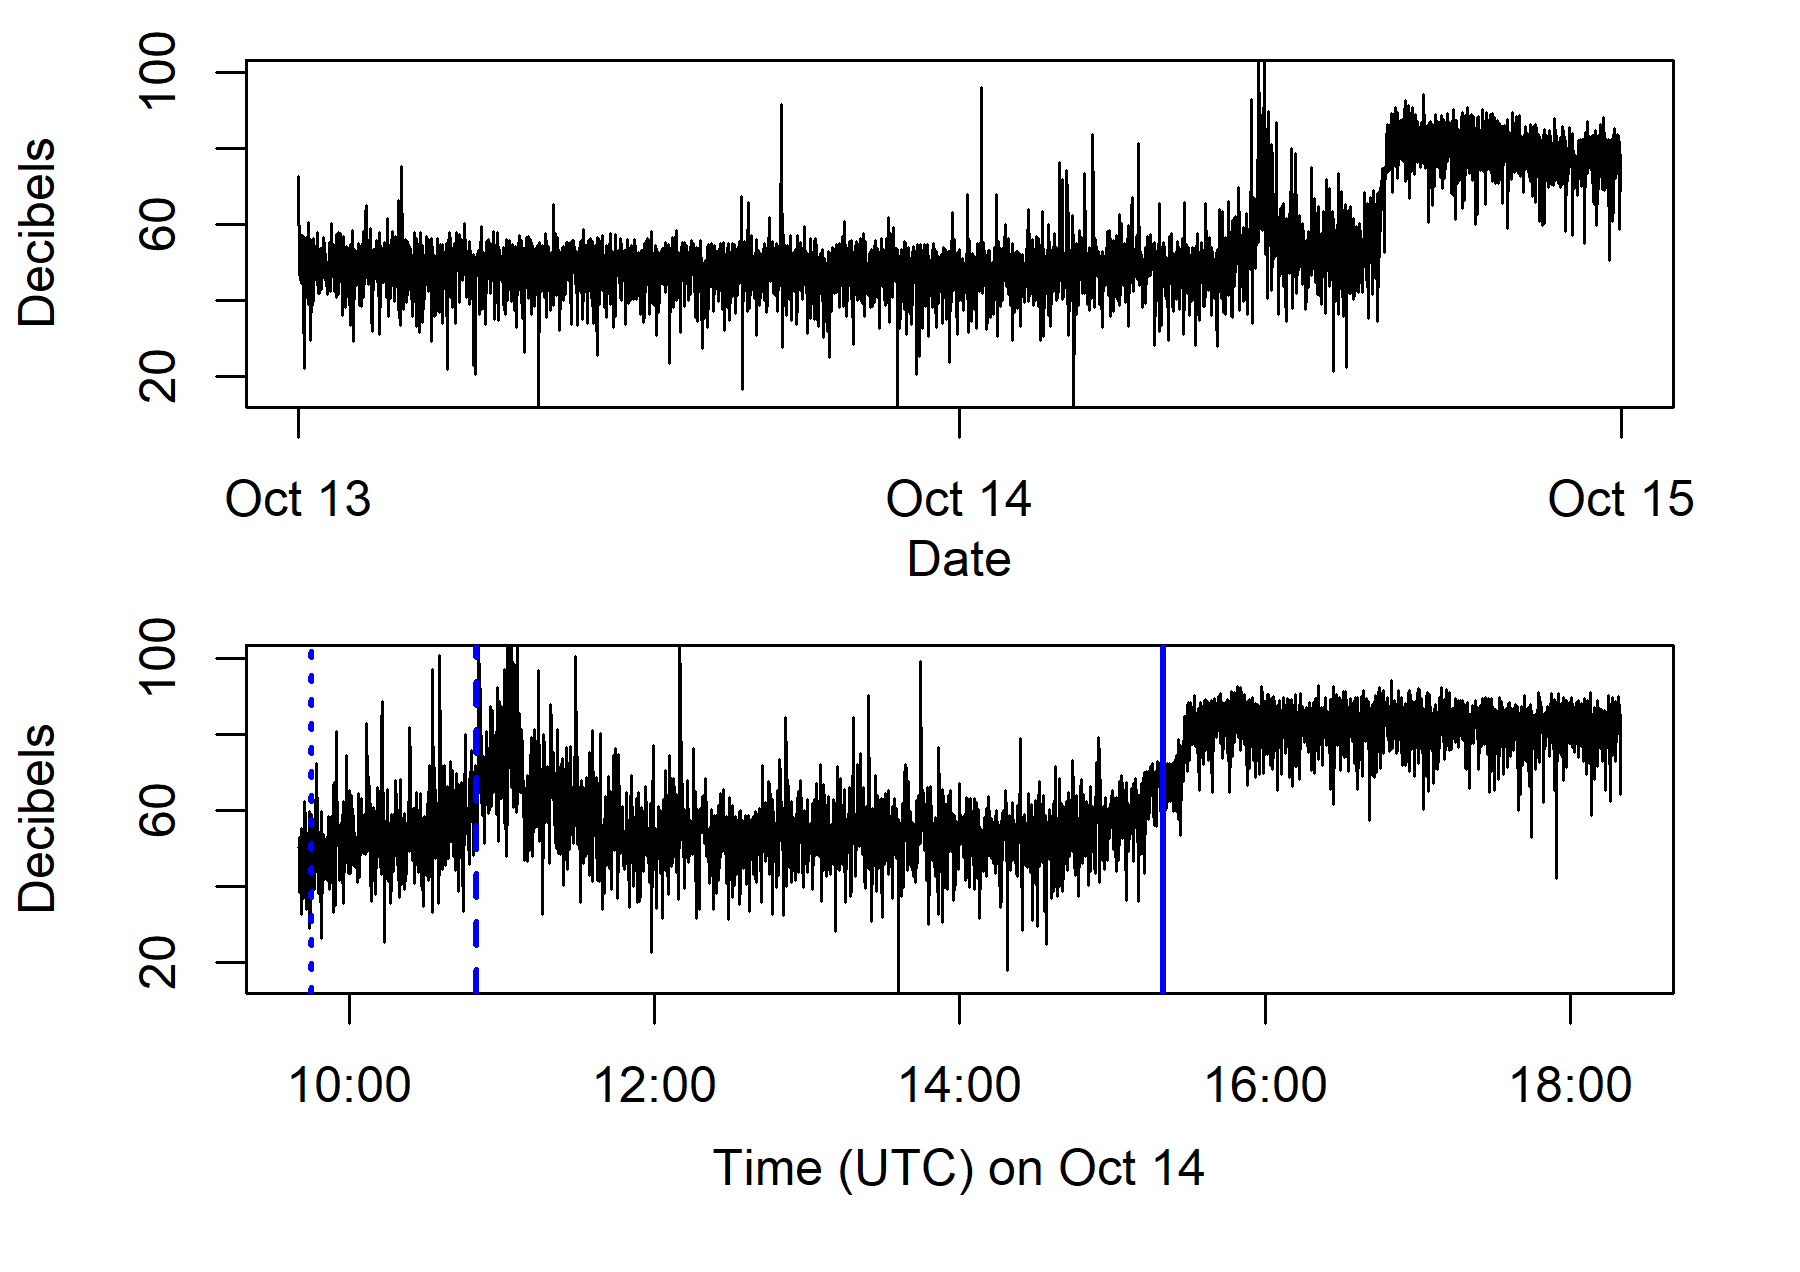}%
\label{fig:test_envelope}}

\caption{Test event: (a) Seismic signal for the 1-5Hz frequency band and (b) the corresponding envelope index in decibels (dB) for the October 2010 eruption event. The dotted, dashed and bold blue vertical lines denote the start of the seismic crisis, the start and end of the seismic swarm and the eruption onset respectively. Note that the time series are deciminated such as every 3456th reading and every 306th reading are shown for the top and bottom plots respectively.}
\label{fig_test}
\end{figure*}

\begin{figure*}[!t]
\centering
\subfloat[Signal]{\includegraphics[width=3.5in,valign=t, trim = {0.8cm 0 0cm 0}]{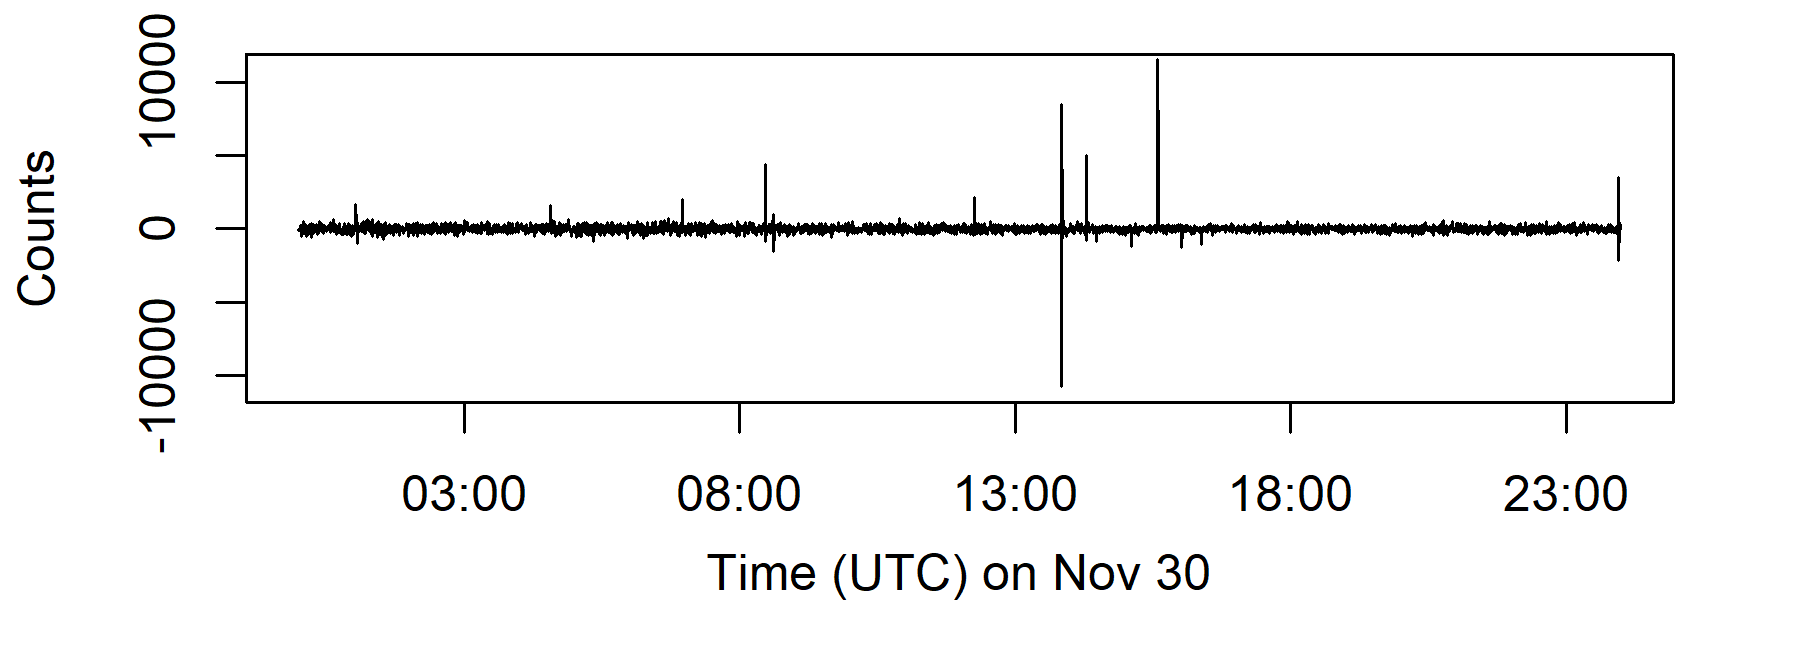}%
\label{fig:nonevent1_signal}}
\hfil
\subfloat[Envelope index]{\includegraphics[width=3.5in,valign=t, trim = {0cm 0 0.8cm 0}]{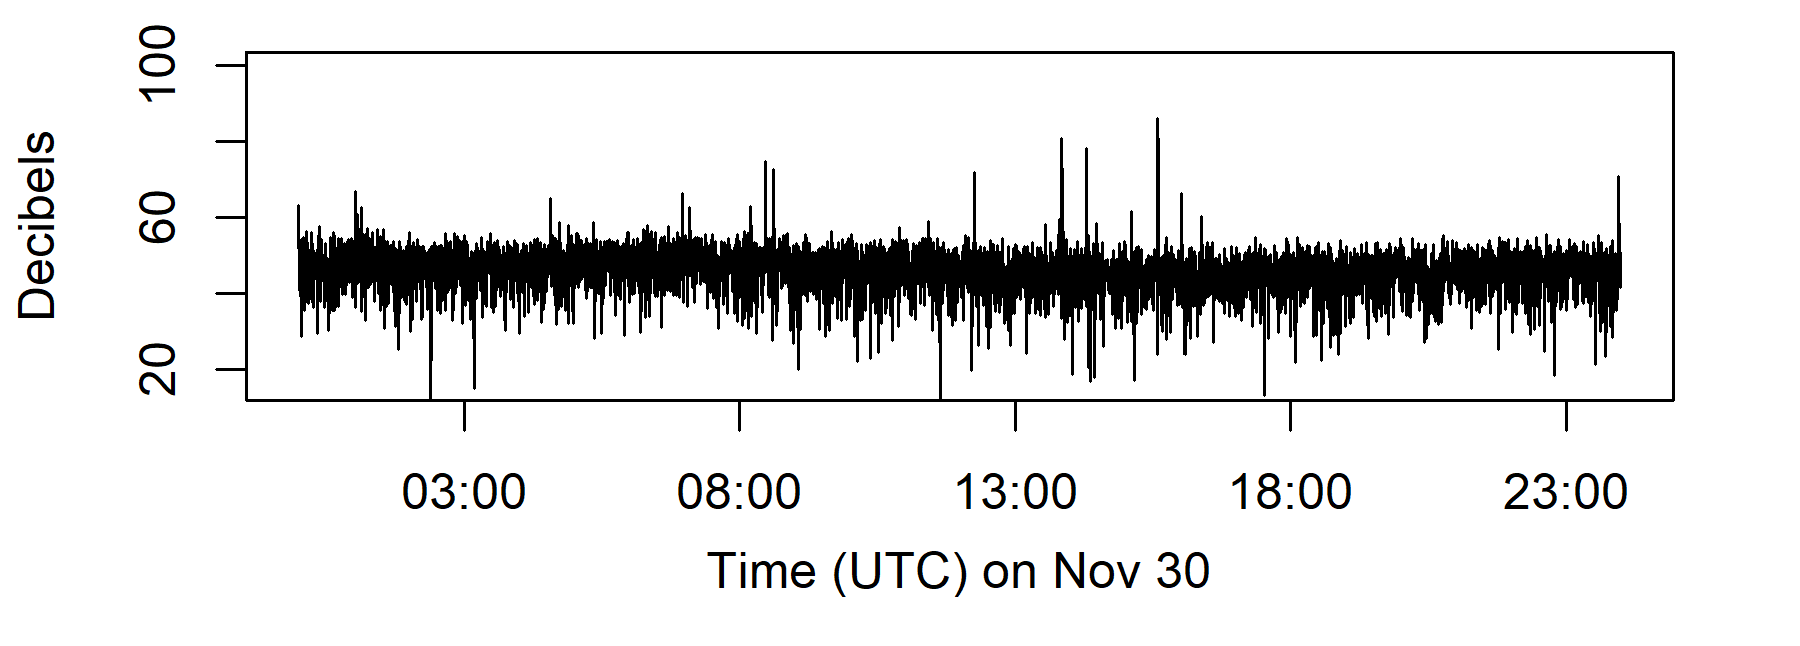}%
\label{fig:nonevent1_envelope}}

\caption{Test non-event 1: (a) Seismic signal for the 1-5Hz frequency band and (b) the corresponding envelope index in decibels (dB) for November 30 2009. Note that the time series are deciminated such as every 1728th reading are shown.}
\label{fig_nonevent1}
\end{figure*}

\begin{figure*}[!t]
\centering
\subfloat[Signal]{\includegraphics[width=3.5in,valign=t, trim = {0.8cm 0 0cm 0}]{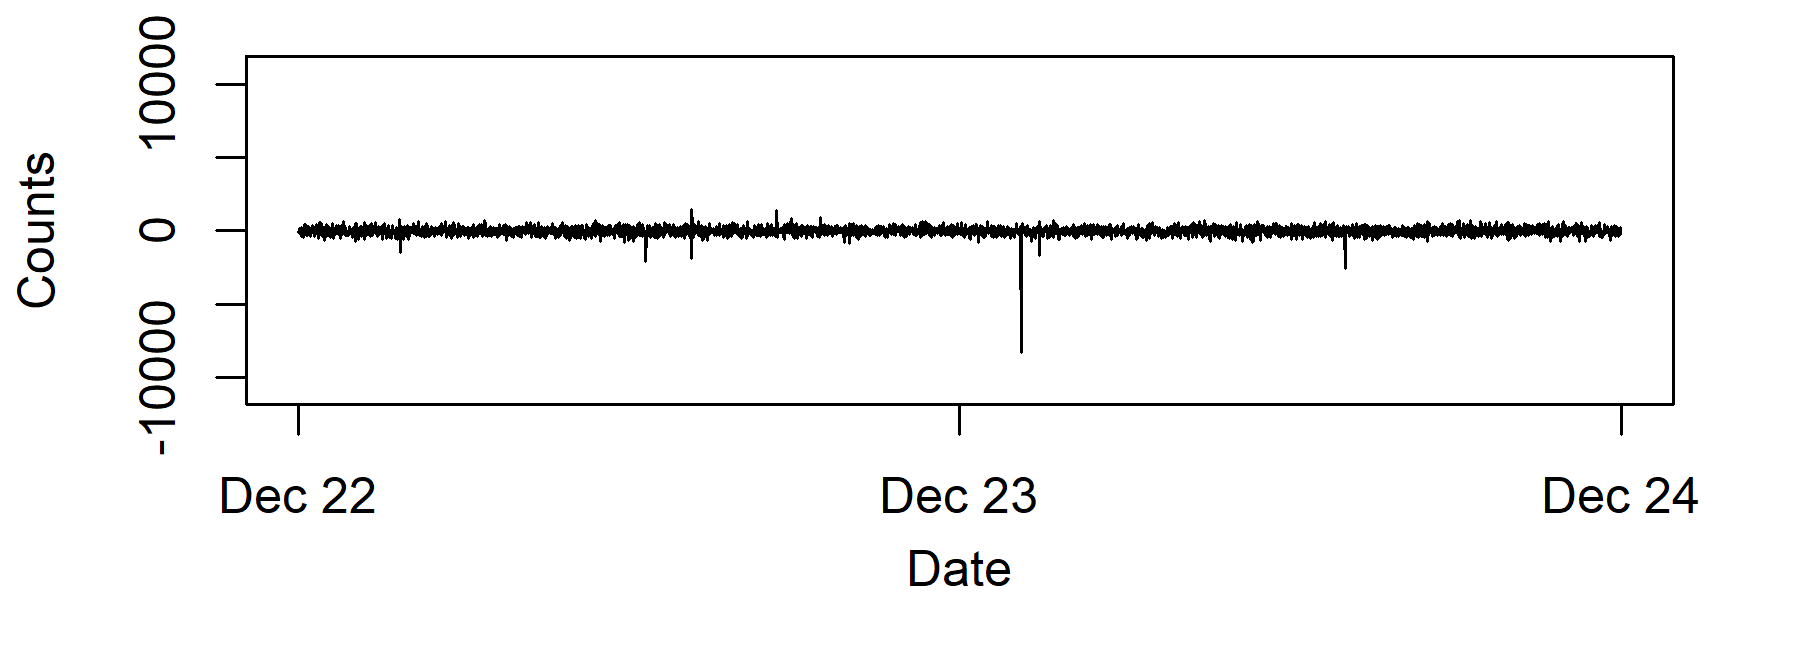}%
\label{fig:nonevent2_signal}}
\hfil
\subfloat[Envelope index]{\includegraphics[width=3.5in,valign=t, trim = {0cm 0 0.8cm 0}]{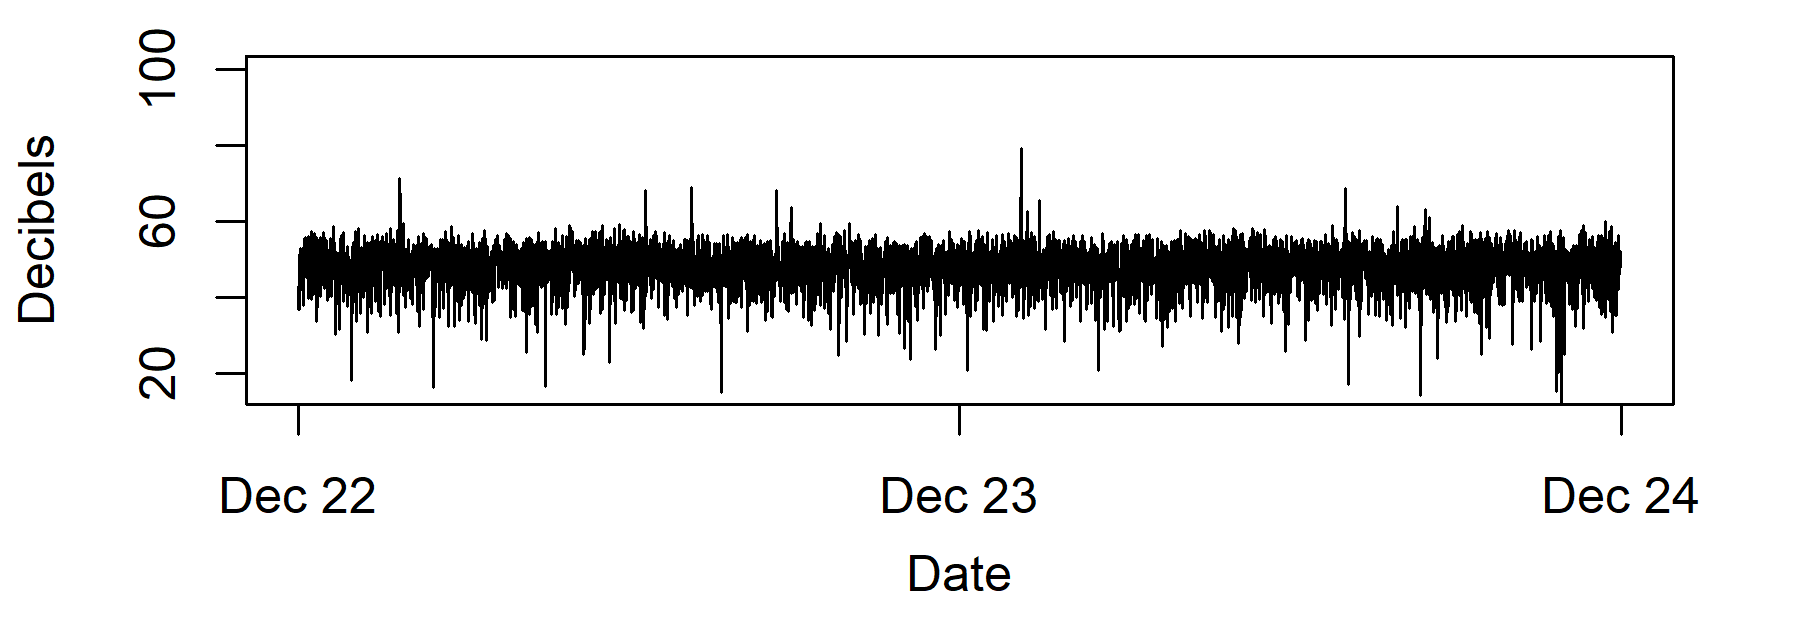}%
\label{fig:nonevent2_envelope}}

\caption{Test non-event 2: (a) Seismic signal for the 1-5Hz frequency band and (b) the corresponding envelope index in decibels (dB) for December 22-23 2009. Note that the time series are deciminated such as every 3456th reading are shown.}
\label{fig_nonevent2}
\end{figure*}

\begin{figure*}[!t]
\centering
\subfloat[Signal]{\includegraphics[width=3.5in,valign=t, trim = {0.8cm 0 0cm 0}]{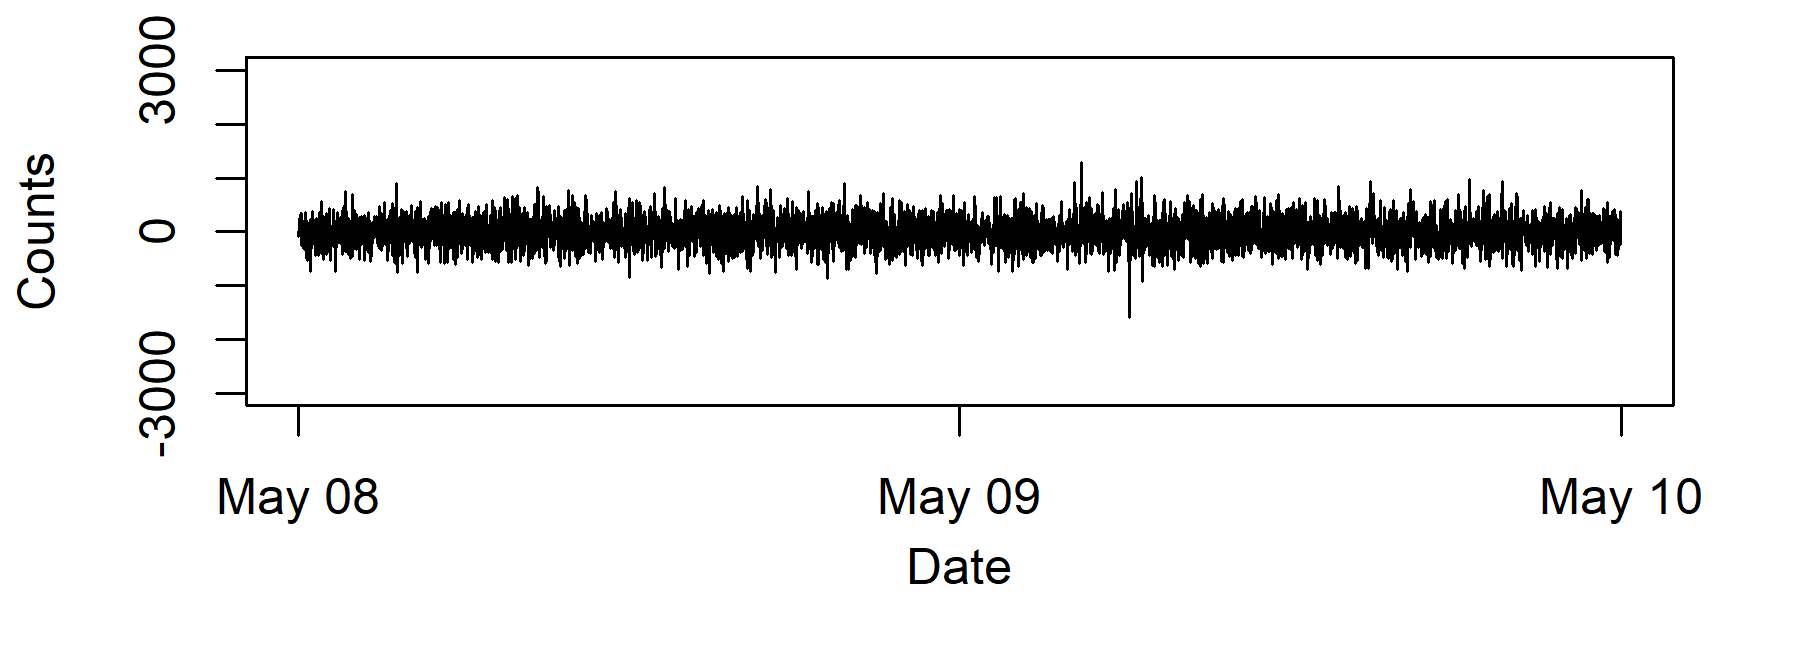}%
\label{fig:nonevent3_signal}}
\hfil
\subfloat[Envelope index]{\includegraphics[width=3.5in,valign=t, trim = {0cm 0 0.8cm 0}]{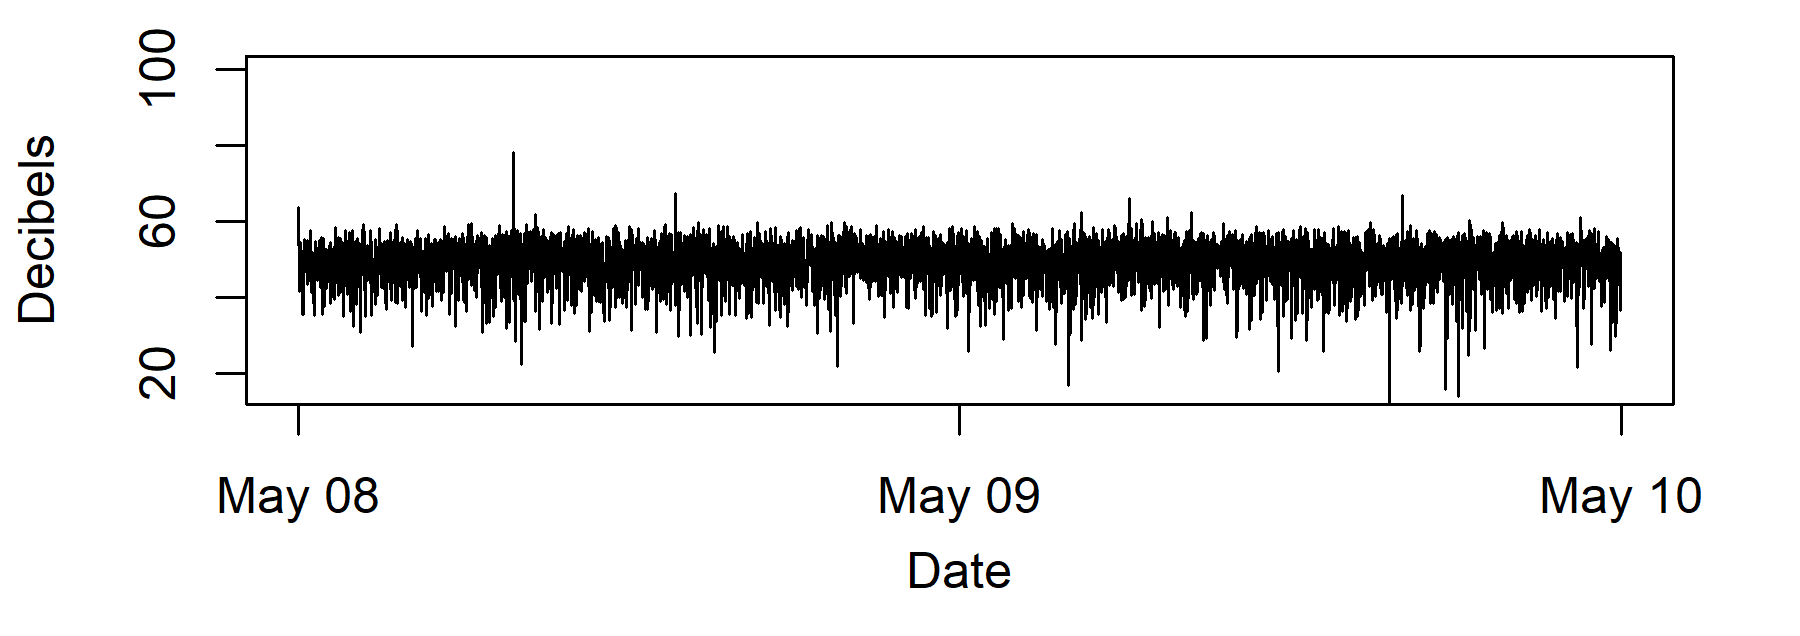}%
\label{fig:nonevent3_envelope}}

\caption{Test non-event 3: (a) Seismic signal for the 1-5Hz frequency band and (b) the corresponding envelope index in decibels (dB) for May 7-8 2010. Note that the time series are deciminated such as every 3456th reading are shown.}
\label{fig_nonevent3}
\end{figure*}

\section{Threshold selection with multiple training events}

There are a few ways we could determine a suitable threshold based on data from multiple events. An initial approach might be to simply combine the data across events and use all exceedances to inform the threshold. Figure \ref{fig_gpd_all} shows that this leads to a relatively high threshold of 95 being selected. In addition, since there were comparatively more exceedances from Event 2 than Events 1 and 3 (260 exceedances versus 14 and 3 exceedances for Events 1 and 3), the model fitted the data from Event 2 better than Events 1 and 3. This is reflected in much higher forecast probabilities near the eruption period for Event 2 than for Events 1 and 3 as seen in Figure \ref{fig_te_prob}.
\\
An alternative approach for choosing a suitable threshold across all training events, which we eventually use, would be to estimate thresholds for the training events separately and use the lowest estimate across events. This will ensure that we have sufficient exceedances to represent each event. 
\\
Figure \ref{fig_gpd_12} shows the p-values for the GPD goodness-of-fit tests for Events 1 and 2 for the 1-5Hz envelope index. The corresponding plot for Event 3 is shown in Figure 1d of the main paper. From these plots, the threshold estimates from Event 1, 2 and 3 are 89, 96 and 85 respectively. We see that the previous estimate of 95 which was obtained by combining the data across events was largely due to Event 2.   With the threshold choice of 85, the lowest estimate among the events, we have 282 exceedances for Training Event 1, 1033 for Event 2 and 423 for Event 3. As shown in Section V of the main paper, one-hour ahead forecast probabilities of sensible magnitudes were obtained for all three training events, the test event and the three non-events.

\begin{figure*}[!t]
\centering
\includegraphics[width=3.5in,valign=t]{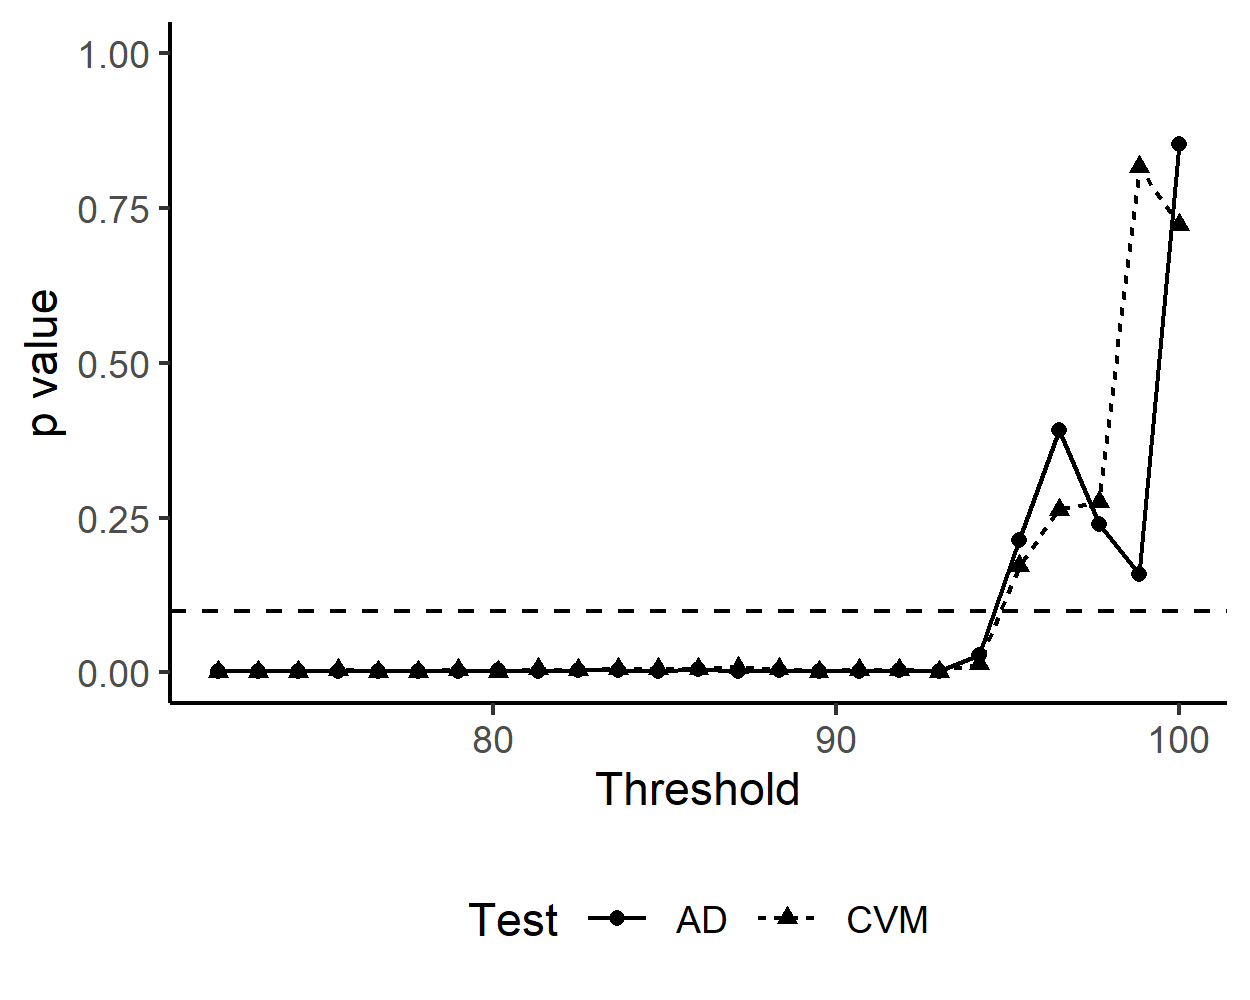}
\caption{Using data from all three Training events: p-values from the GPD goodness-of-fit tests (we select the lowest threshold for which the p-value exceeds the 10\% significance level).}
\label{fig_gpd_all}
\end{figure*}

\begin{figure*}[!t]
\centering
\subfloat[Training event 1]{\includegraphics[width=3.5in,valign=t]{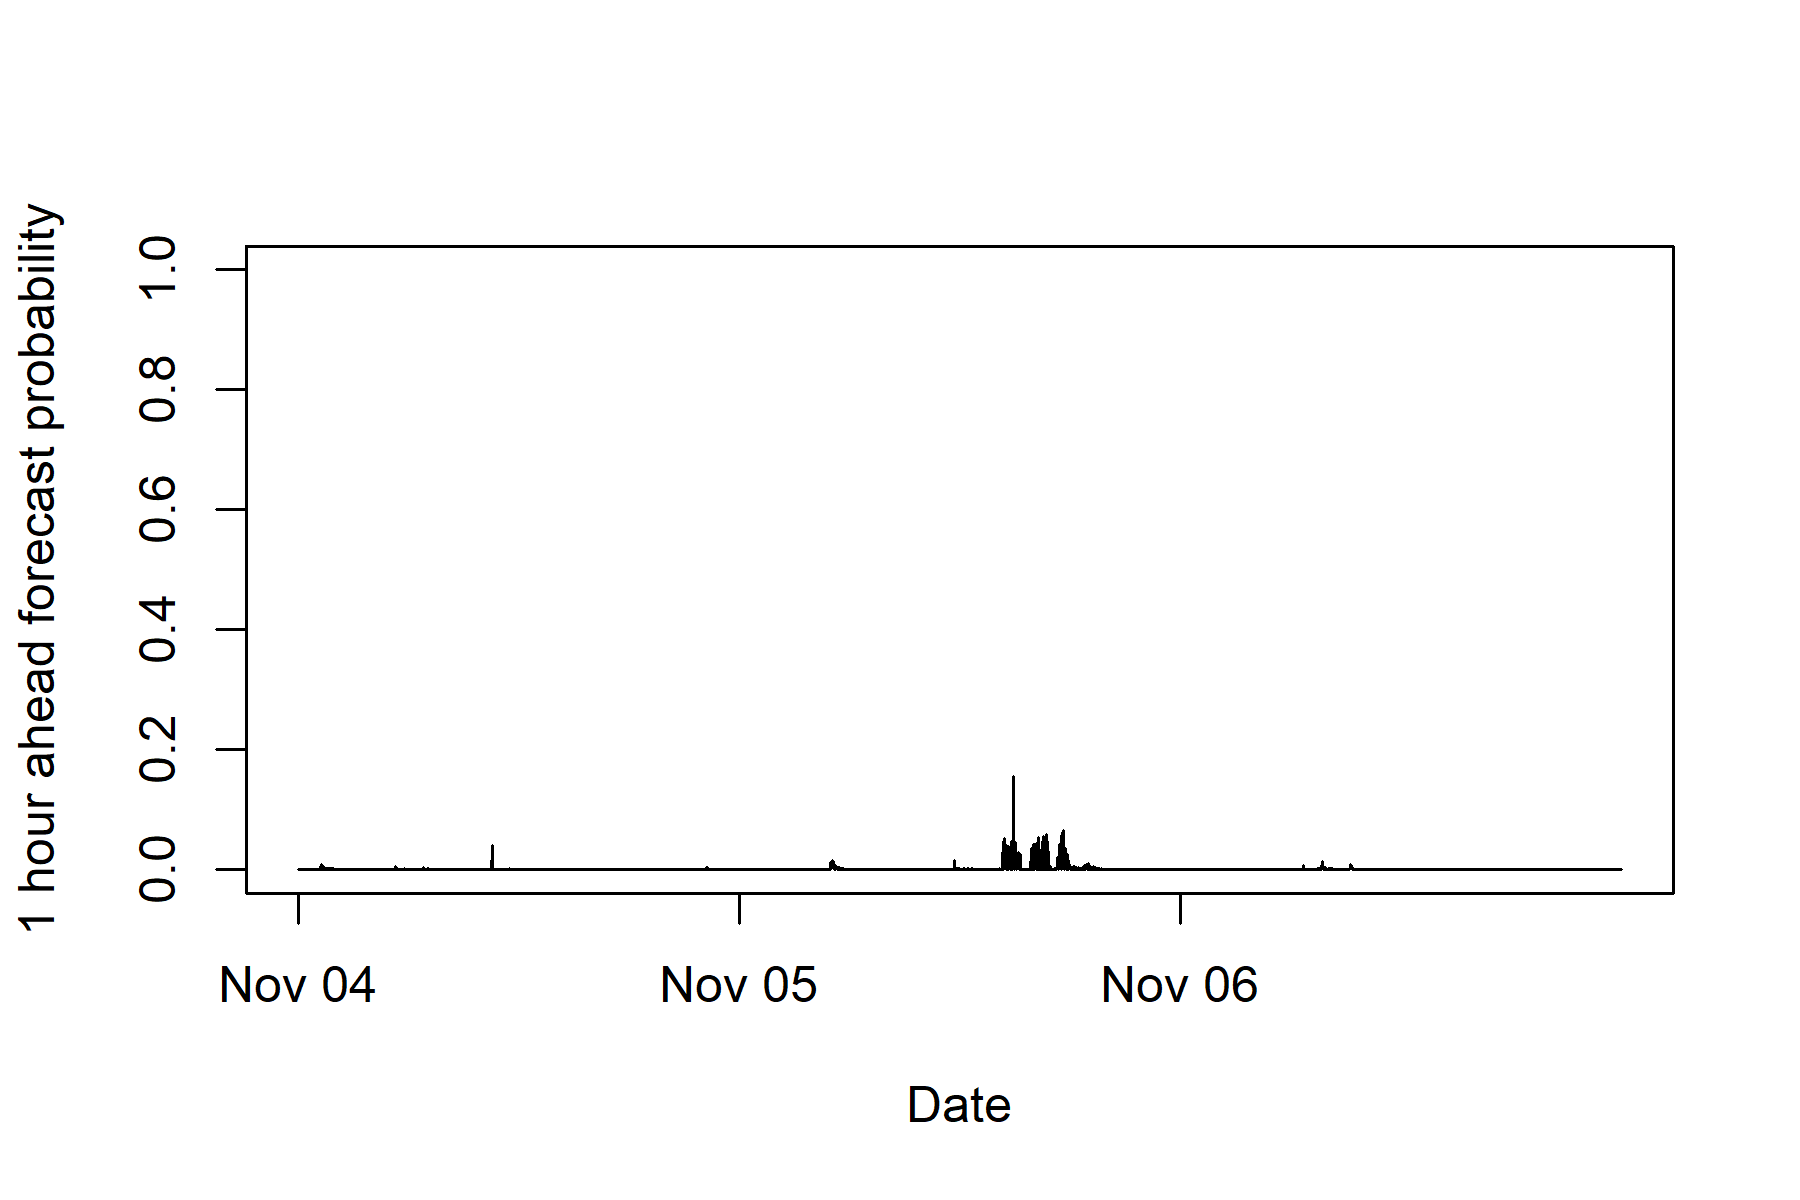}
\label{fig_te_prob_1}}
\subfloat[Training event 2]{\includegraphics[width=3.5in,valign=t]{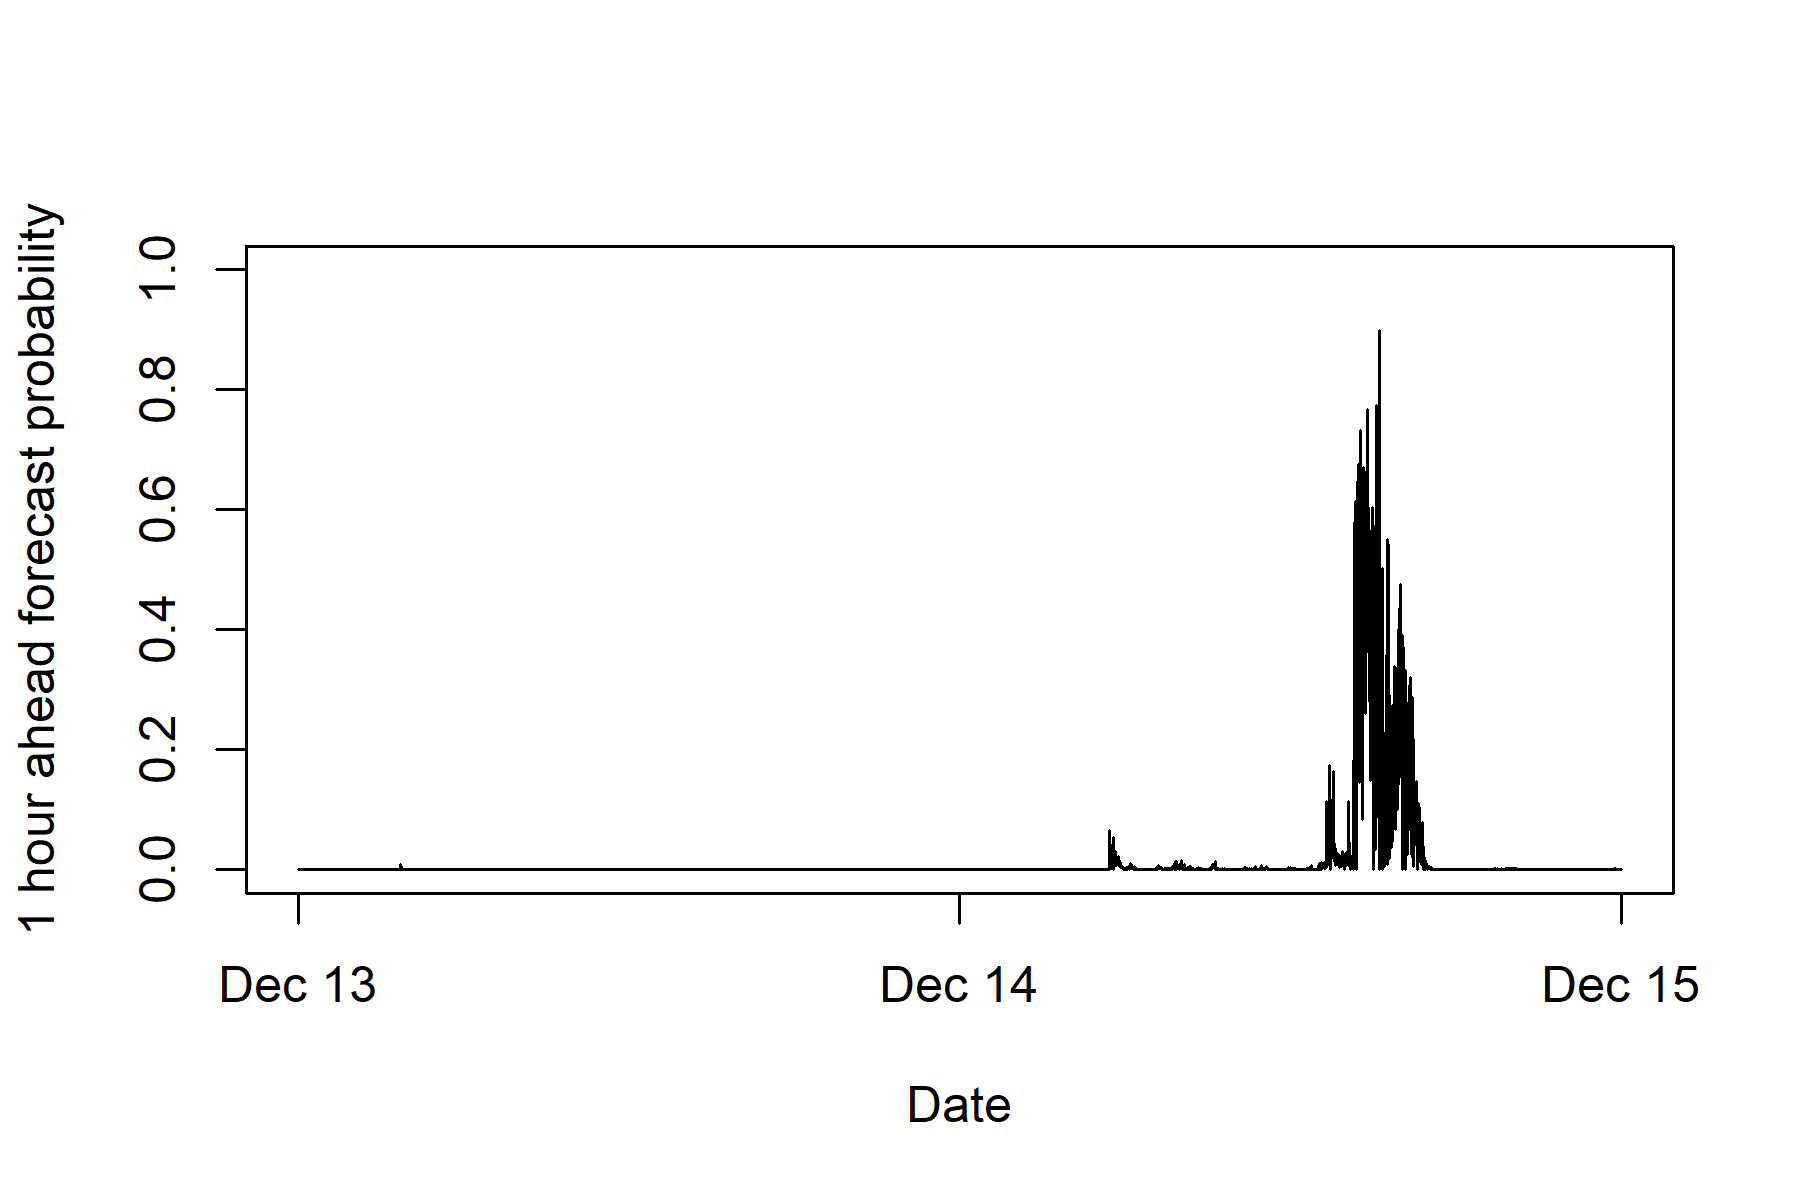}
\label{fig_te_prob_2}}
\\
\subfloat[Training event 3]{\includegraphics[width=3.5in,valign=t]{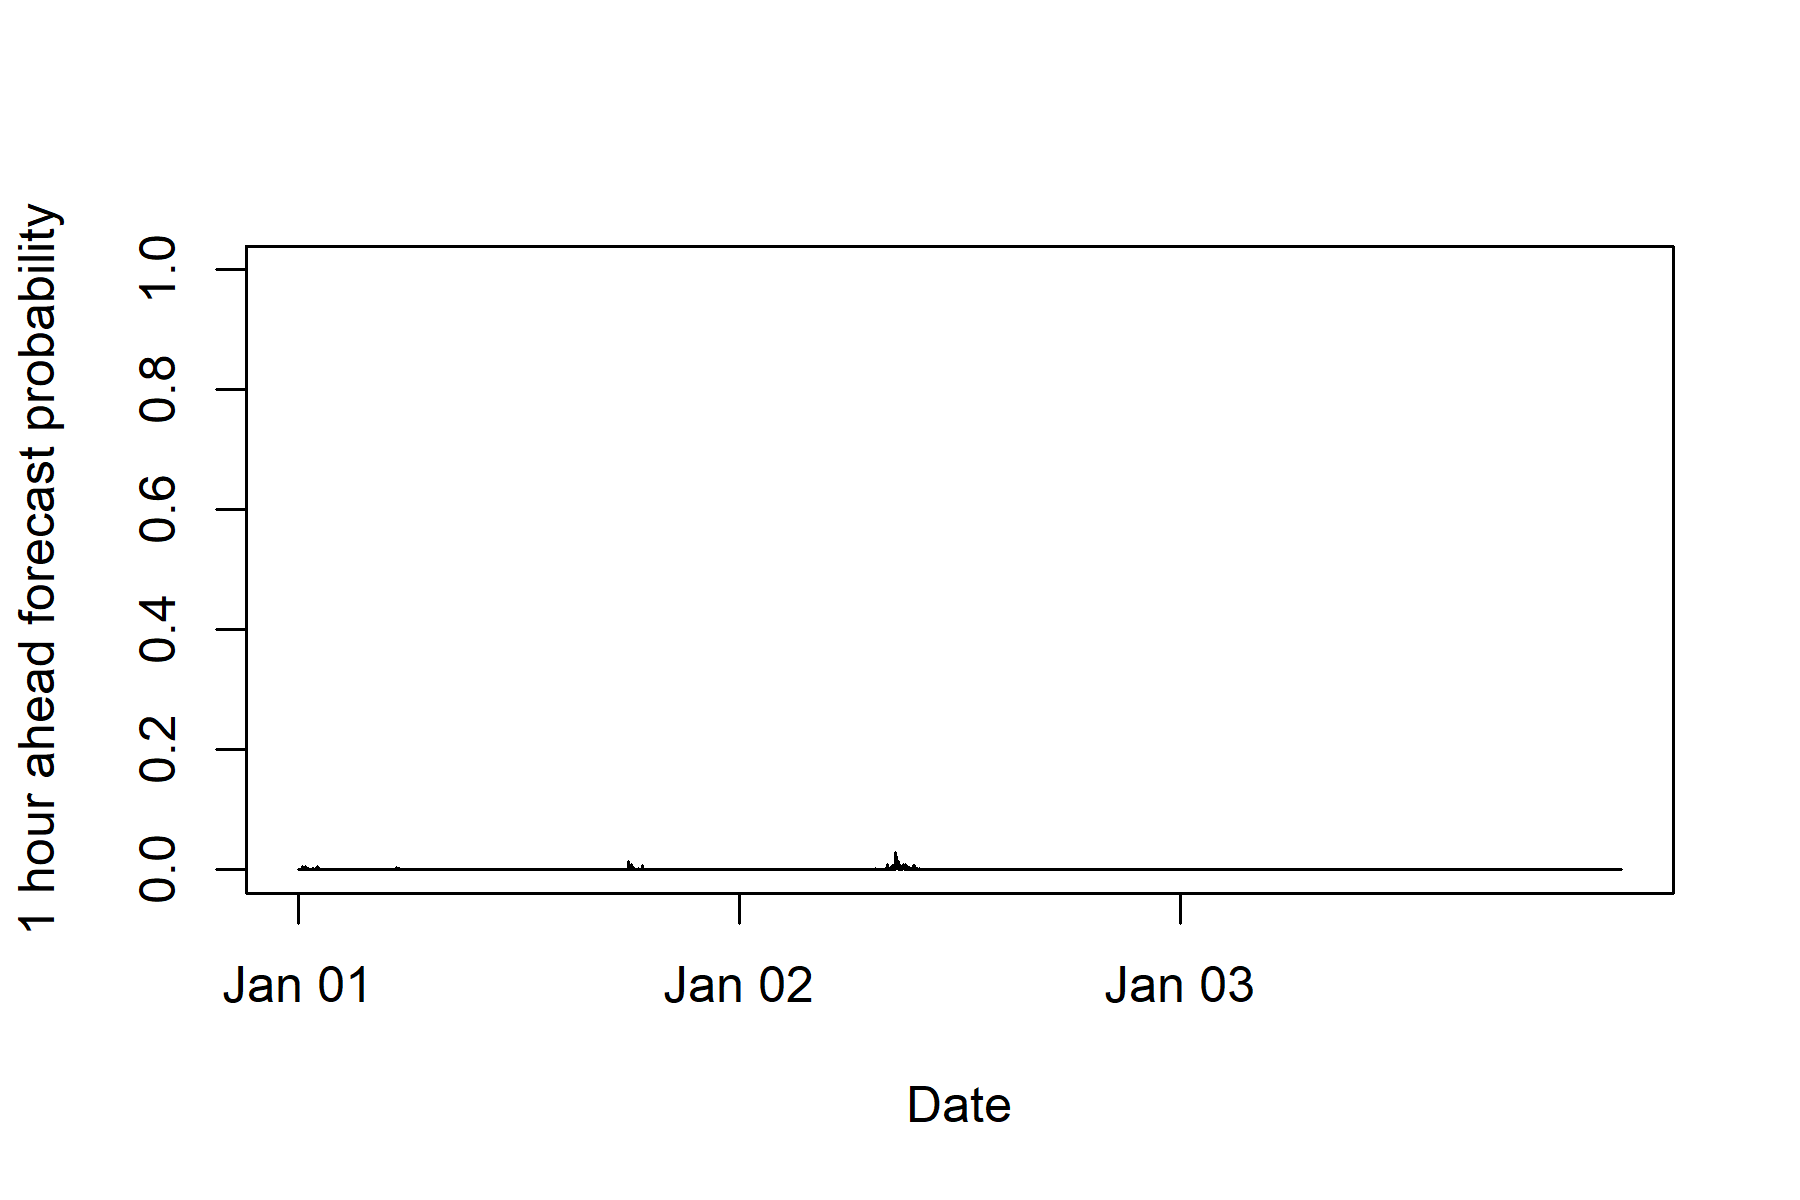}
\label{fig_te_prob_3}}

\caption{One-hour ahead threshold exceedance forecasts for the three training events using a threshold informed by data across events. Compared to Training event 2, the model is less able to distinguish and hence forecast eruptive activity for the other two training events because they contribute very few exceedances to inform the fit.}
\label{fig_te_prob}
\end{figure*}

\begin{figure*}[!t]
\centering
\subfloat[Training event 1]{\includegraphics[width=3.5in,valign=t]{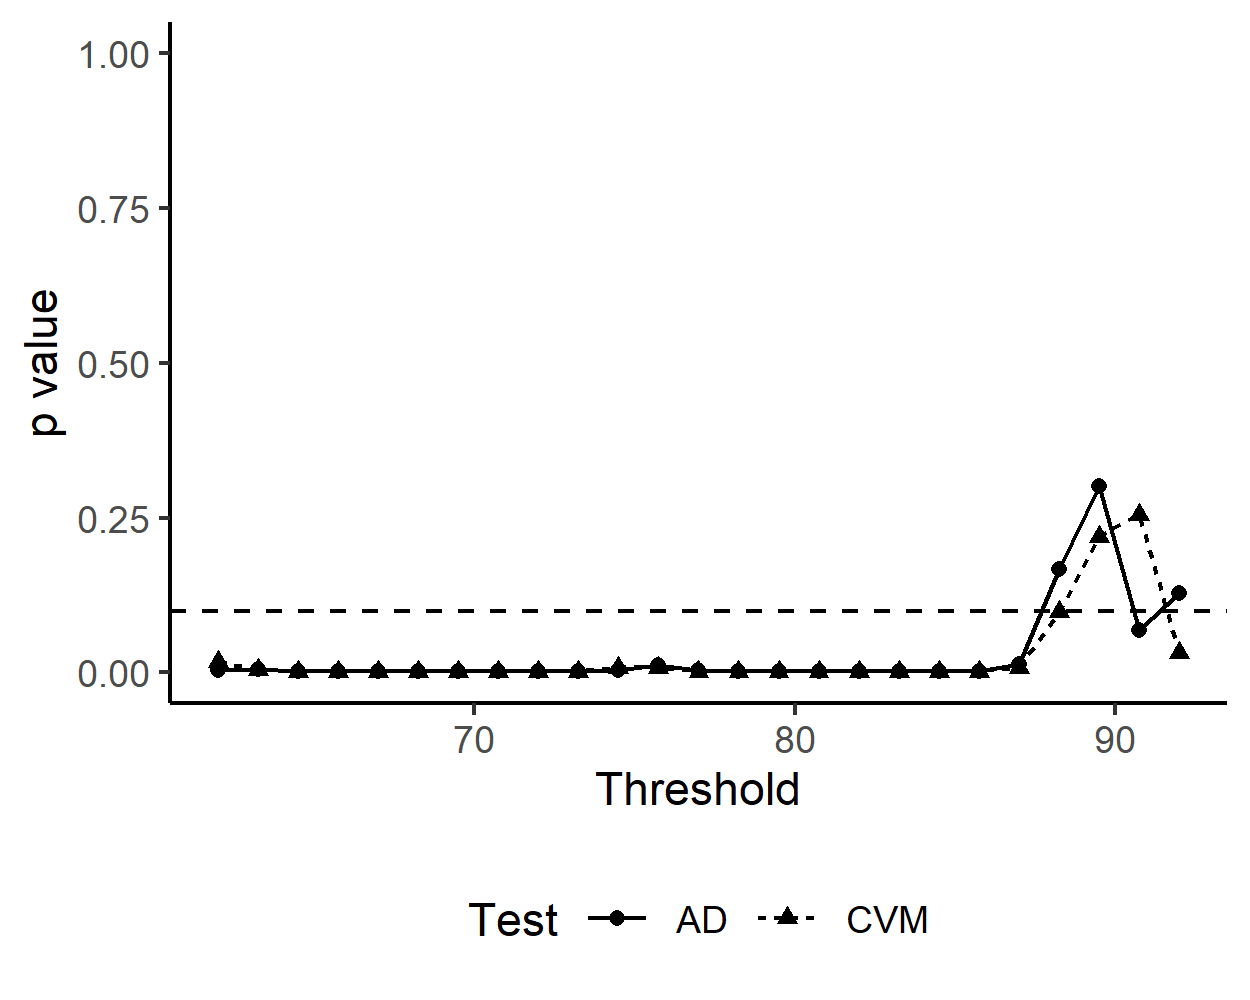}
\label{fig_gpd_pval_1}}
\subfloat[Training event 2]{\includegraphics[width=3.5in,valign=t]{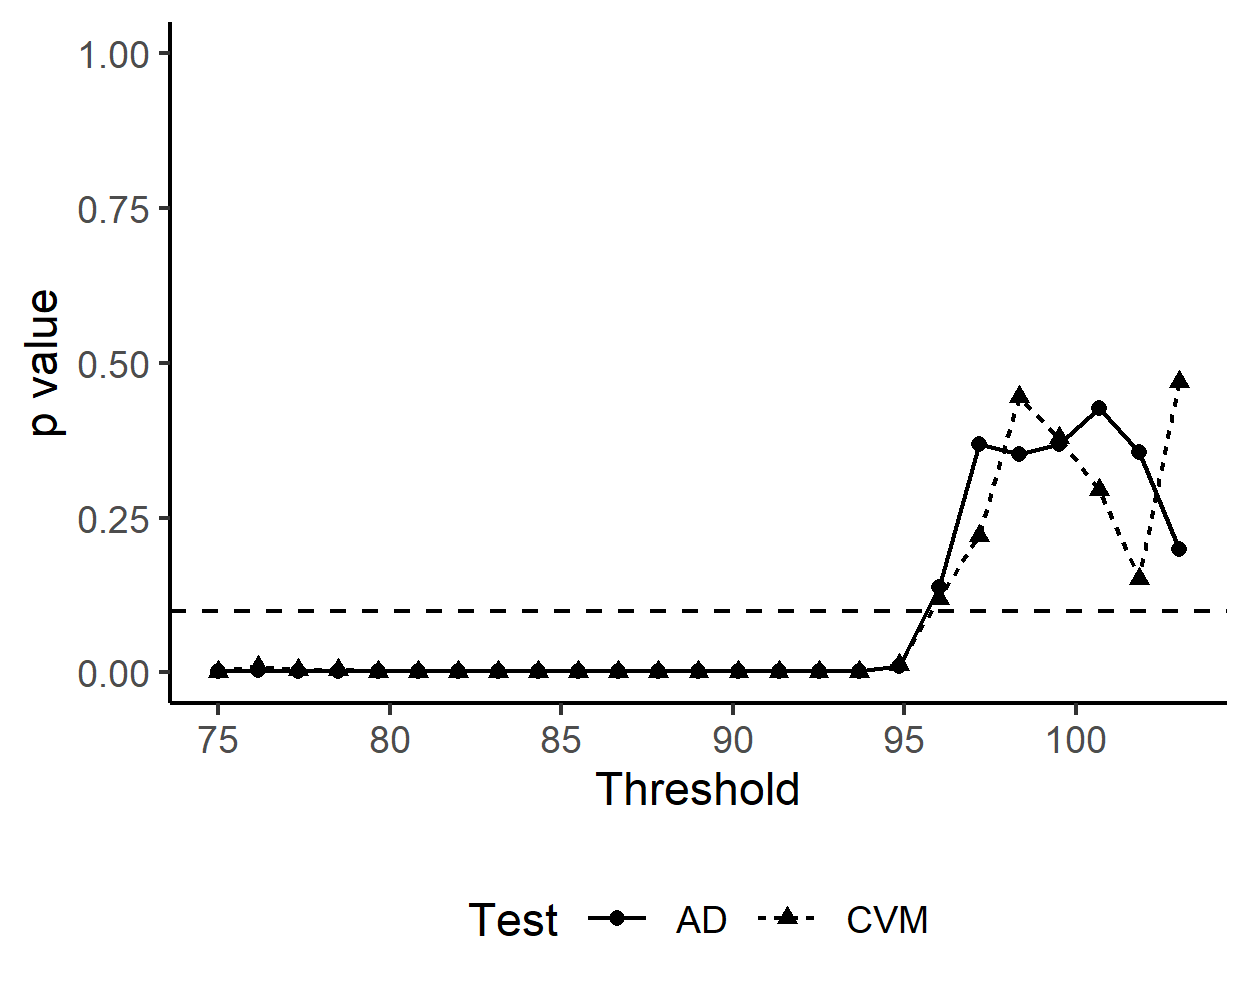}
\label{fig_gpd_pval_2}}

\caption{Using data from (a) Training event 1 and (b) Training event 2 separately: p-values from the GPD goodness-of-fit tests (we select the lowest threshold for which the p-value exceeds the 10\% significance level).}
\label{fig_gpd_12}
\end{figure*}

\section{Summary tables for the fitted logistic and GPD regression}

Tables \ref{tab:logistic} and \ref{tab:GPDreg} show the chosen covariates and parameter estimates for the threshold exceedance and excess models of the 1-5Hz envelope index. These were fitted using the three training event sets with the threshold being the lowest estimate among the three events.   

% latex table generated in R 3.6.1 by xtable 1.8-4 package
% Wed Feb 09 14:16:32 2022
\begin{table*}[!t]
\centering
\begin{tabular}{rrrrrrr}
  \hline
  Covariate $x$ & Transformation & & Estimate & Std. Error & z value & Pr($>$$|$z$|$) \\ 
  \hline
& & (Intercept) & -7.3880 & 0.1439 & -51.35 & 0.0000 \\ 
0.1-1Hz skewness & $x^2$ & skew\_011 & -0.1691 & 0.0441 & -3.84 & 0.0001 \\ 
0.1-1Hz maximum & $x^{-0.5}$ & max\_011 & 0.8403 & 0.1304 & 6.45 & 0.0000 \\ 
0.1-1Hz frequency mean kurtosis & $\log(x)$ & freq\_mean\_kurtosis\_011 & 0.6168 & 0.0829 & 7.44 & 0.0000 \\ 
0.1-1Hz frequency ROA & $\log(x)$ & freq\_roa\_011 & -0.9633 & 0.1020 & -9.45 & 0.0000 \\ 
0.1-1Hz frequency minimum & $\log(x)$ & freq\_min\_011 & -0.1473 & 0.0900 & -1.64 & 0.1017 \\ 
0.1-1Hz cepstral mean & $x^{0.5}$ & cep\_mean\_011 & -0.1463 & 0.0521 & -2.81 & 0.0049 \\ 
0.1-1Hz cepstral RMS bandwidth & $x^{0.5}$ & cep\_rms\_bw\_011 & -0.2902 & 0.0831 & -3.49 & 0.0005 \\ 
1-5Hz skewness & $x^{2}$ & skew\_15 & 0.4427 & 0.0564 & 7.85 & 0.0000 \\ 
1-5Hz cepstral kurtosis & $x^2$ & cep\_kurtosis\_15 & -0.2386 & 0.0650 & -3.67 & 0.0002 \\ 
1-5Hz cepstral ROA & $\log(x)$ & cep\_roa\_15 & -0.6387 & 0.0877 & -7.28 & 0.0000 \\ 
1-5Hz cepstral minimum & $x^{2}$ & cep\_min\_15 & 0.1153 & 0.0732 & 1.57 & 0.1153 \\ 
0.1-20Hz RMS bandwidth & $x^{2}$ & rms\_bw\_0120 & 0.0818 & 0.0499 & 1.64 & 0.1016 \\ 
0.1-20Hz cepstral skewness & $x^{2}$ & cep\_skew\_0120 & 3.9080 & 1.9356 & 2.02 & 0.0435 \\ 
0.1-20Hz cepstral kurtosis & $x^{2}$ & cep\_kurtosis\_0120 & -4.1807 & 1.9673 & -2.13 & 0.0336 \\ 
0.1-20Hz cepstral shannon entropy & $x^{2}$ & cep\_shannon\_0120 & -0.8076 & 0.1418 & -5.70 & 0.0000 \\ 
0.1-20Hz cepstral ratio of maximum over mean & $x^{-1}$ & cep\_ratio\_mom\_0120 & -0.1943 & 0.0854 & -2.27 & 0.0229 \\ 
5-15Hz ioCE & $x$ & ioce\_515 & -0.1323 & 0.0360 & -3.68 & 0.0002 \\ 
5-15Hz frequency ioCE & $\log(x)$ & freq\_ioce\_515 & -0.2535 & 0.1189 & -2.13 & 0.0330 \\ 
5-15Hz frequency mean kurtosis & $x^{-0.5}$ & freq\_mean\_kurtosis\_515 & -0.4388 & 0.0916 & -4.79 & 0.0000 \\ 
5-15Hz frequency shannon entropy & $x^{2}$ & freq\_shannon\_515 & 1.7404 & 0.1686 & 10.33 & 0.0000 \\ 
5-15Hz cepstral kurtotis & $x^{2}$ & cep\_kurtosis\_515 & 0.2686 & 0.0962 & 2.79 & 0.0053 \\ 
5-15Hz cepstral minimum & $x$ & cep\_min\_515 & -0.3022 & 0.0625 & -4.84 & 0.0000 \\ 
5-15Hz frequency ratio of maximum over mean & $\log(x)$ & freq\_ratio\_mom\_515 & -0.5775 & 0.1338 & -4.32 & 0.0000 \\ 
High pass 0.01Hz skewness & $x^{2}$ & skew\_hp001 & 0.1527 & 0.0517 & 2.95 & 0.0032 \\ 
High pass 0.01Hz energy & $\log(x)$ & energy\_hp001 & 3.3015 & 0.1915 & 17.24 & 0.0000 \\ 
High pass 0.01Hz minimum & $x^{2}$ & min\_hp001 & -0.2913 & 0.0571 & -5.10 & 0.0000 \\ 
High pass 0.01Hz frequency skewness & $x^{-0.5}$ & freq\_skew\_hp001 & -0.5542 & 0.0809 & -6.85 & 0.0000 \\ 
High pass 0.01Hz cepstral ratio of maximum over mean & $x^{-1.5}$ & cep\_ratio\_mom\_hp001 & -0.1076 & 0.0598 & -1.80 & 0.0717 \\ 
0.1-1Hz envelope mean & $x^{-2}$ & env\_mean\_011 & -0.6742 & 0.0959 & -7.03 & 0.0000 \\ 
0.1-1Hz envelope standard deviation & $x^{-2}$ & env\_sd\_011 & 0.1178 & 0.0612 & 1.93 & 0.0541 \\ 
0.1-1Hz envelope kurtosis & $x$ & env\_kurtosis\_011 & -0.1522 & 0.0463 & -3.28 & 0.0010 \\ 
0.1-1Hz envelope RMS bandwidth & $x^{2}$ & env\_rms\_bw\_011 & -0.1574 & 0.0219 & -7.20 & 0.0000 \\ 
0.1-1Hz envelope ROA & $\log(x)$ & env\_roa\_011 & -0.6990 & 0.0819 & -8.53 & 0.0000 \\ 
0.1-1Hz envelope minimum & $x^{1.5}$ & env\_min\_011 & -0.4781 & 0.0723 & -6.61 & 0.0000 \\ 
1-5Hz envelope kurtosis & $x^{-0.5}$ & env\_kurtosis\_15 & 0.6752 & 0.0614 & 10.99 & 0.0000 \\ 
1-5Hz envelope mean kurtosis & $x^{-2}$ & env\_mean\_kurtosis\_15 & 0.3609 & 0.0390 & 9.25 & 0.0000 \\ 
1-5Hz envelope ROA & $\log(x)$ & env\_roa\_15 & 0.5165 & 0.0576 & 8.97 & 0.0000 \\ 
0.1-20Hz envelope ROA & $x^{0.5}$ & env\_roa\_0120 & 0.5678 & 0.0657 & 8.65 & 0.0000 \\ 
5-15Hz envelope ROA & $x^{-1.5}$ & env\_roa\_515 & 0.1469 & 0.0450 & 3.27 & 0.0011 \\ 
   \hline \\
\end{tabular}
\caption{Table of parameter estimates for the logistic regression for the threshold exceedance of the 1-5Hz envelope index. Here, ROA refers to the rate of attack, RMS refers to root mean square and ioCE refers to i of Central Energy.}
\label{tab:logistic}
\end{table*}

% latex table generated in R 3.6.1 by xtable 1.8-4 package
% Wed Feb 09 14:52:38 2022
\begin{table*}[!t]
\centering
\begin{tabular}{rrrrrrr}
  \hline
  Covariate $x$ & Transformation & & Estimate & Std. Error & z value & Pr($>$$|$z$|$) \\ 
  \hline
& & (Intercept) & 1.74 & 0.07 & 24.00 & 0.00 \\ 
1-5Hz frequency kurtosis & $\log(x)$ &  freq\_kurtosis\_15 & -0.25 & 0.02 & -11.98 & 0.00 \\ 
1-5Hz frequency ioCE & $x^{0.5}$ & freq\_ioce\_15 & -0.48 & 0.07 & -7.13 & 0.00 \\ 
1-5Hz frequency RMS bandwidth & $x^{-1.5}$ &  freq\_rms\_bw\_15 & -0.18 & 0.03 & -6.83 & 0.00 \\ 
0.1-20Hz envelope ROA & $x^{0.5}$ & env\_roa\_0120 & -0.27 & 0.05 & -5.50 & 0.00 \\ 
5-15Hz cepstral ratio of maximum over mean & $x^{-1}$ & cep\_ratio\_mom\_515 & 0.09 & 0.04 & 2.42 & 0.01 \\ 
0.1-1Hz envelope shannon entropy & $x^{2}$ & env\_shannon\_011 & -0.02 & 0.01 & -2.49 & 0.01 \\ 
1-5Hz cepstral shannon entropy & $x$ & cep\_shannon\_15 & -0.07 & 0.04 & -1.82 & 0.03 \\ 
   \hline \\
\end{tabular}
\caption{Table of parameter estimates for the GPD regression for the threshold excesses of the 1-5Hz envelope index. Here, ROA refers to the rate of attack, RMS refers to root mean square and ioCE refers to i of Central Energy.}
\label{tab:GPDreg}
\end{table*}

\section{Major covariates in the fitted logistic regression}

\vspace{-1mm}

From Table \ref{tab:logistic}, we see that the three covariates with the highest absolute coefficient estimates in the logistic regression for the 1-5Hz envelope index are 0.1-20Hz cepstral kurtosis (cep\_kurtosis\_0120), 0.1-20Hz cepstral skewness (cep\_skew\_0120) and high pass 0.01Hz energy (energy\_hp001). Figures \ref{fig_train1_covar}-\ref{fig_test_covar} shows their corresponding time series for the training and test events.

\begin{figure*}[!t]
\centering
\subfloat[0.1-20Hz cepstral kurtosis]{\includegraphics[width=3.5in,valign=t]{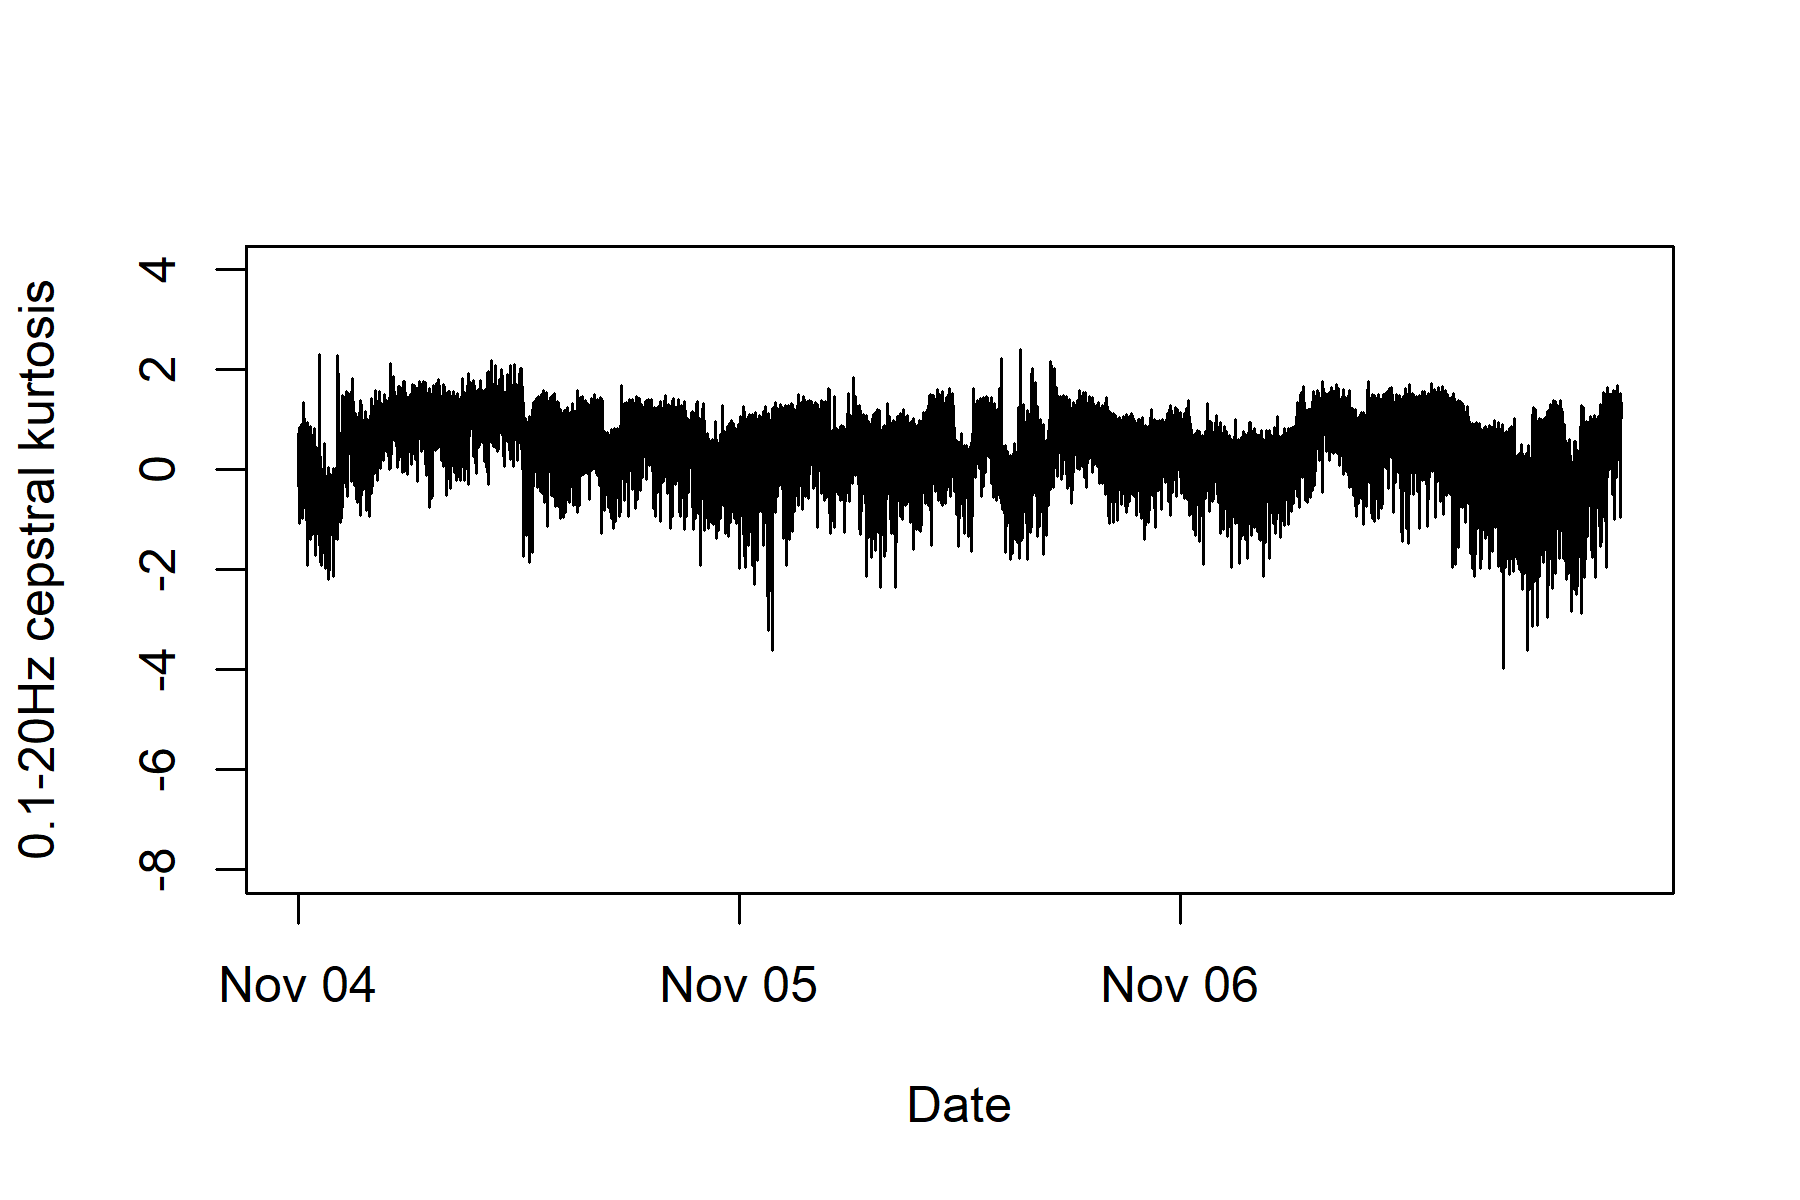}
}
\subfloat[Zoomed in]{\includegraphics[width=3.5in,valign=t]{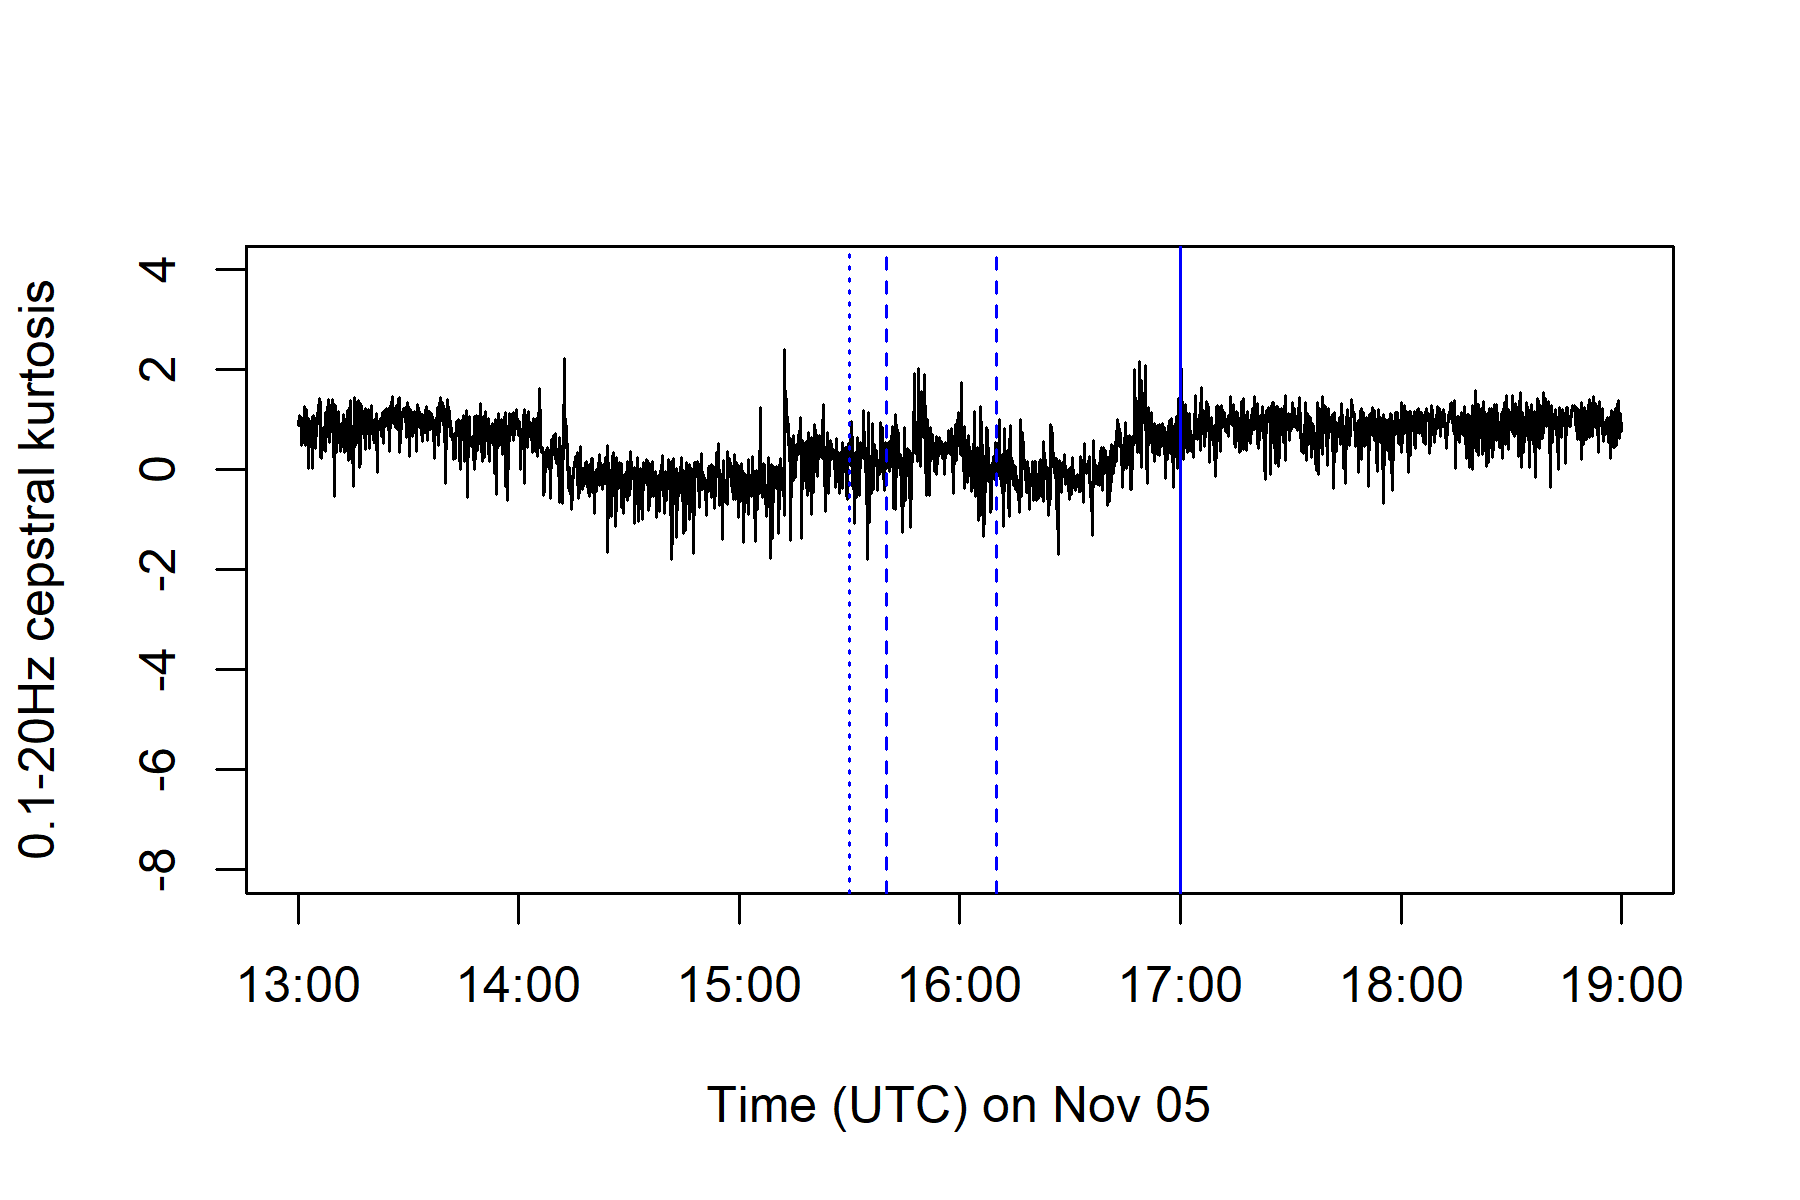}
}
\\
\subfloat[0.1-20Hz cepstral skewness]{\includegraphics[width=3.5in,valign=t]{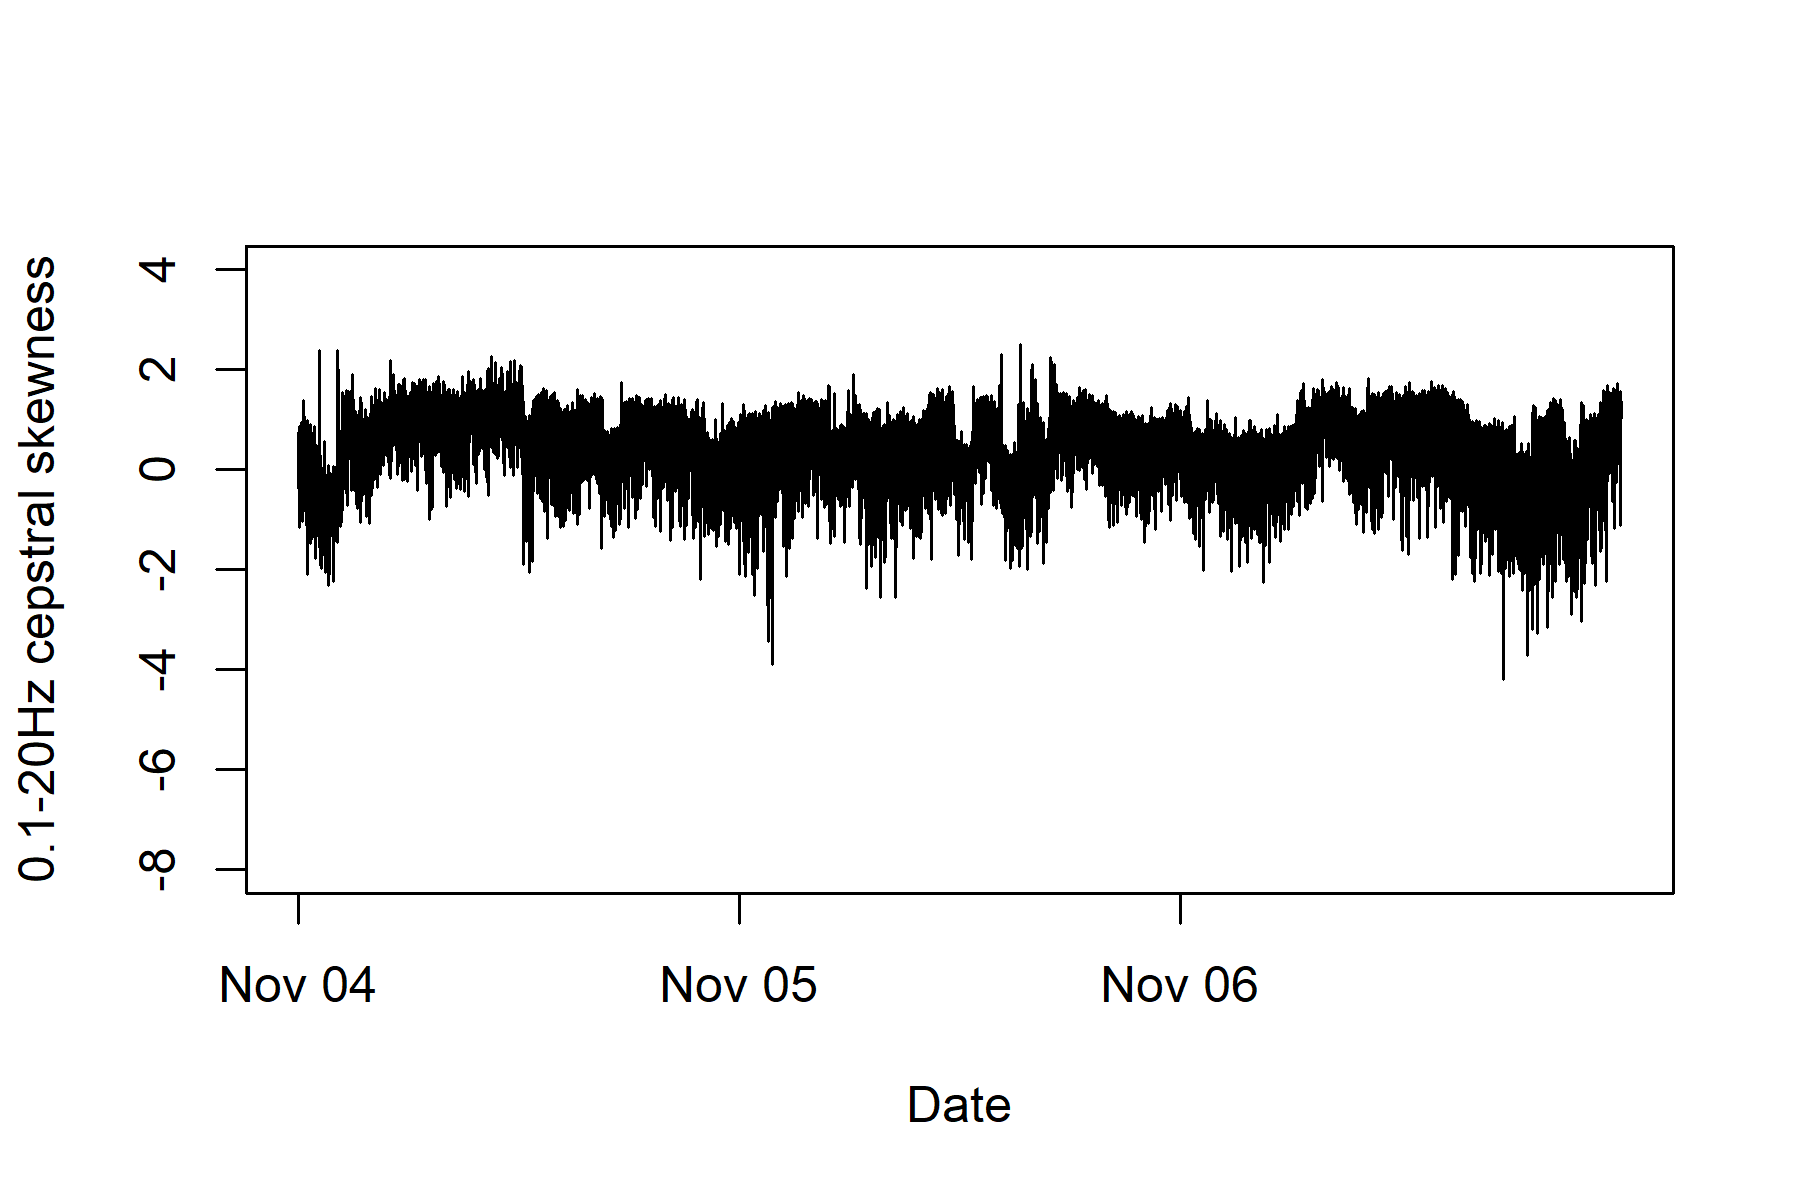}
}
\subfloat[Zoomed in]{\includegraphics[width=3.5in,valign=t]{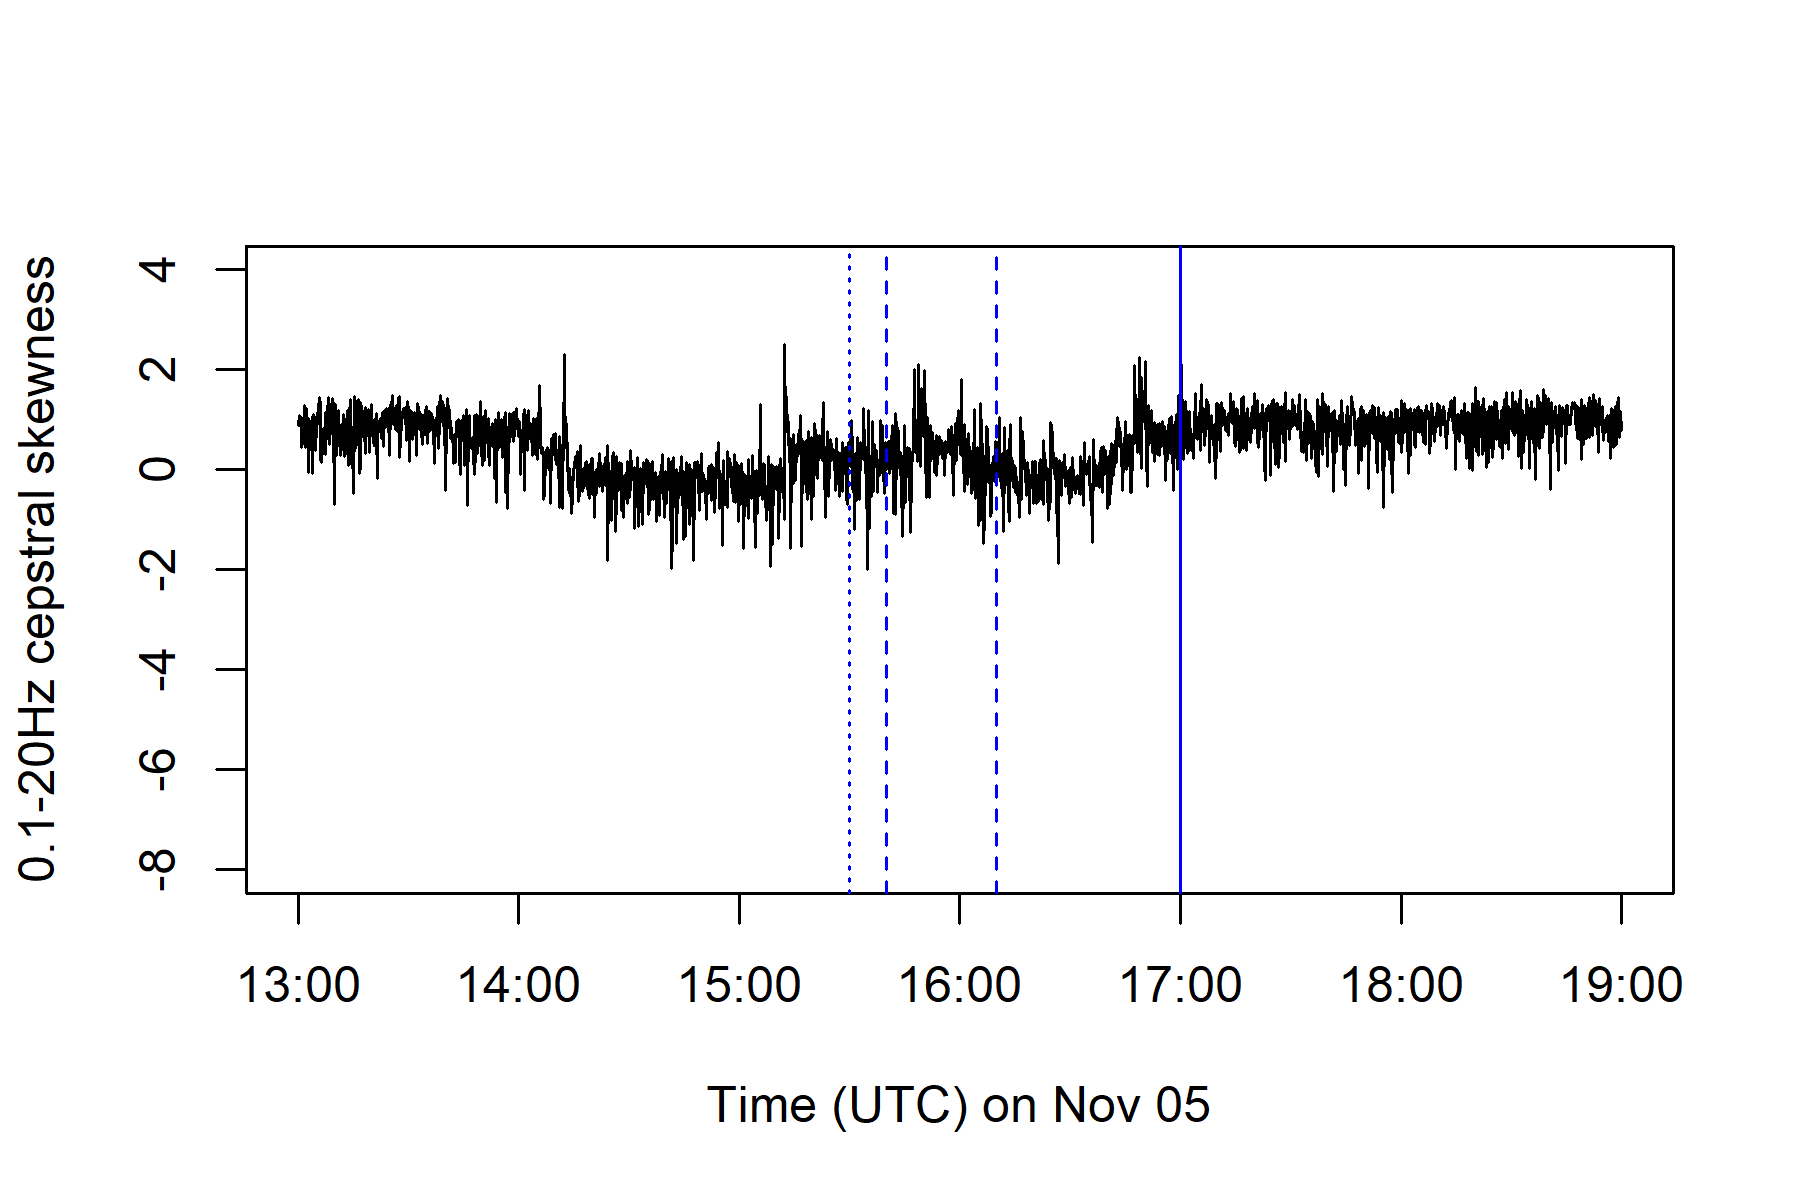}
}
\\
\subfloat[High pass 0.01Hz energy]{\includegraphics[width=3.5in,valign=t]{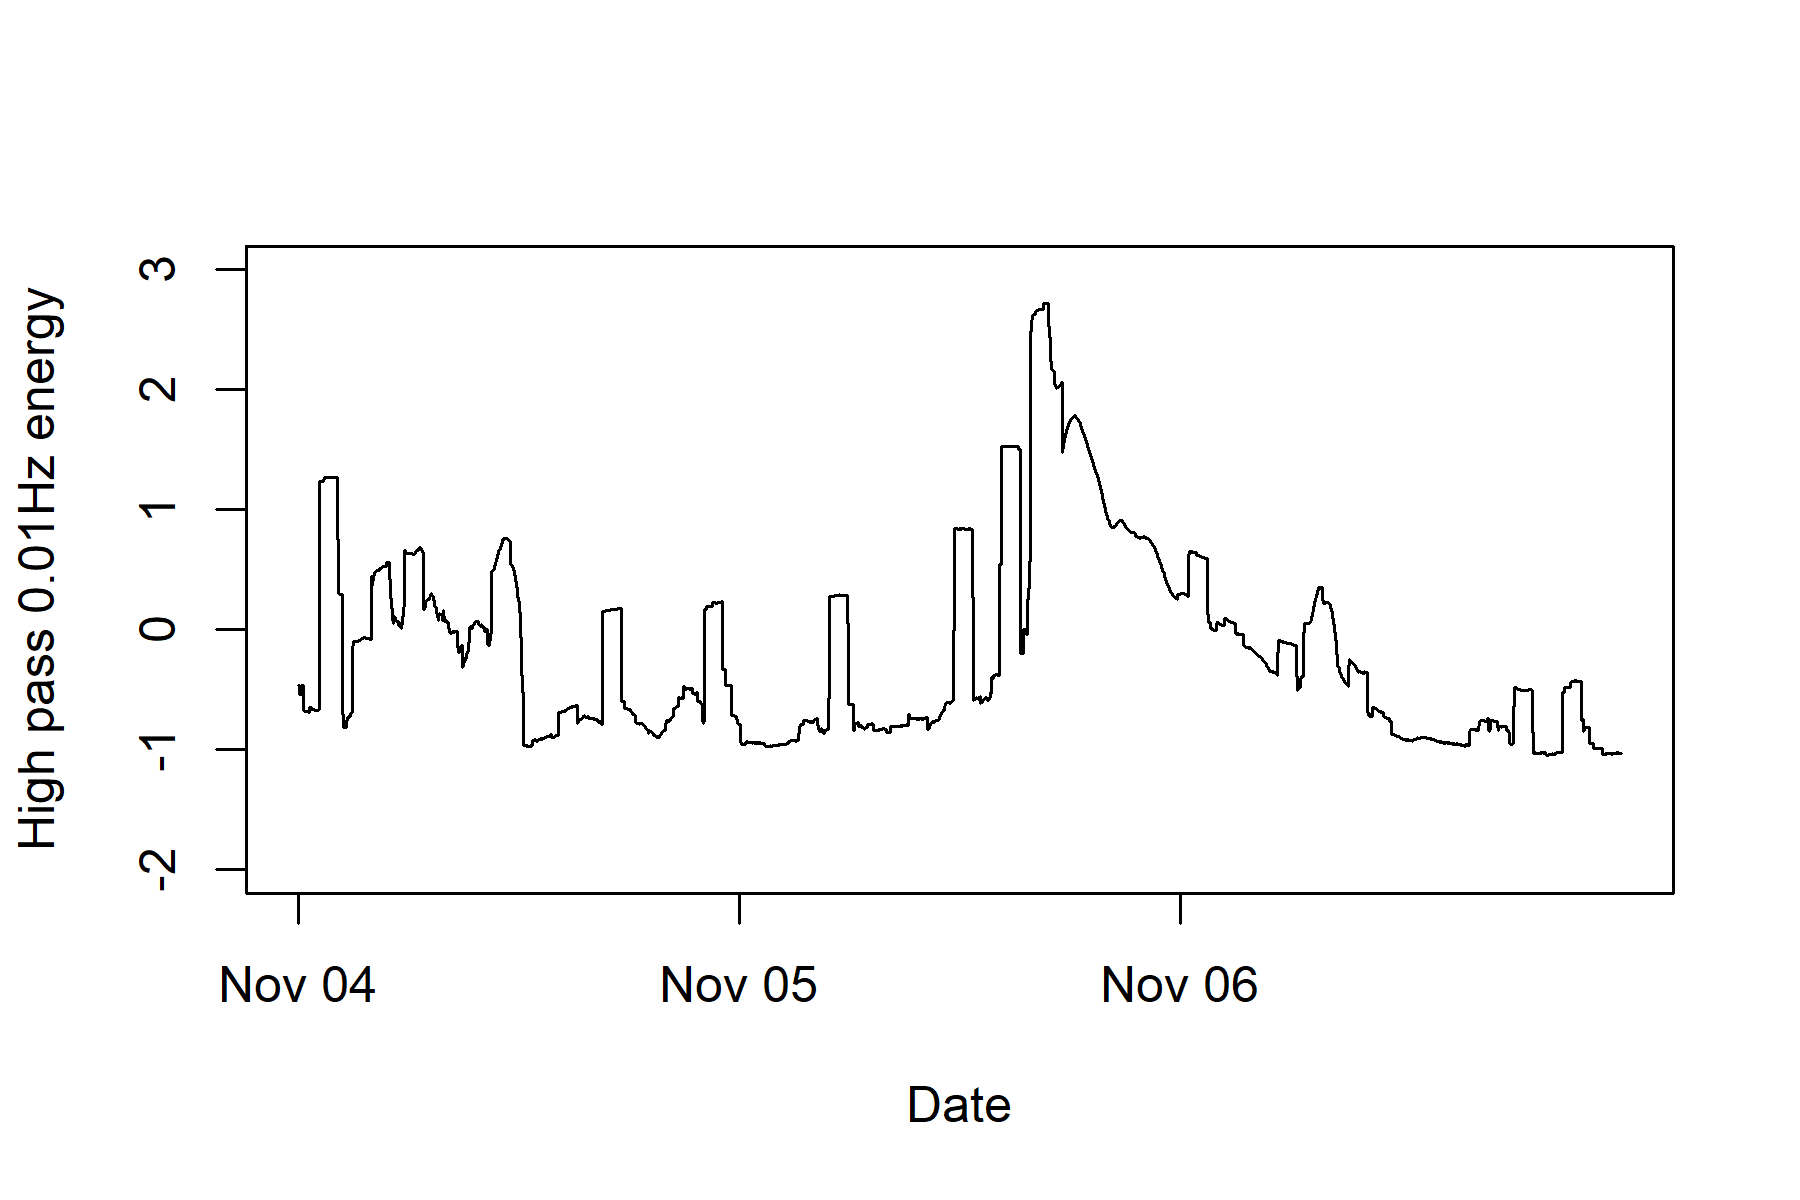}
}
\subfloat[Zoomed in]{\includegraphics[width=3.5in,valign=t]{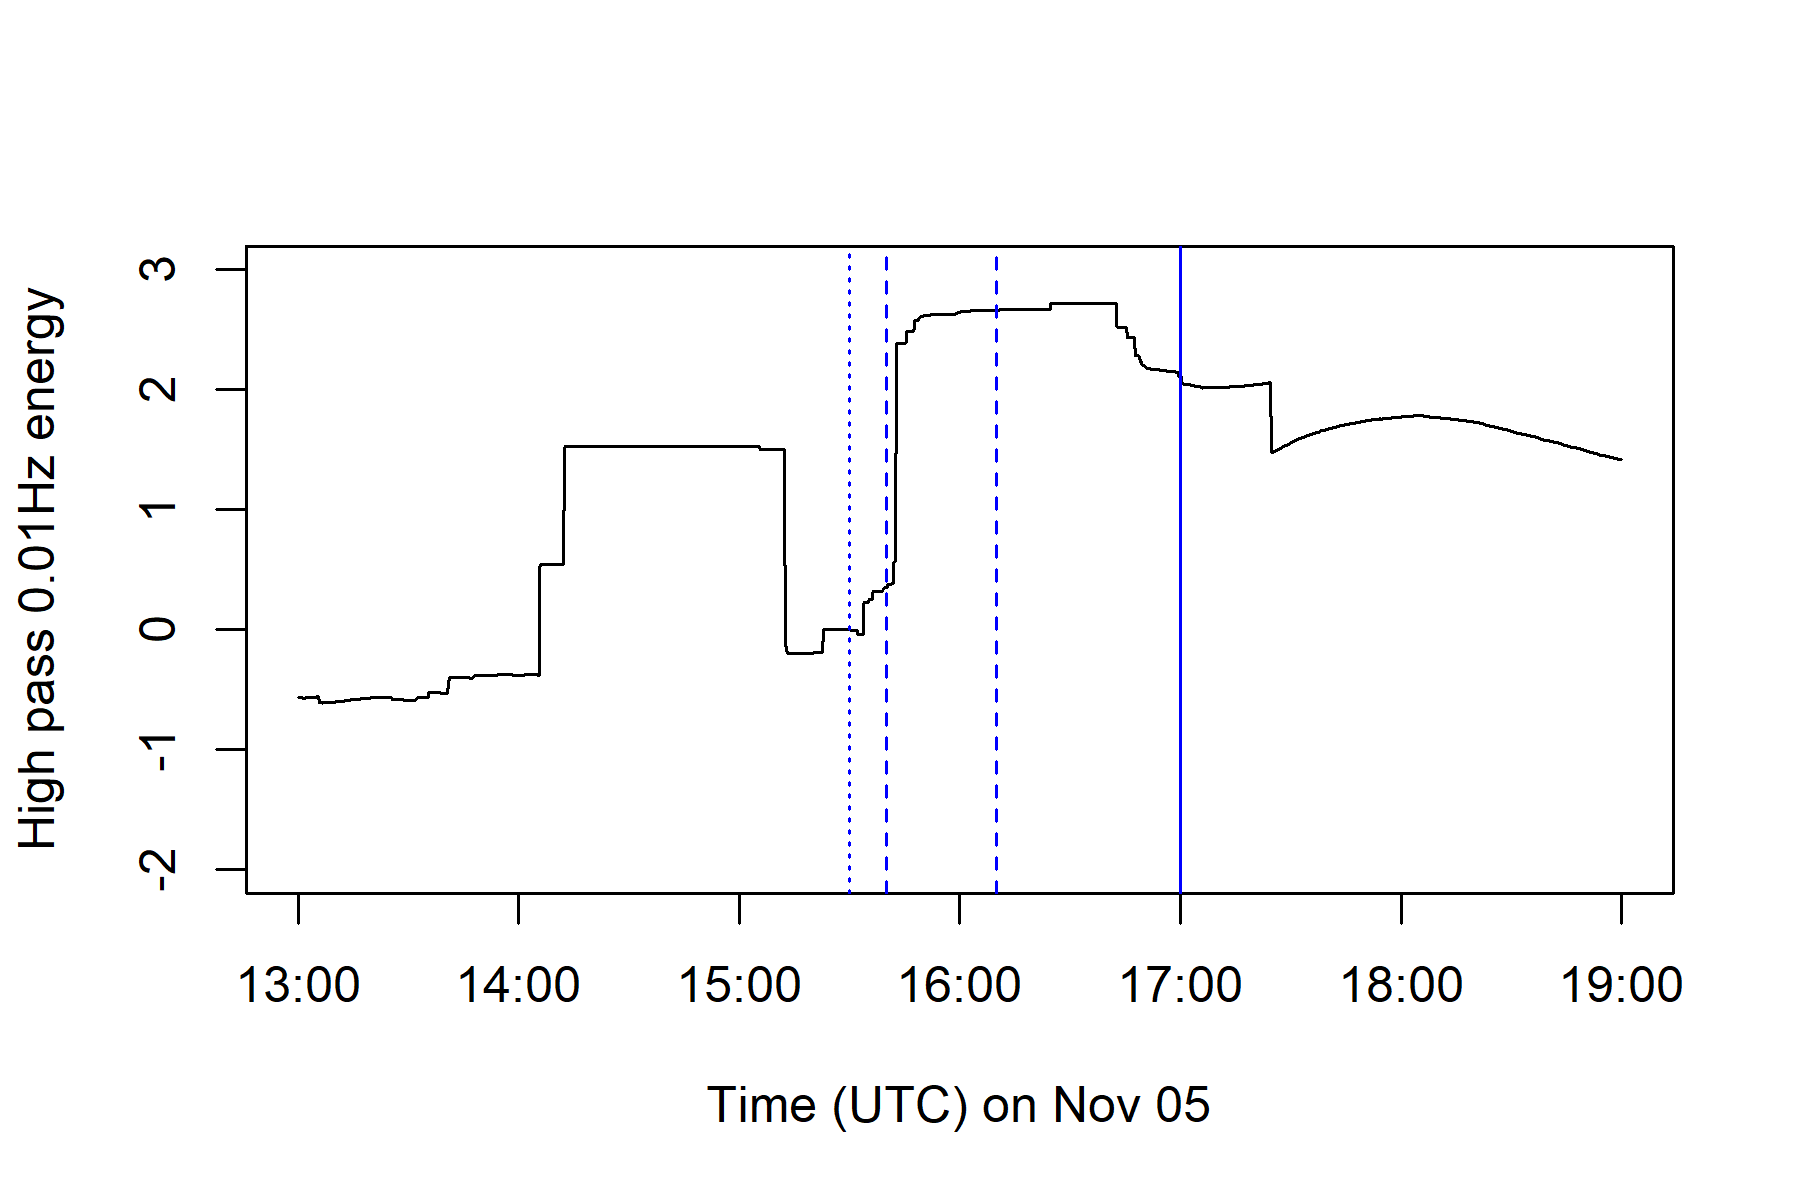}
}
\caption{Training event 1: Time series plots of the three major covariates in the logistic regression.}
\label{fig_train1_covar}
\end{figure*}

\begin{figure*}[!t]
\centering
\subfloat[0.1-20Hz cepstral kurtosis]{\includegraphics[width=3.5in,valign=t]{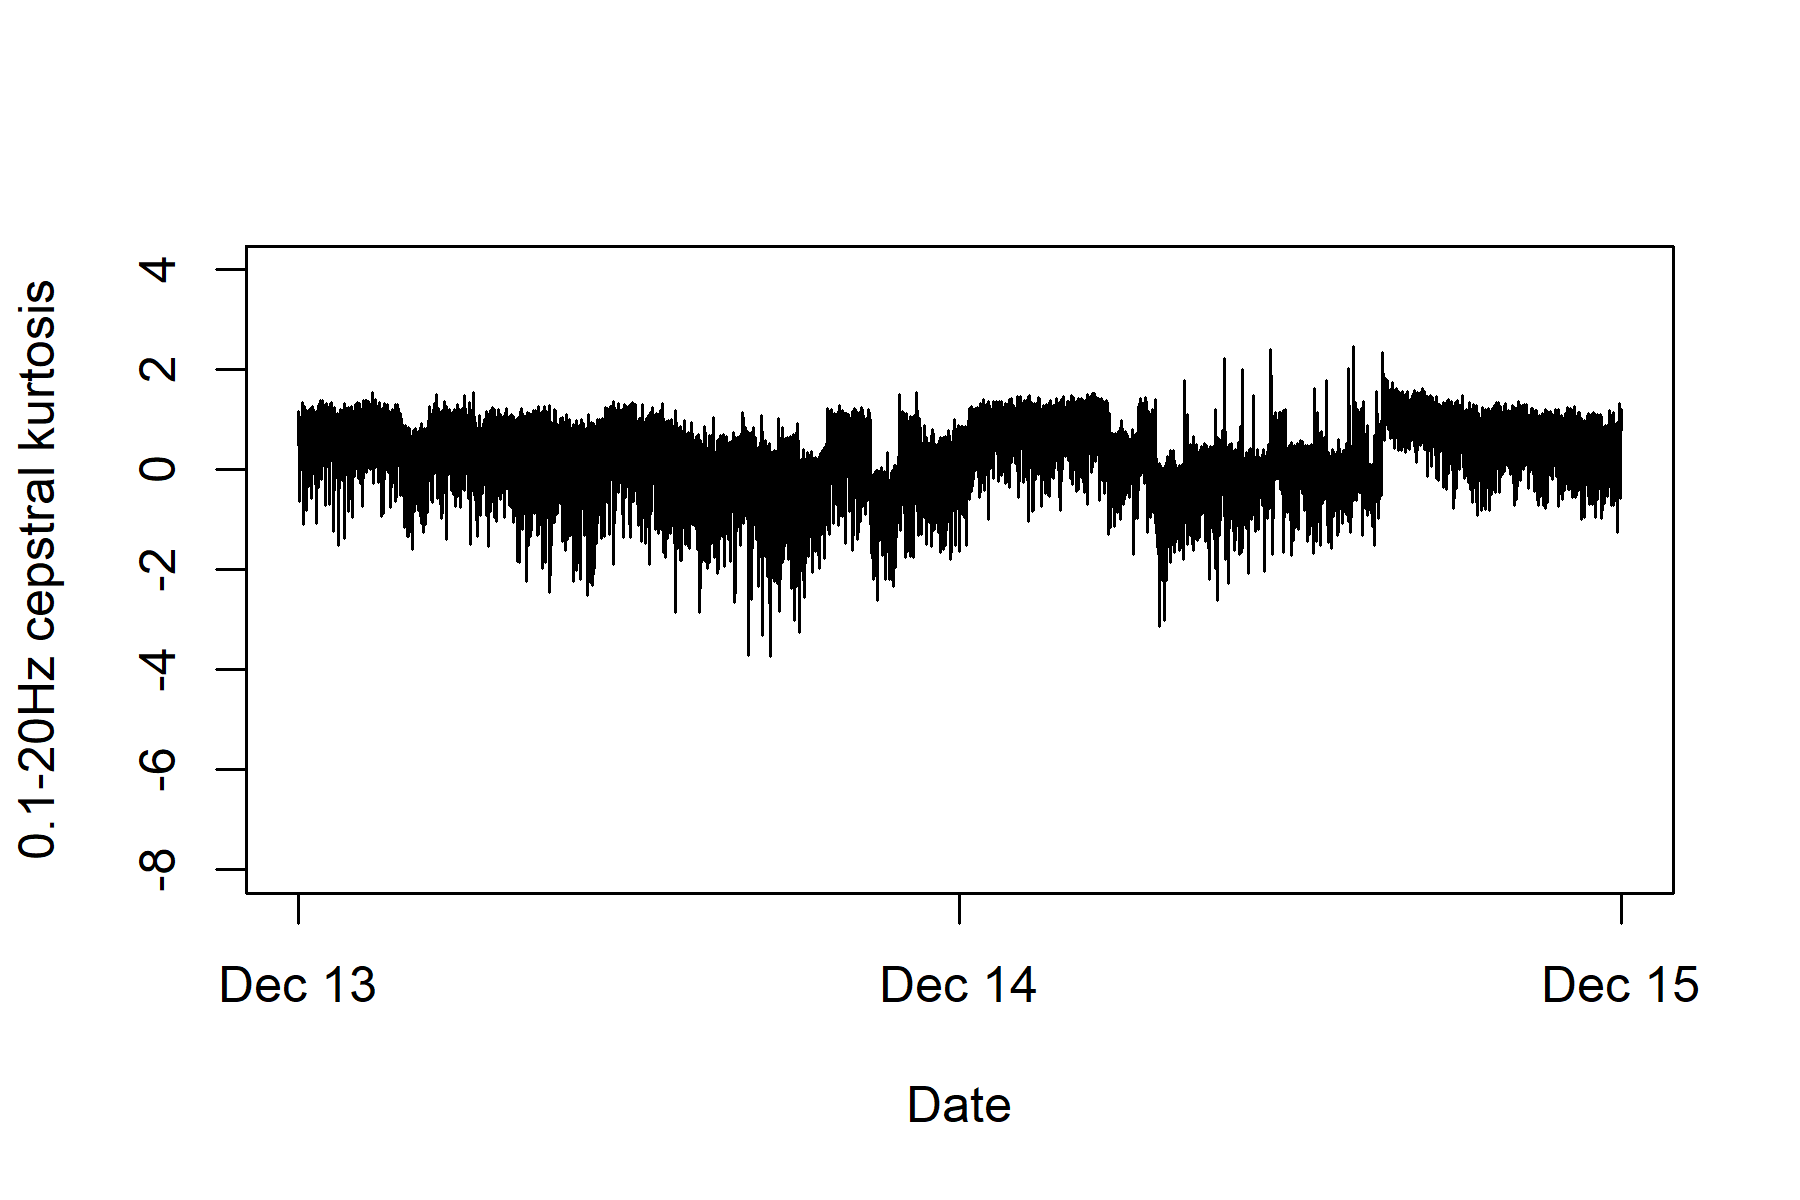}
}
\subfloat[Zoomed in]{\includegraphics[width=3.5in,valign=t]{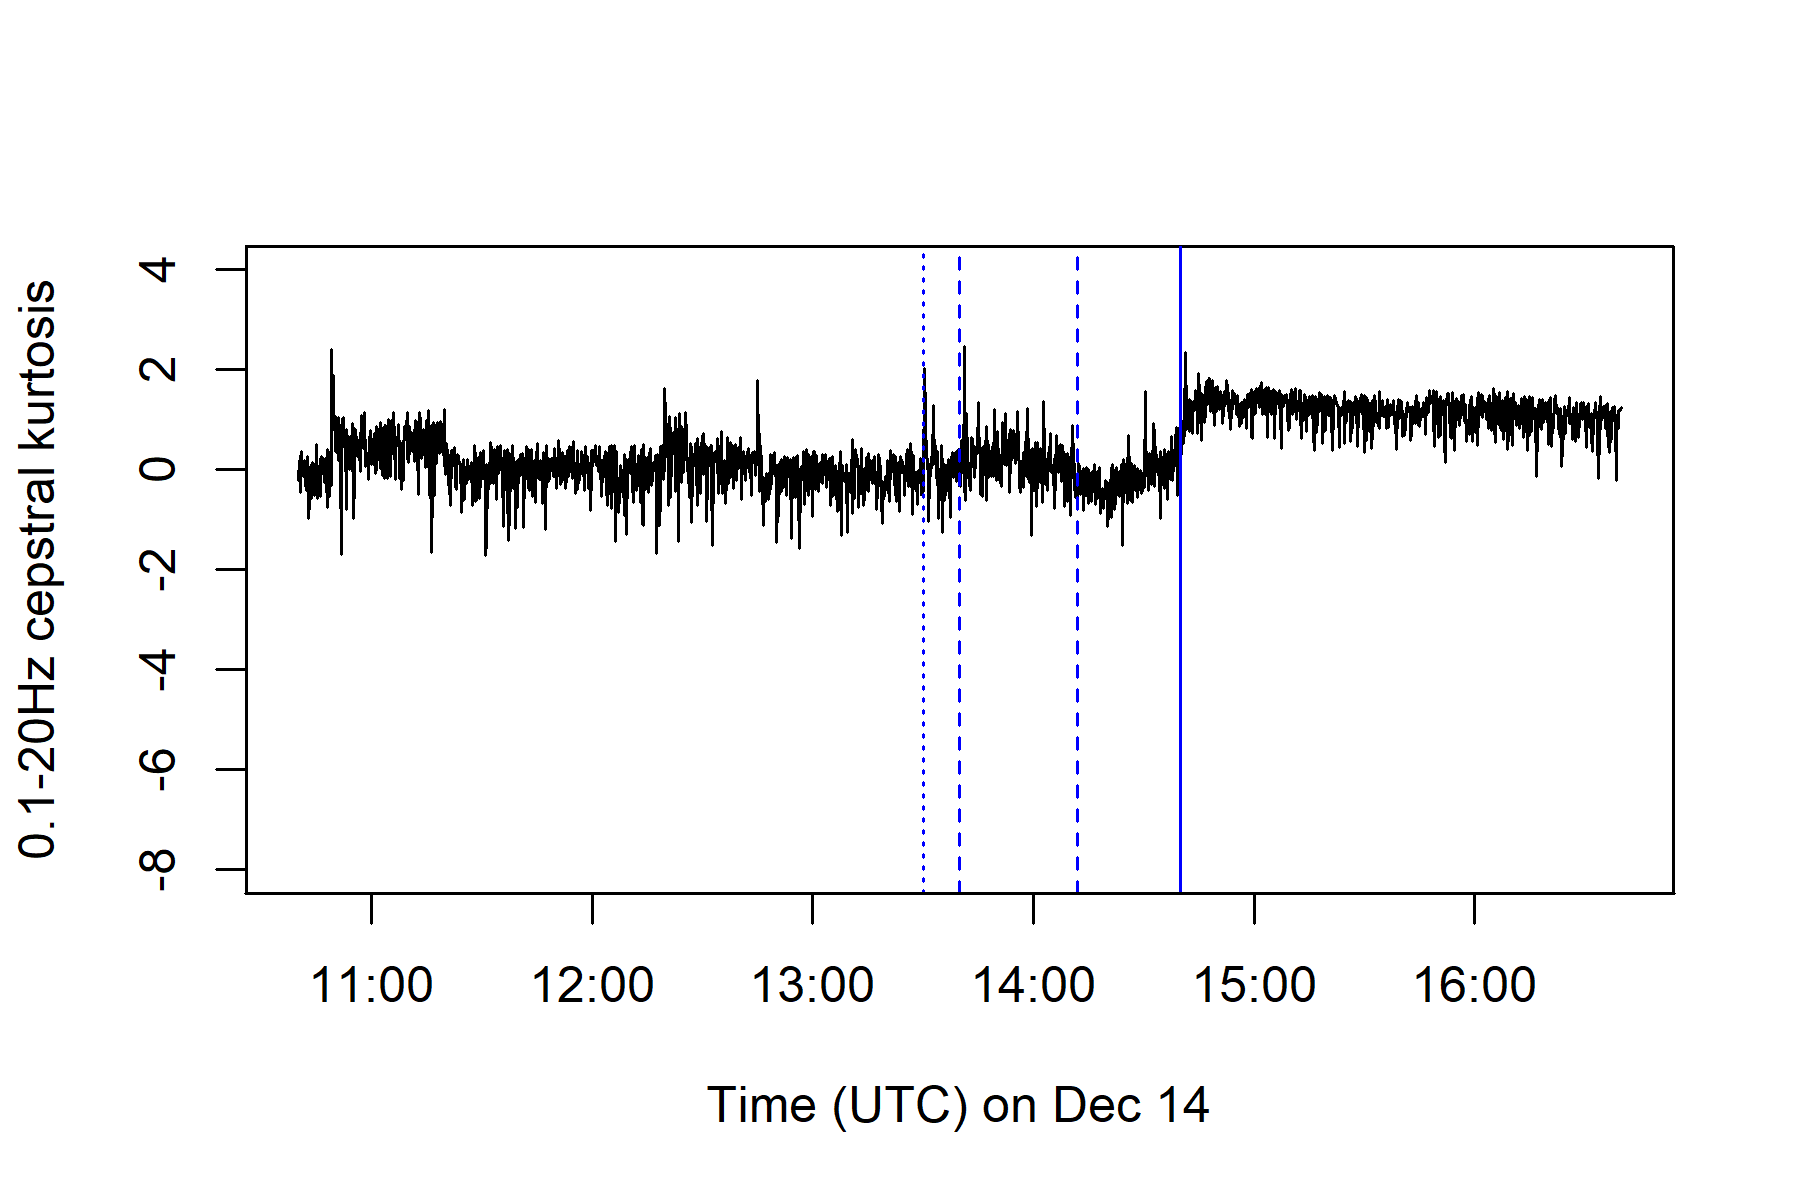}
}
\\
\subfloat[0.1-20Hz cepstral skewness]{\includegraphics[width=3.5in,valign=t]{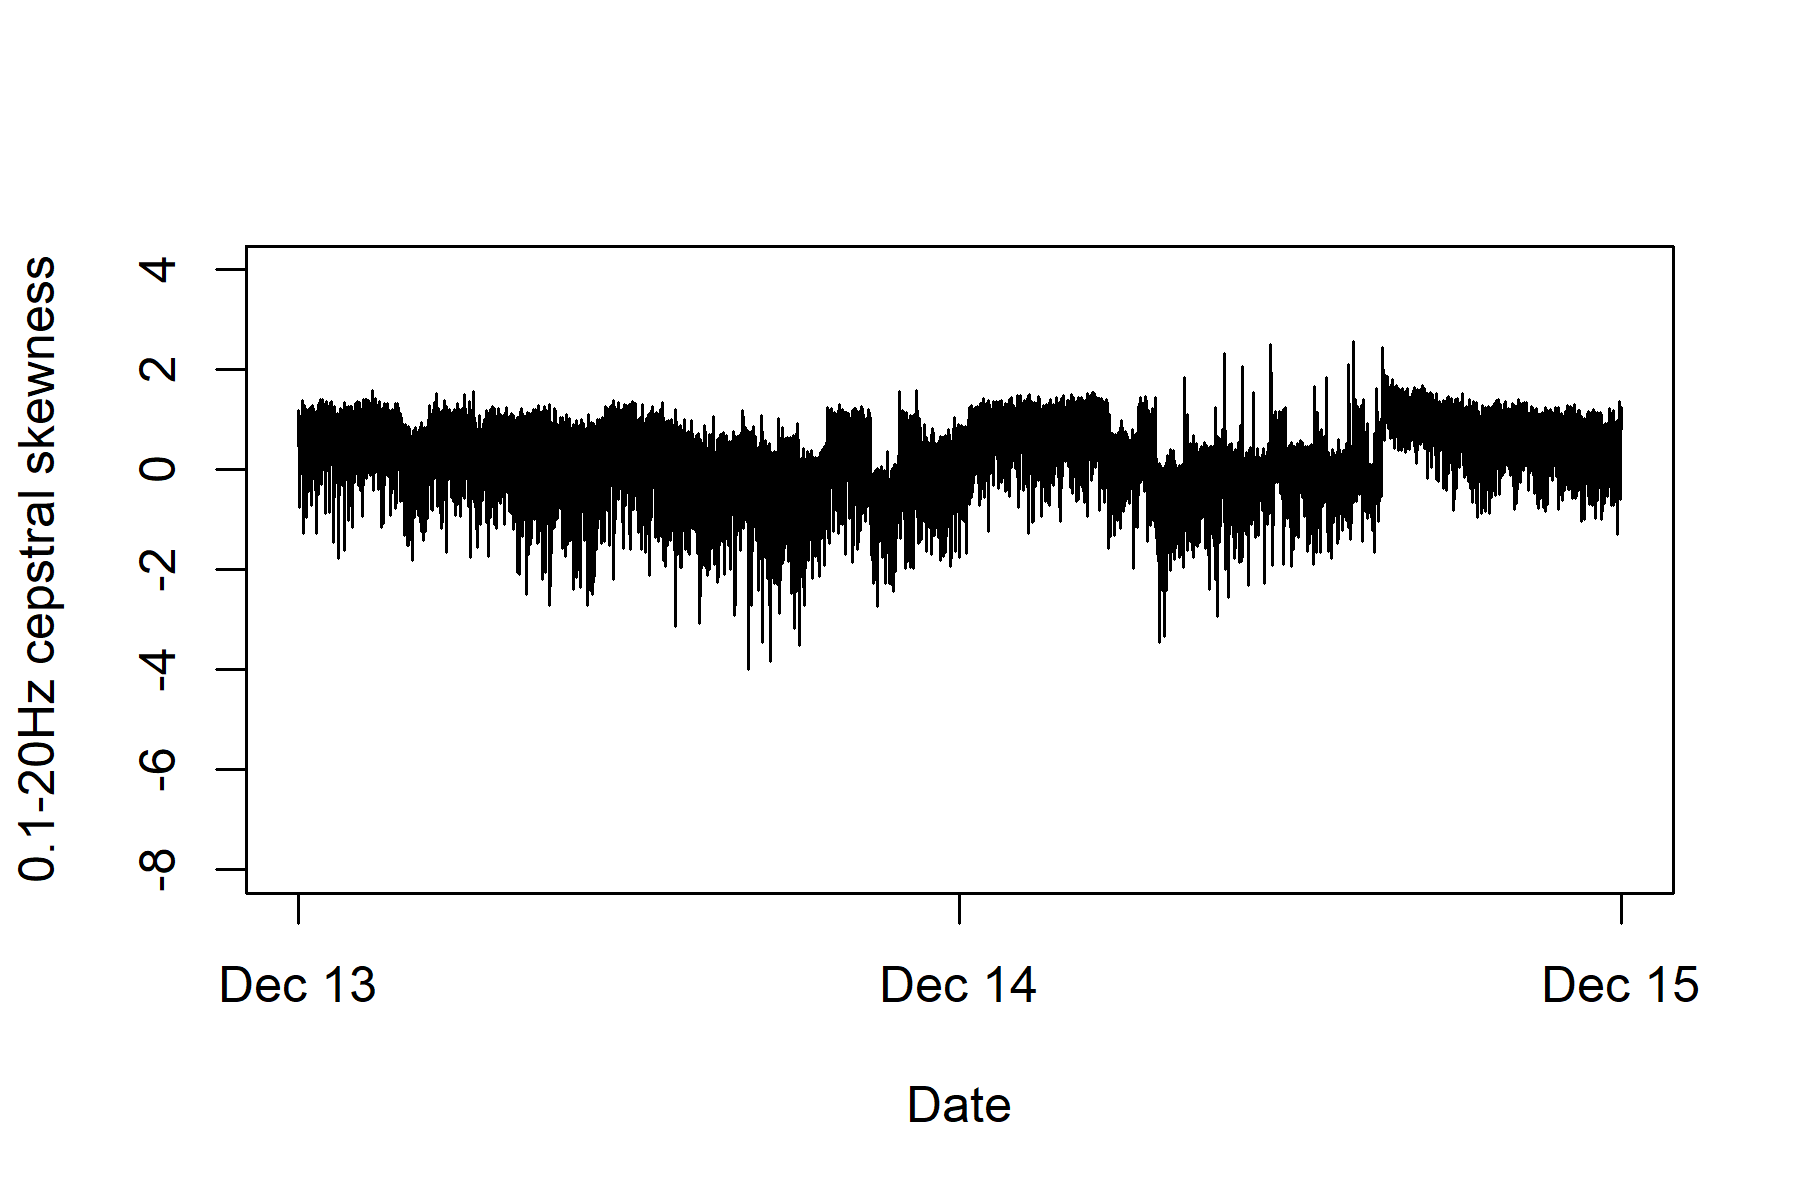}
}
\subfloat[Zoomed in]{\includegraphics[width=3.5in,valign=t]{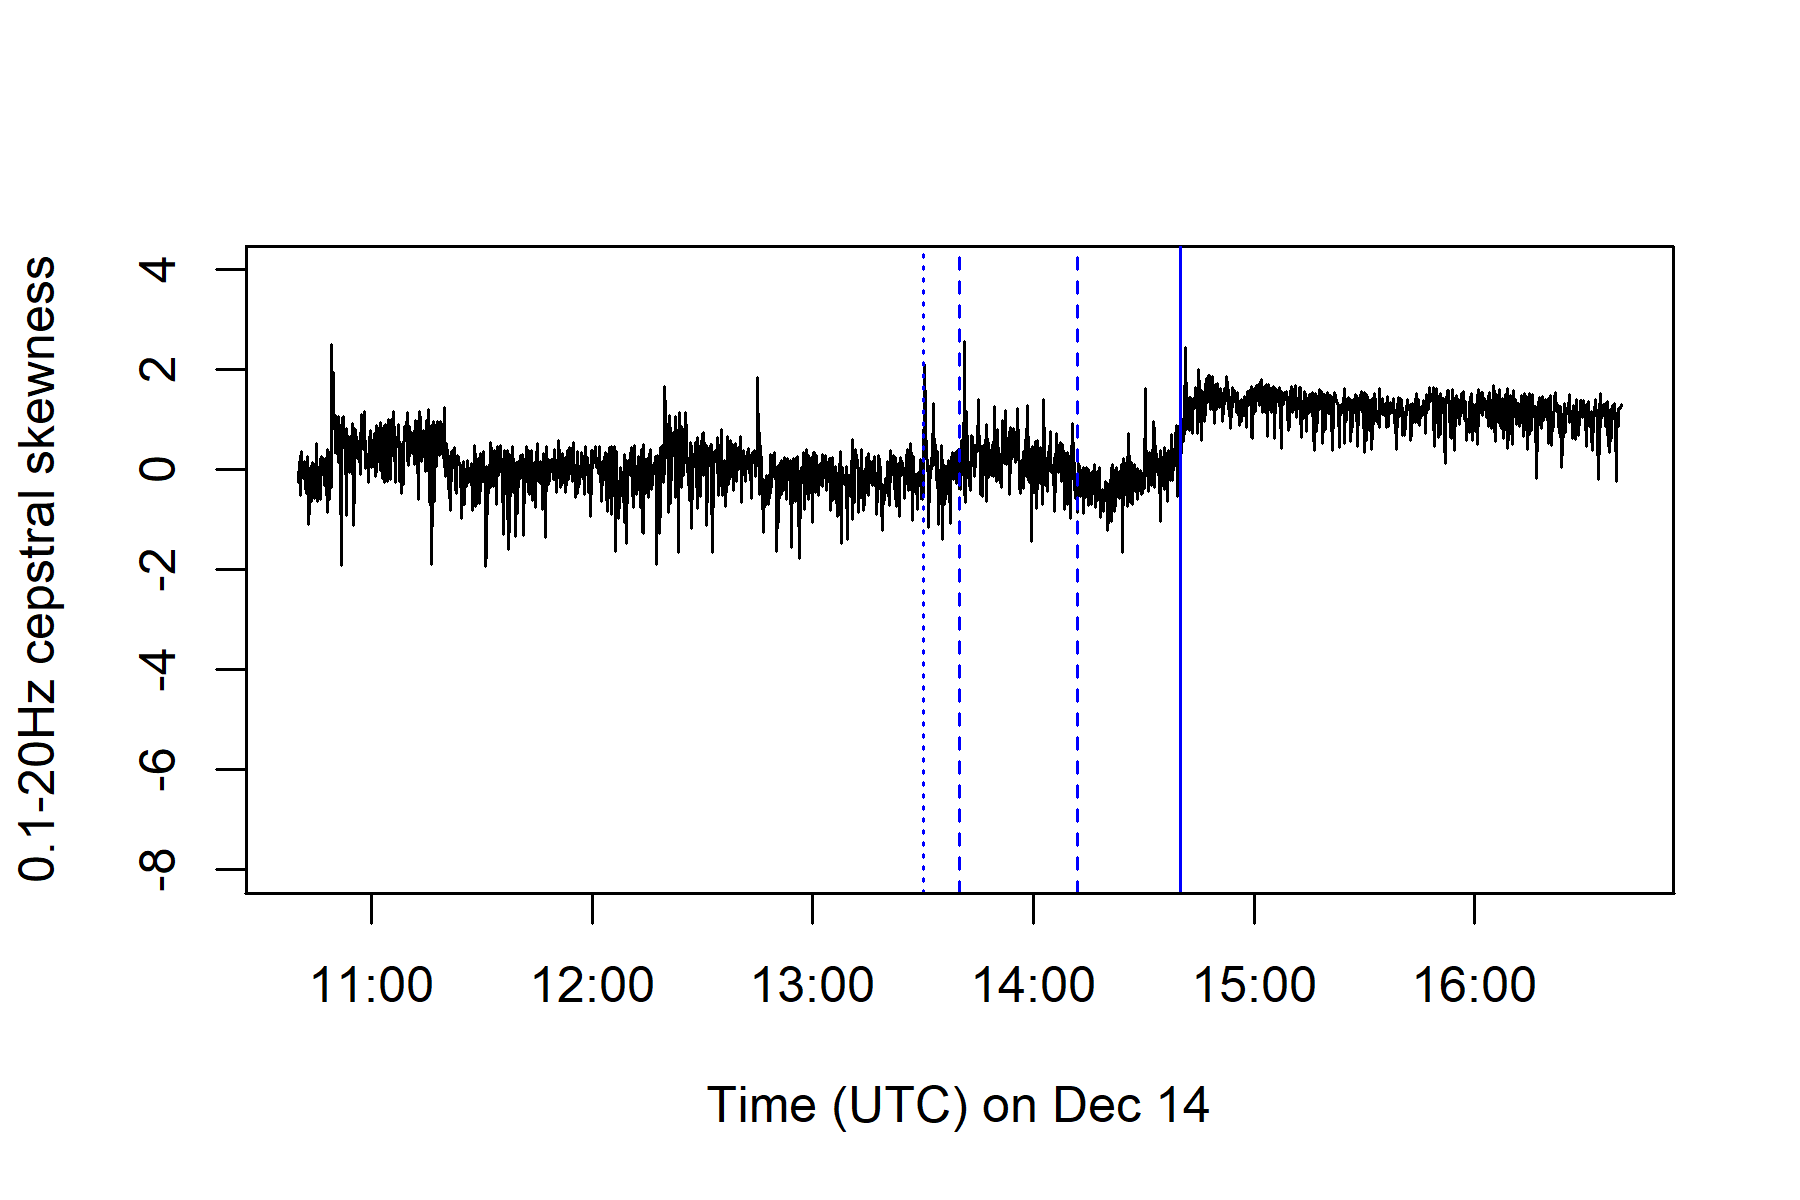}
}
\\
\subfloat[High pass 0.01Hz energy]{\includegraphics[width=3.5in,valign=t]{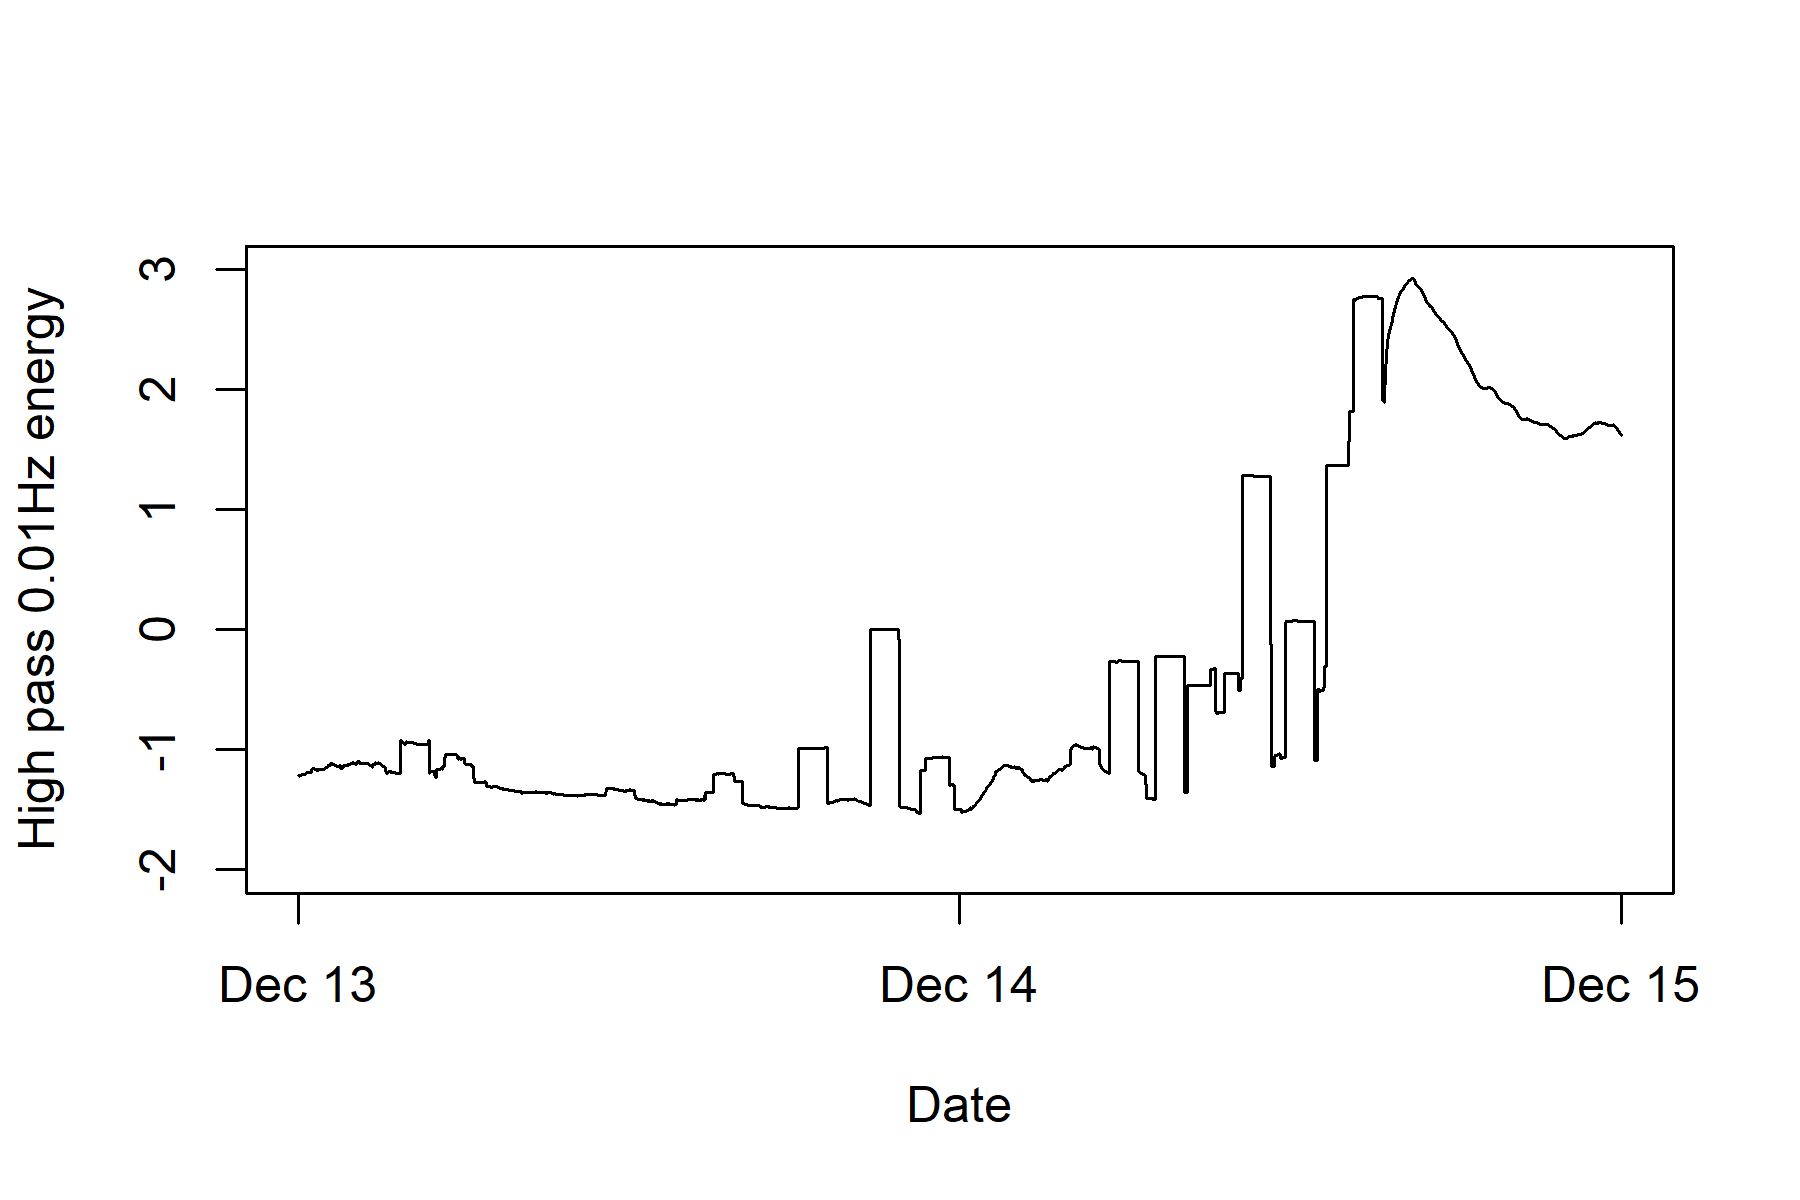}
}
\subfloat[Zoomed in]{\includegraphics[width=3.5in,valign=t]{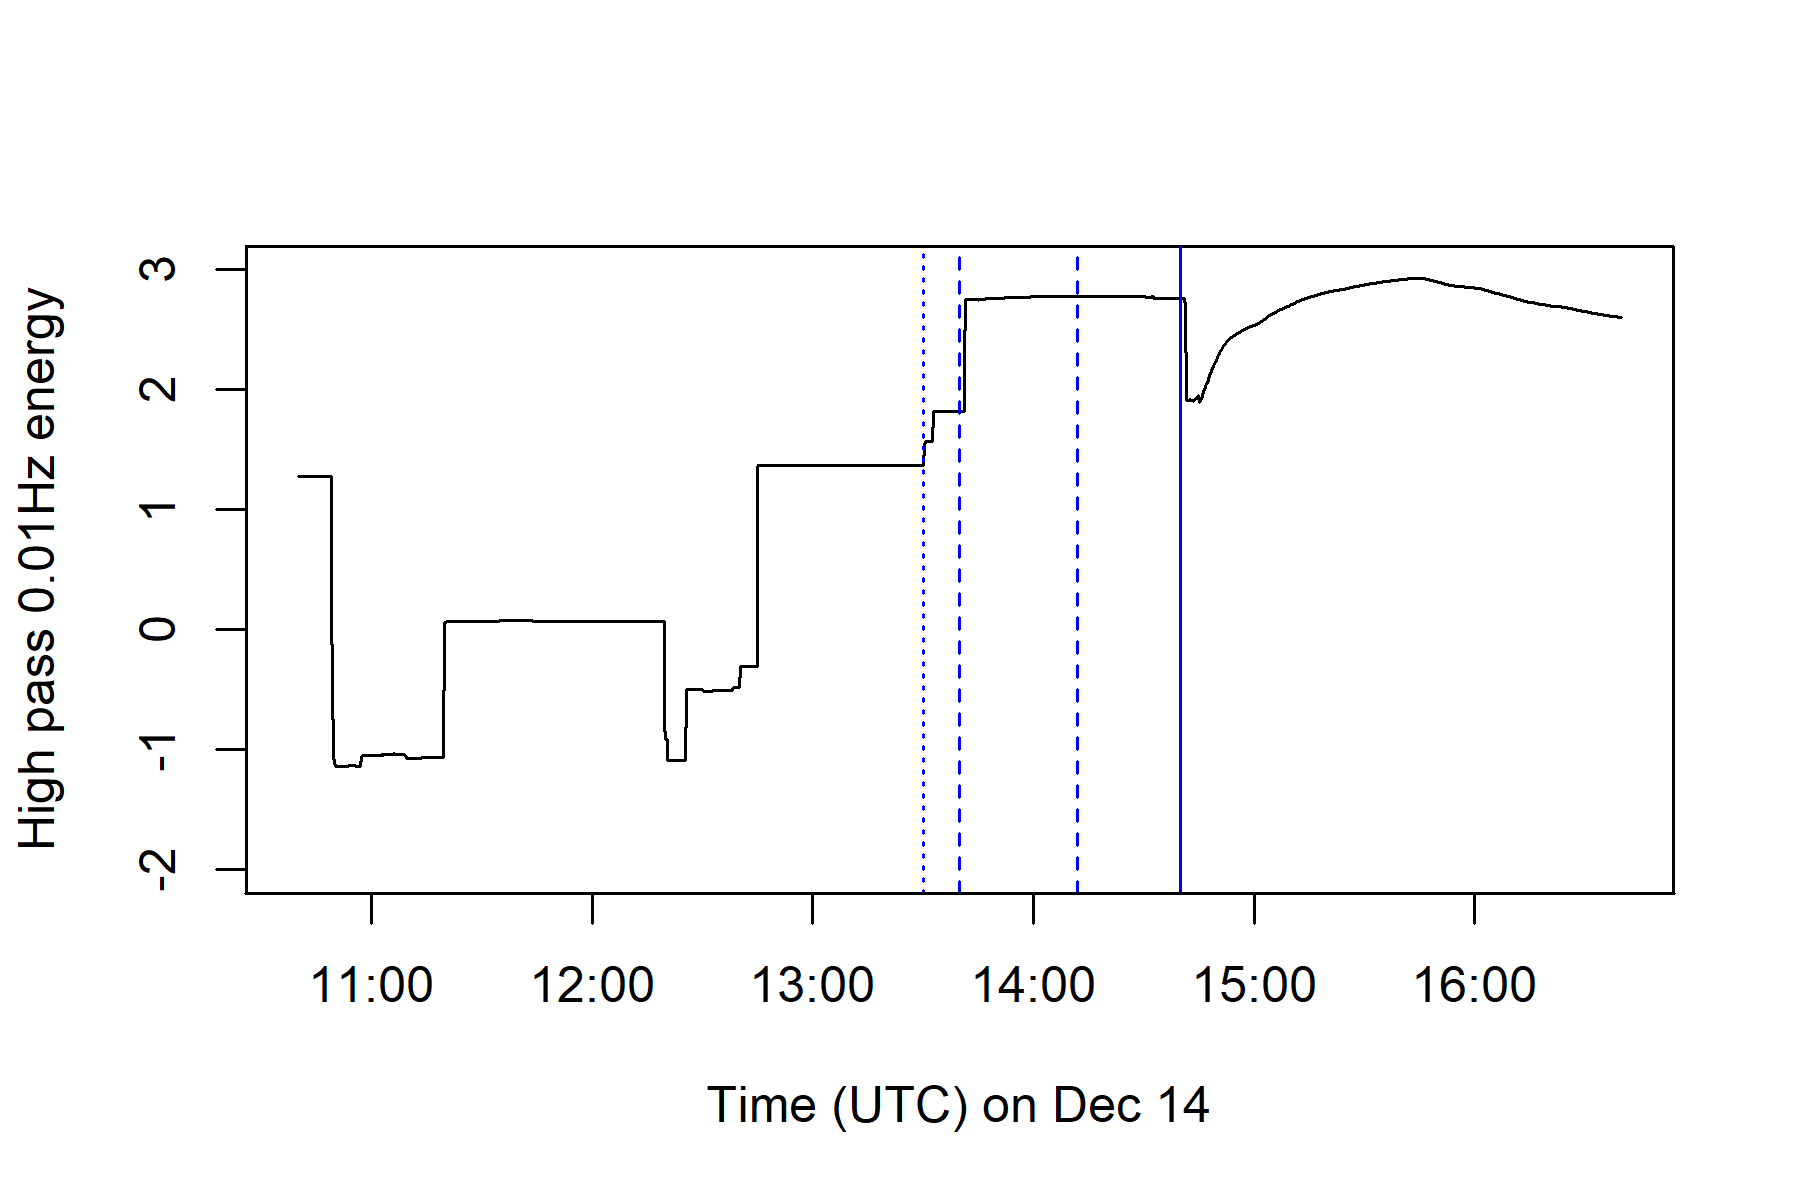}
}
\caption{Training event 2: Time series plots of the three major covariates in the logistic regression.}
\label{fig_train2_covar}
\end{figure*}

\begin{figure*}[!t]
\centering
\subfloat[0.1-20Hz cepstral kurtosis]{\includegraphics[width=3.5in,valign=t]{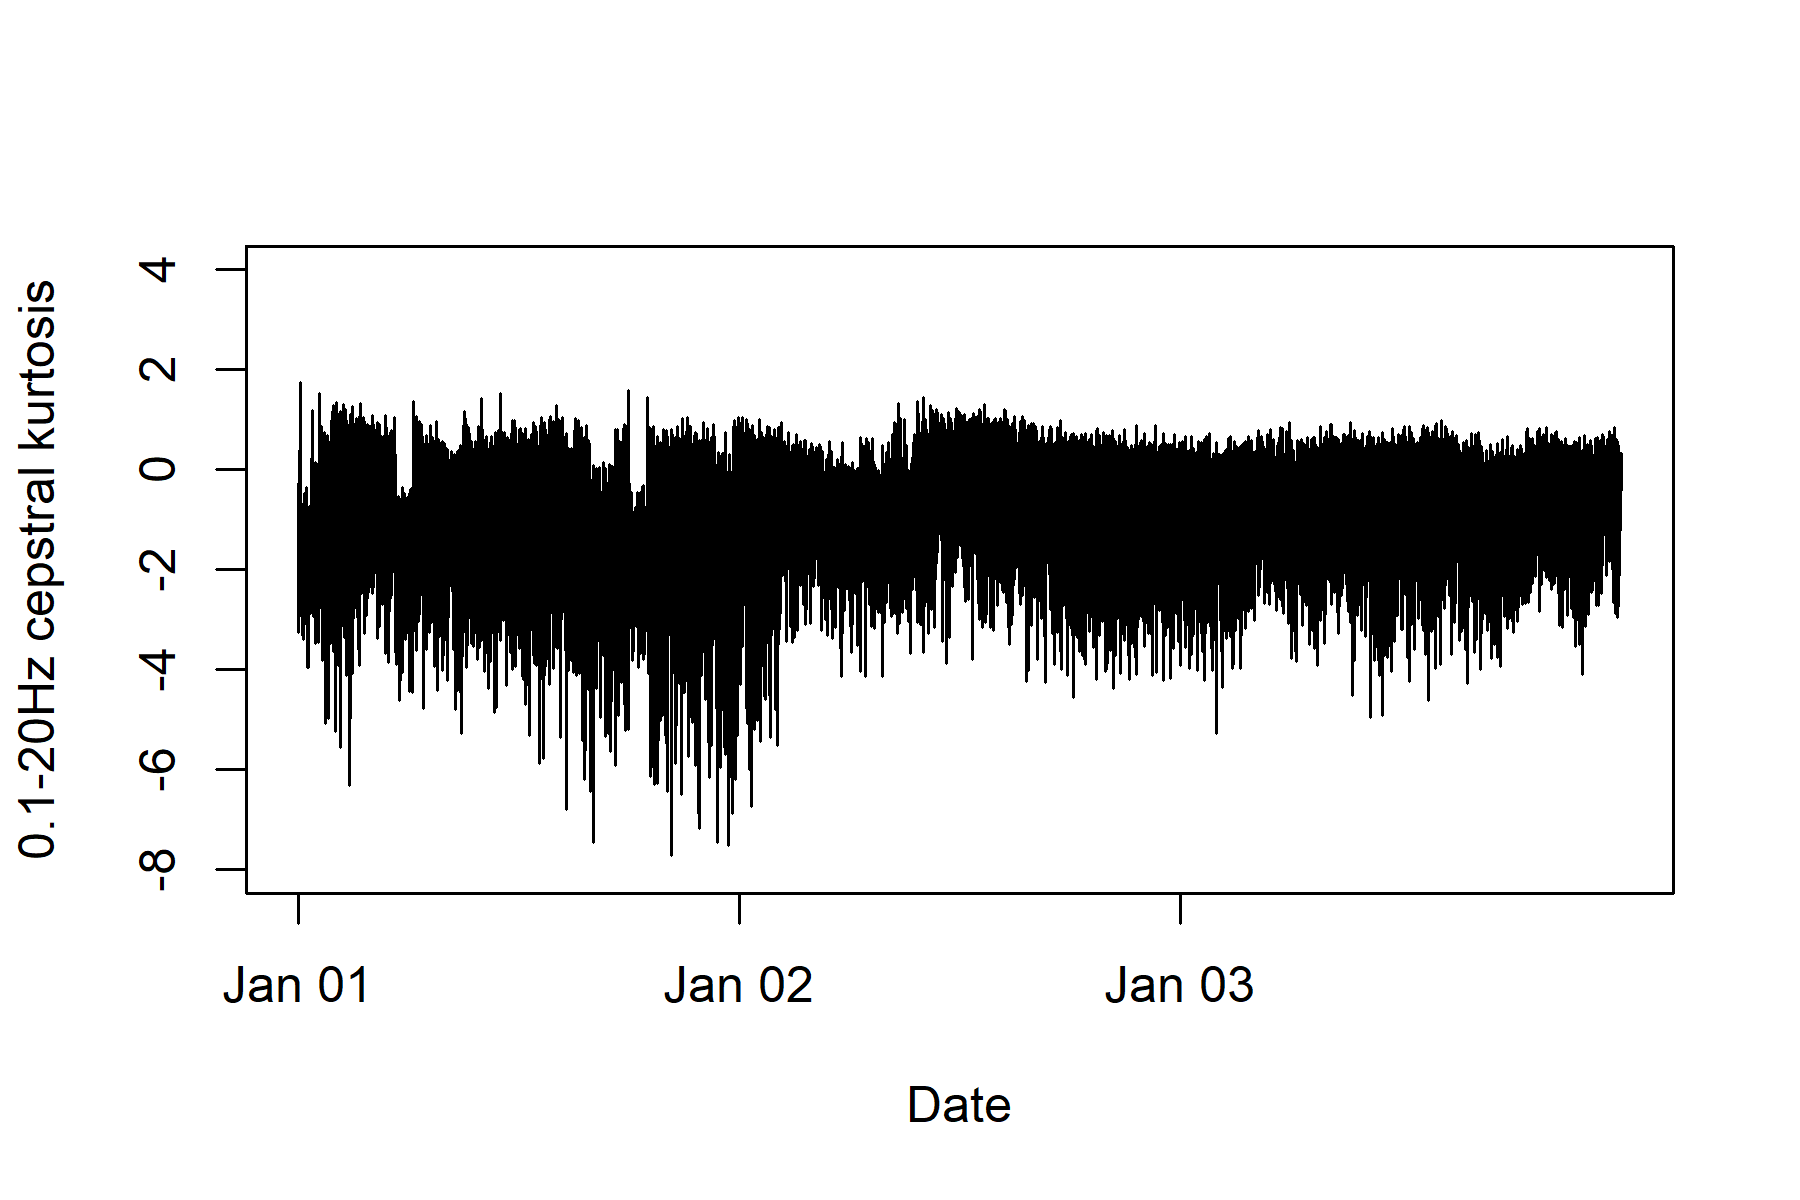}
}
\subfloat[Zoomed in]{\includegraphics[width=3.5in,valign=t]{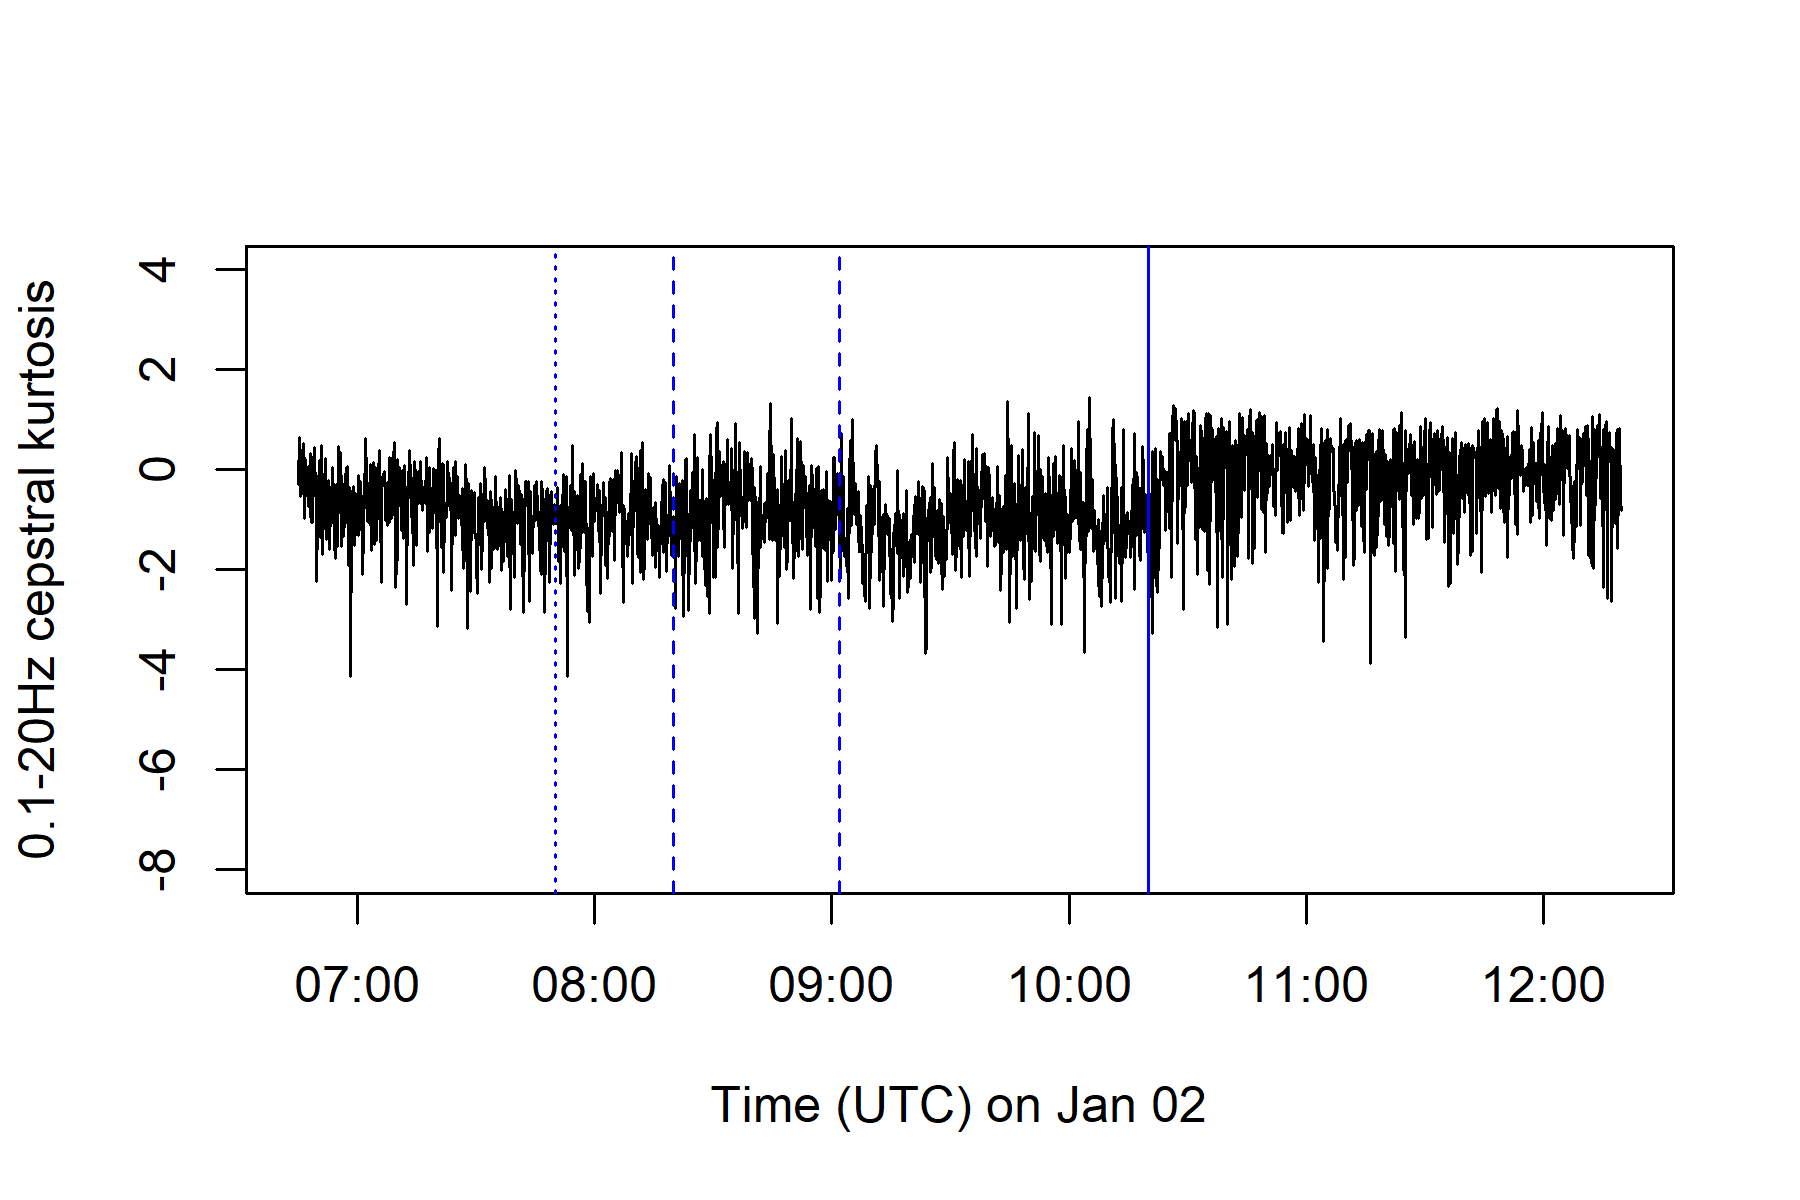}
}
\\
\subfloat[0.1-20Hz cepstral skewness]{\includegraphics[width=3.5in,valign=t]{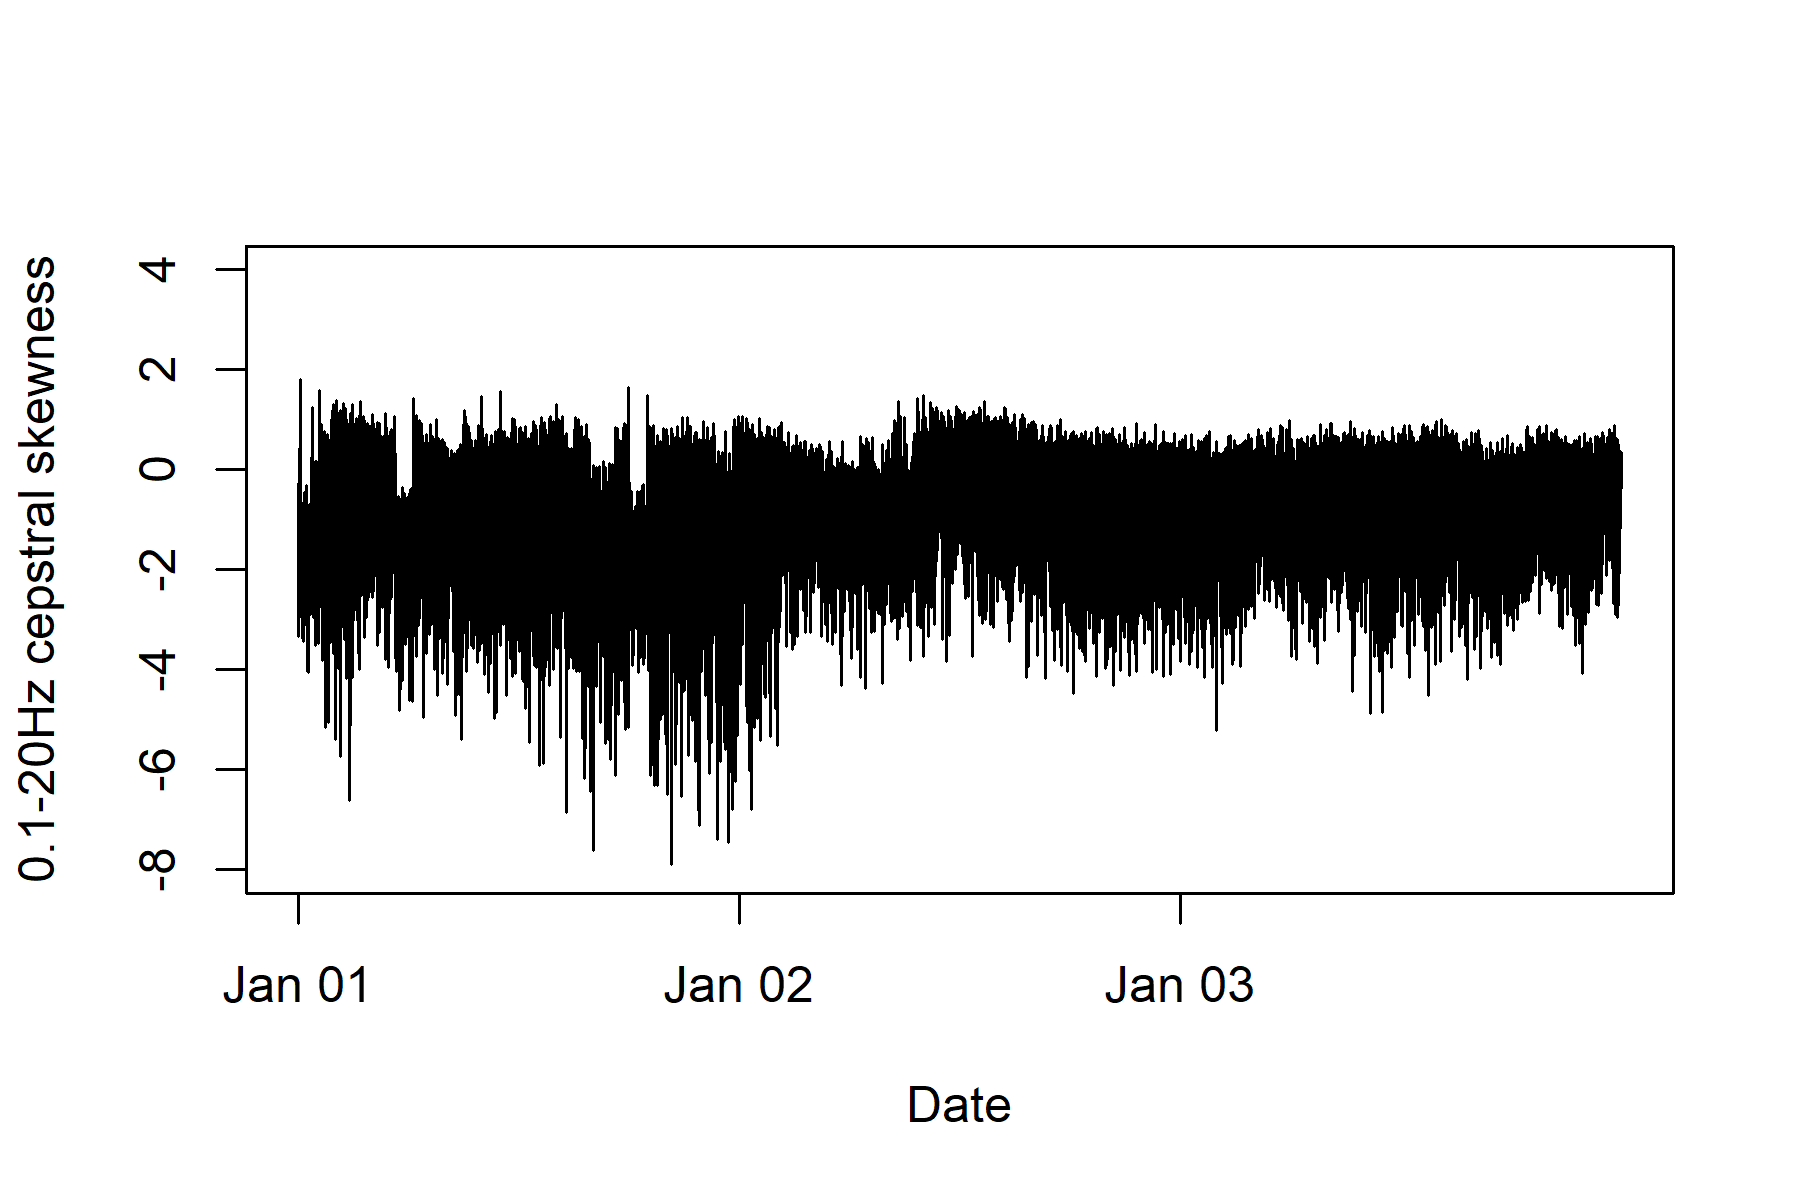}
}
\subfloat[Zoomed in]{\includegraphics[width=3.5in,valign=t]{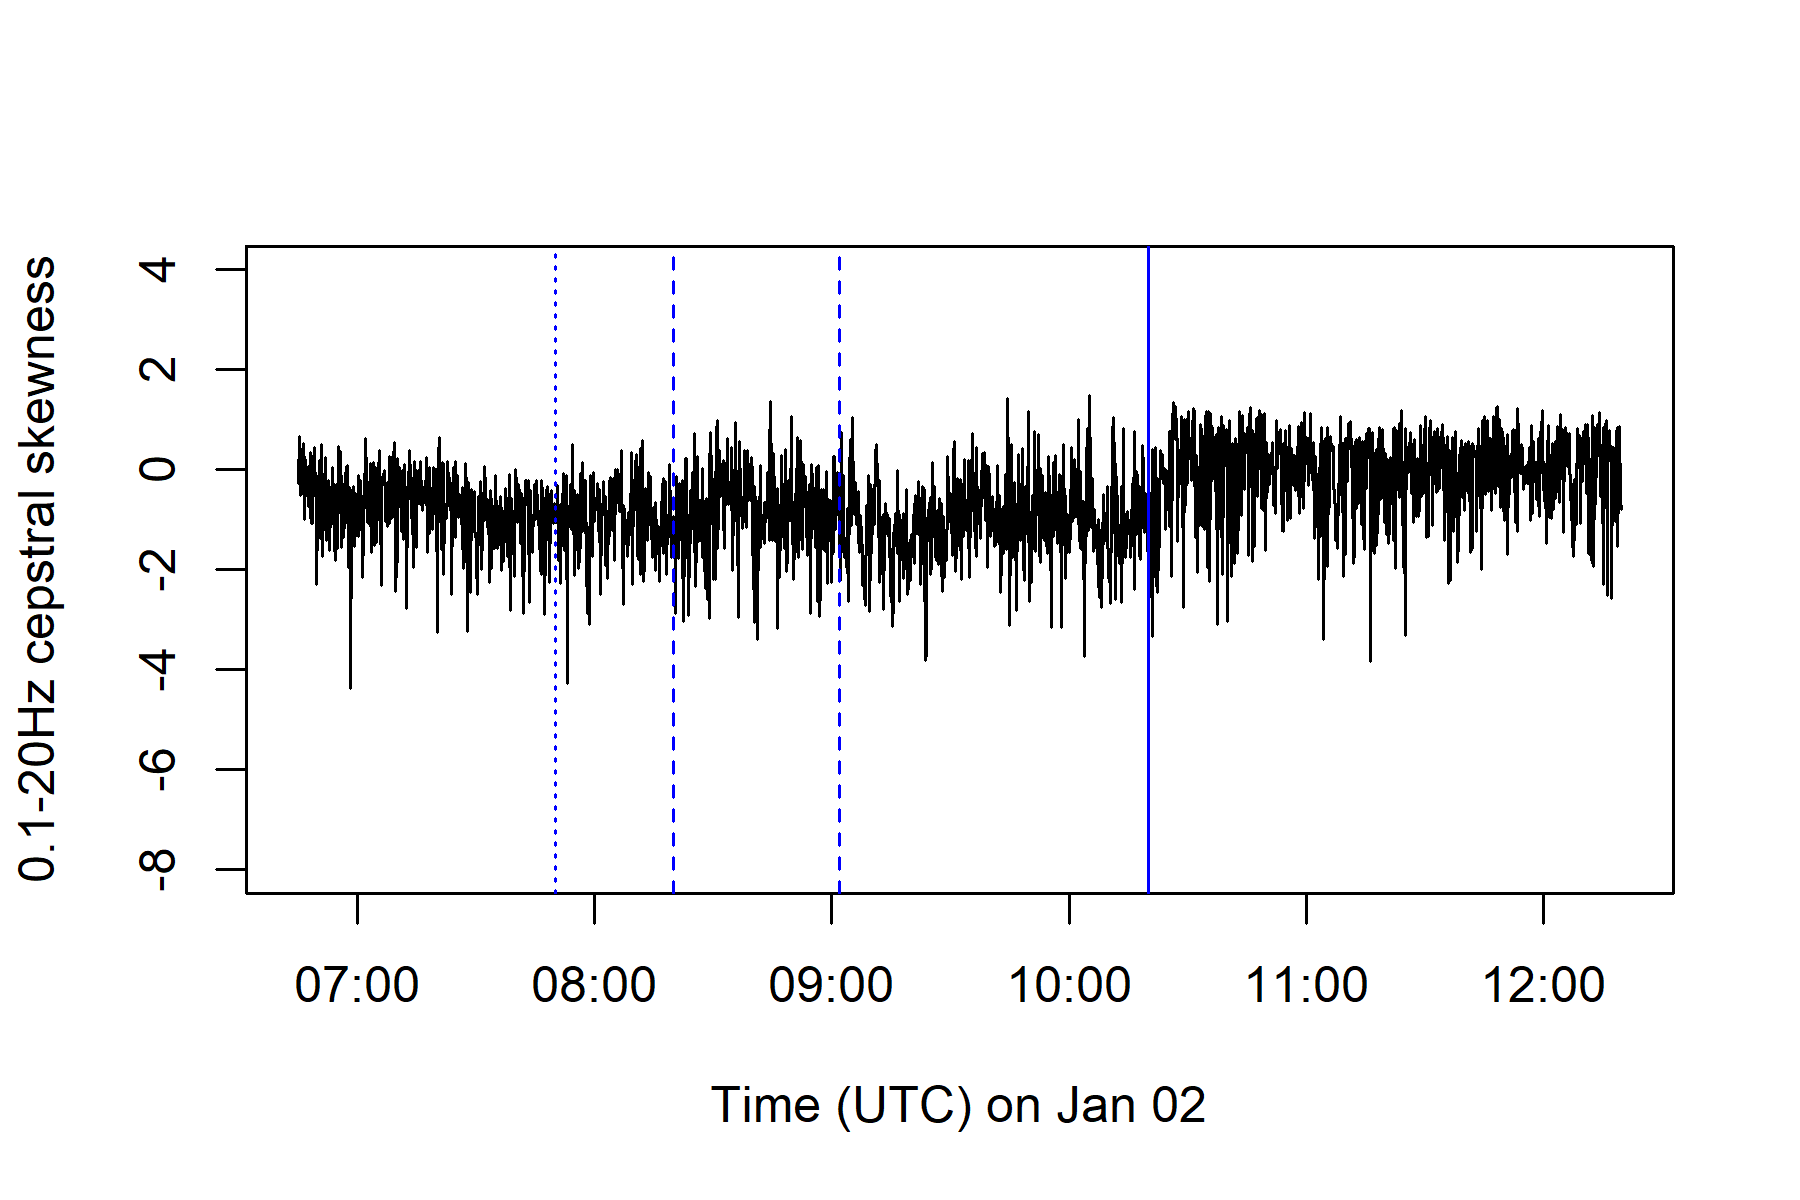}
}
\\
\subfloat[High pass 0.01Hz energy]{\includegraphics[width=3.5in,valign=t]{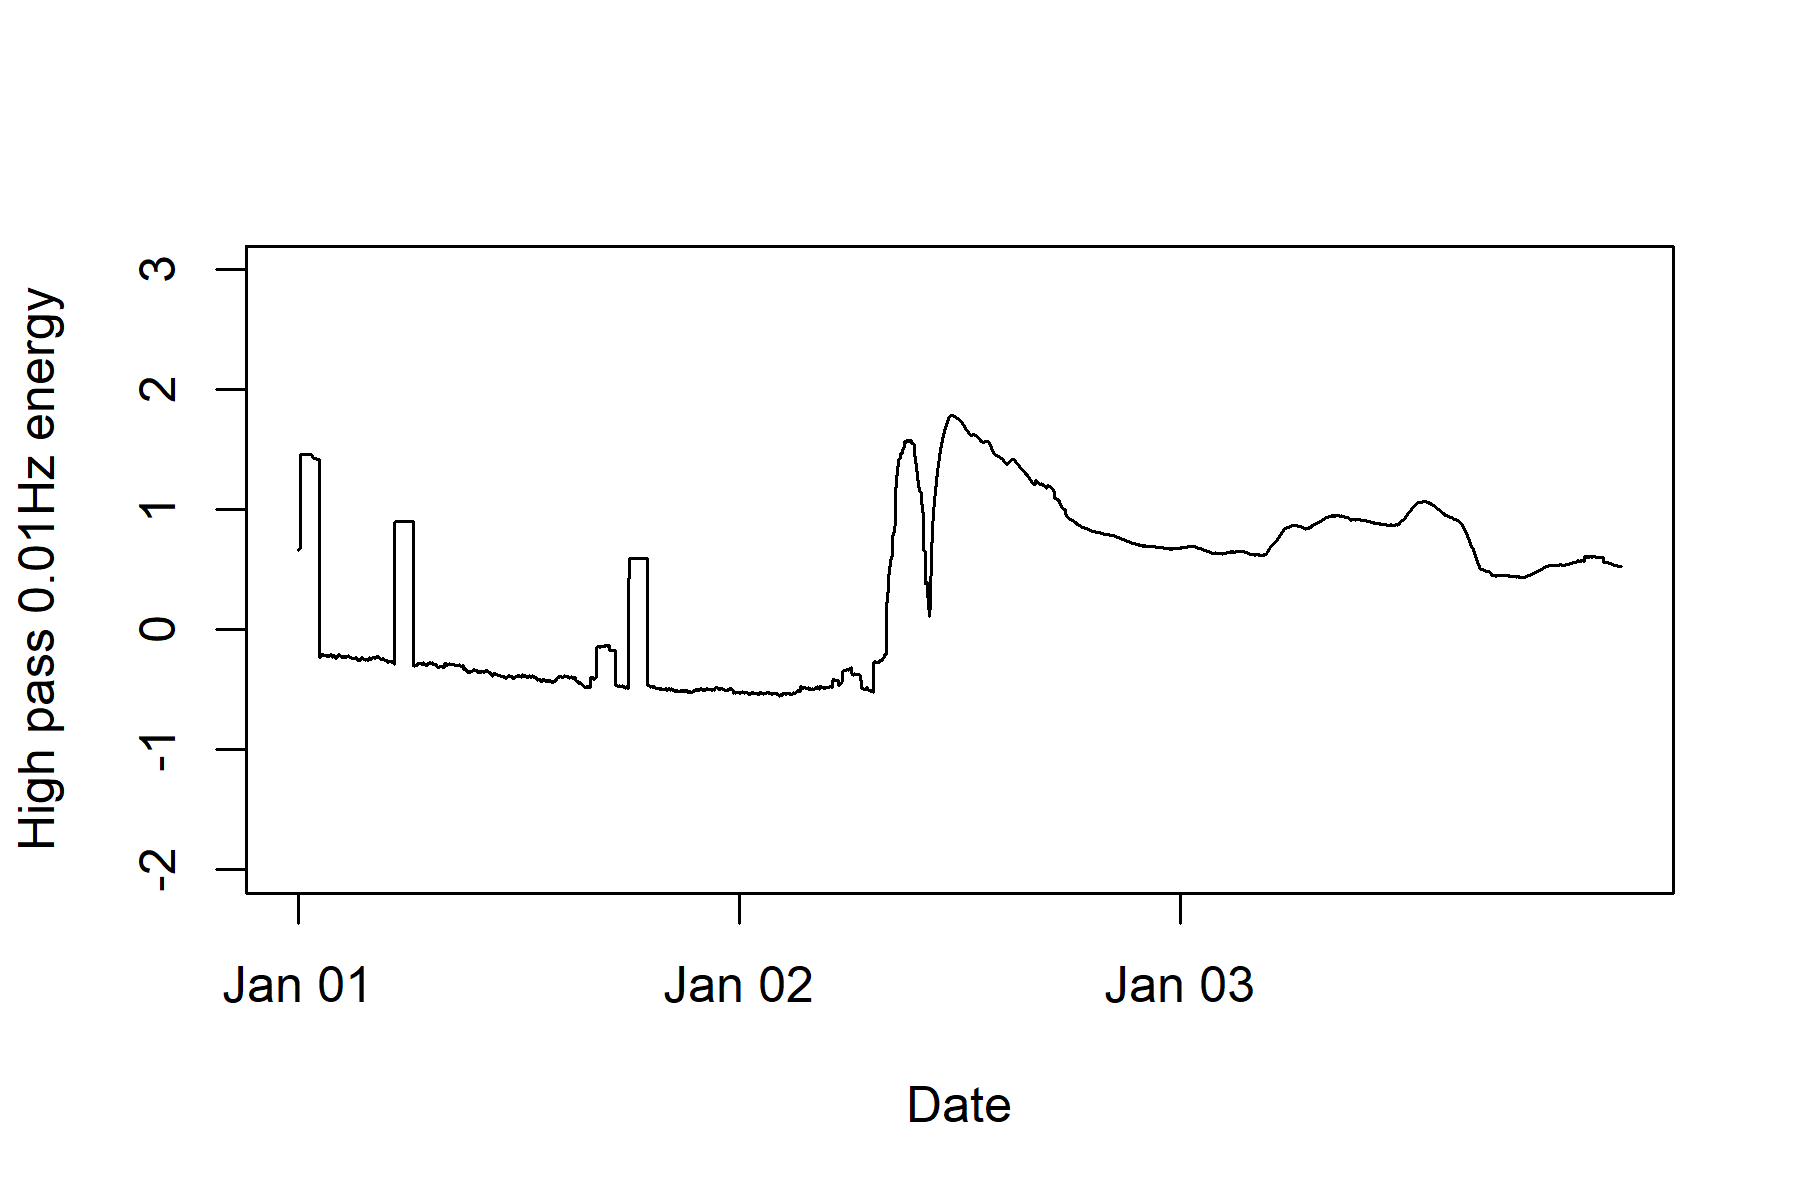}
}
\subfloat[Zoomed in]{\includegraphics[width=3.5in,valign=t]{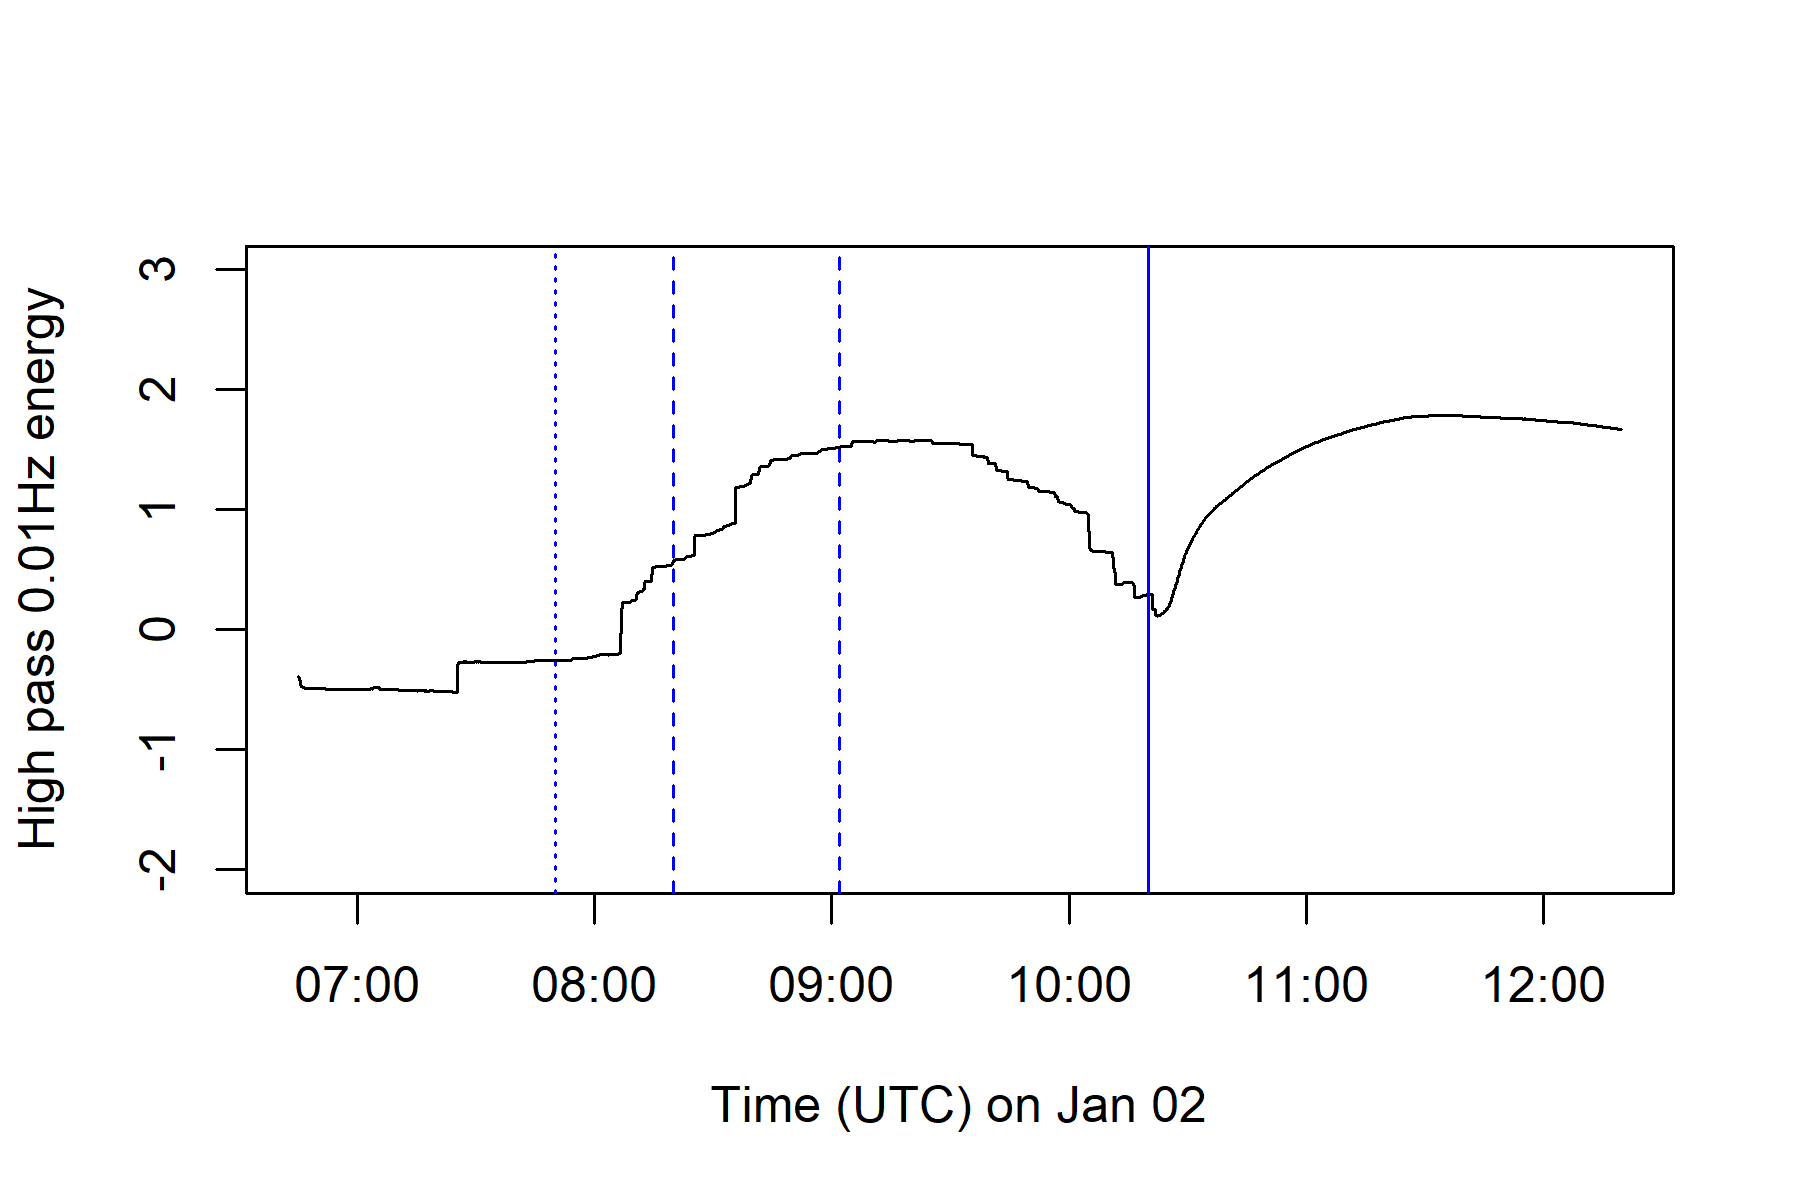}
}
\caption{Training event 3: Time series plots of the three major covariates in the logistic regression.}
\label{fig_train3_covar}
\end{figure*}

\begin{figure*}[!t]
\centering
\subfloat[0.1-20Hz cepstral kurtosis]{\includegraphics[width=3.5in,valign=t]{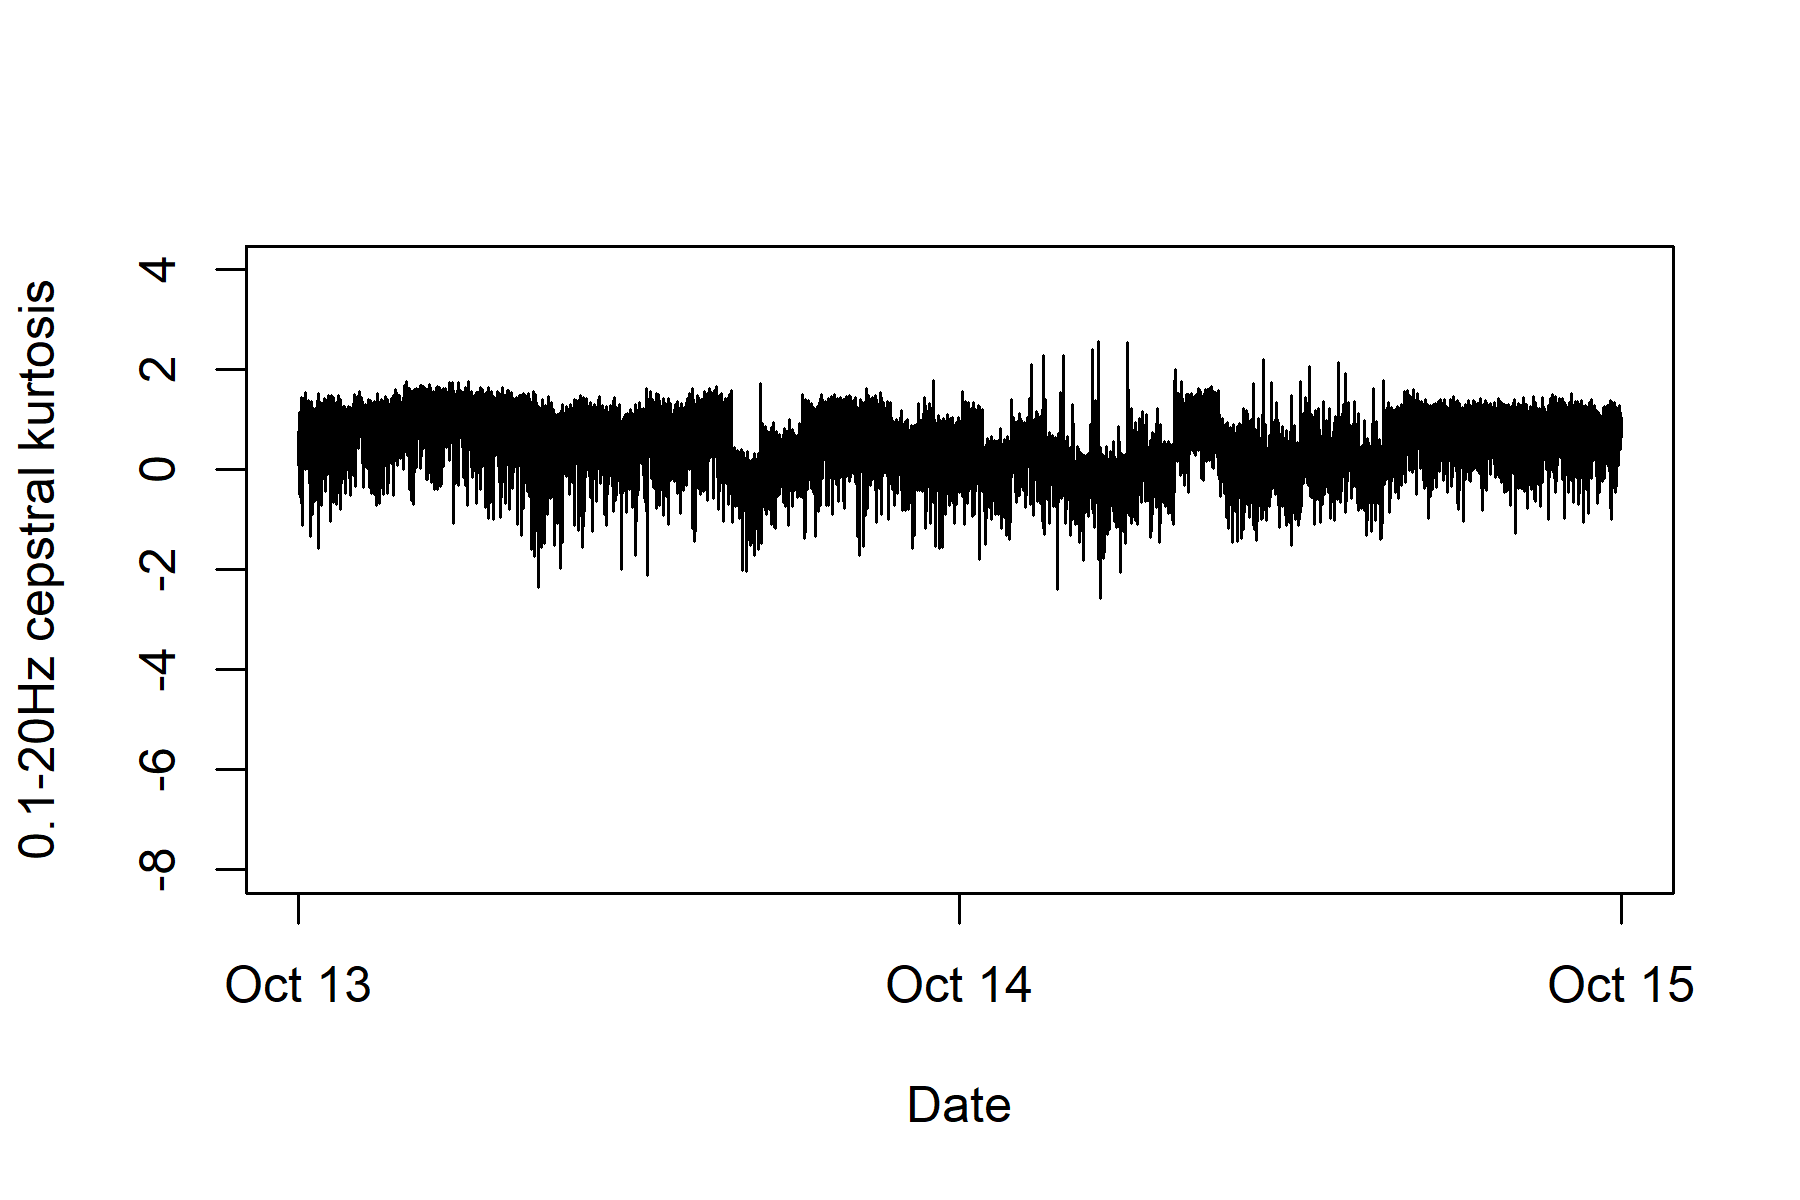}
}
\subfloat[Zoomed in]{\includegraphics[width=3.5in,valign=t]{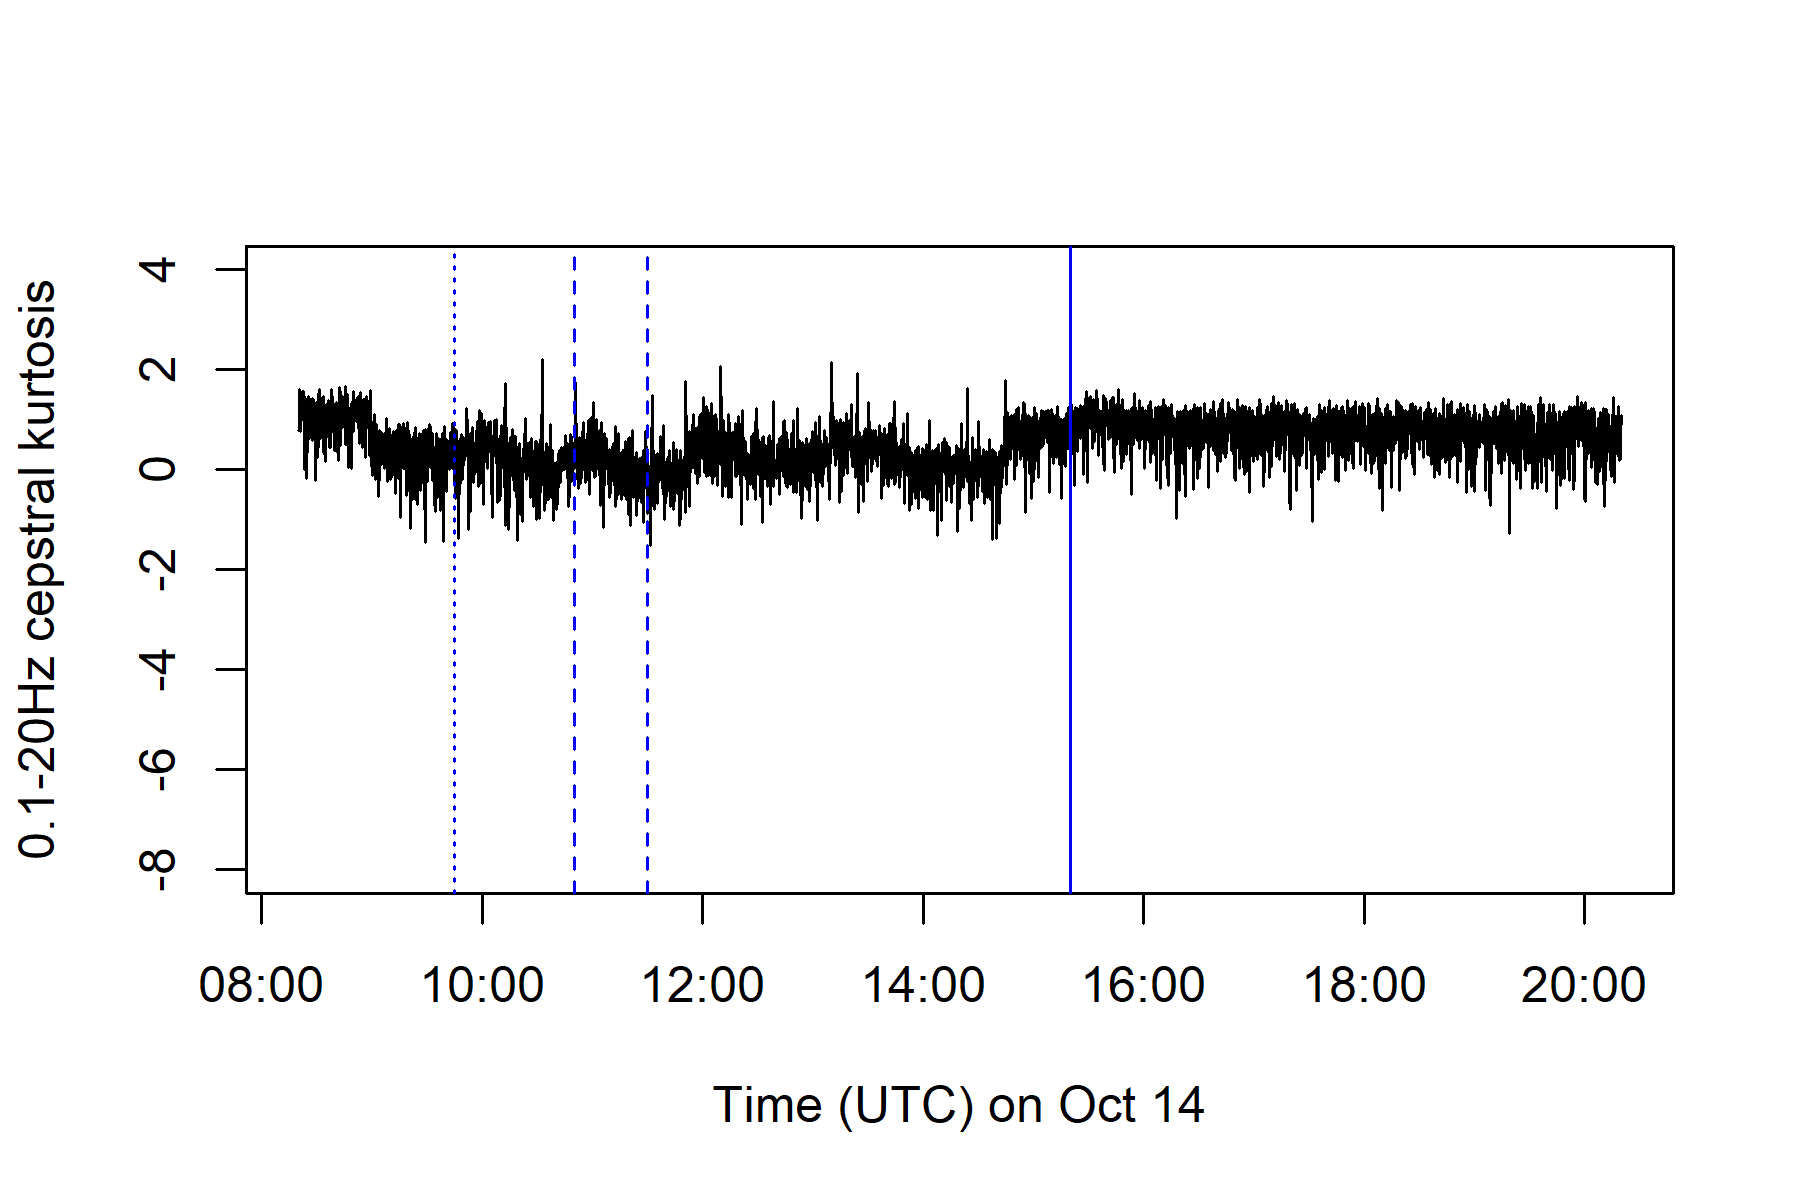}
}
\\
\subfloat[0.1-20Hz cepstral skewness]{\includegraphics[width=3.5in,valign=t]{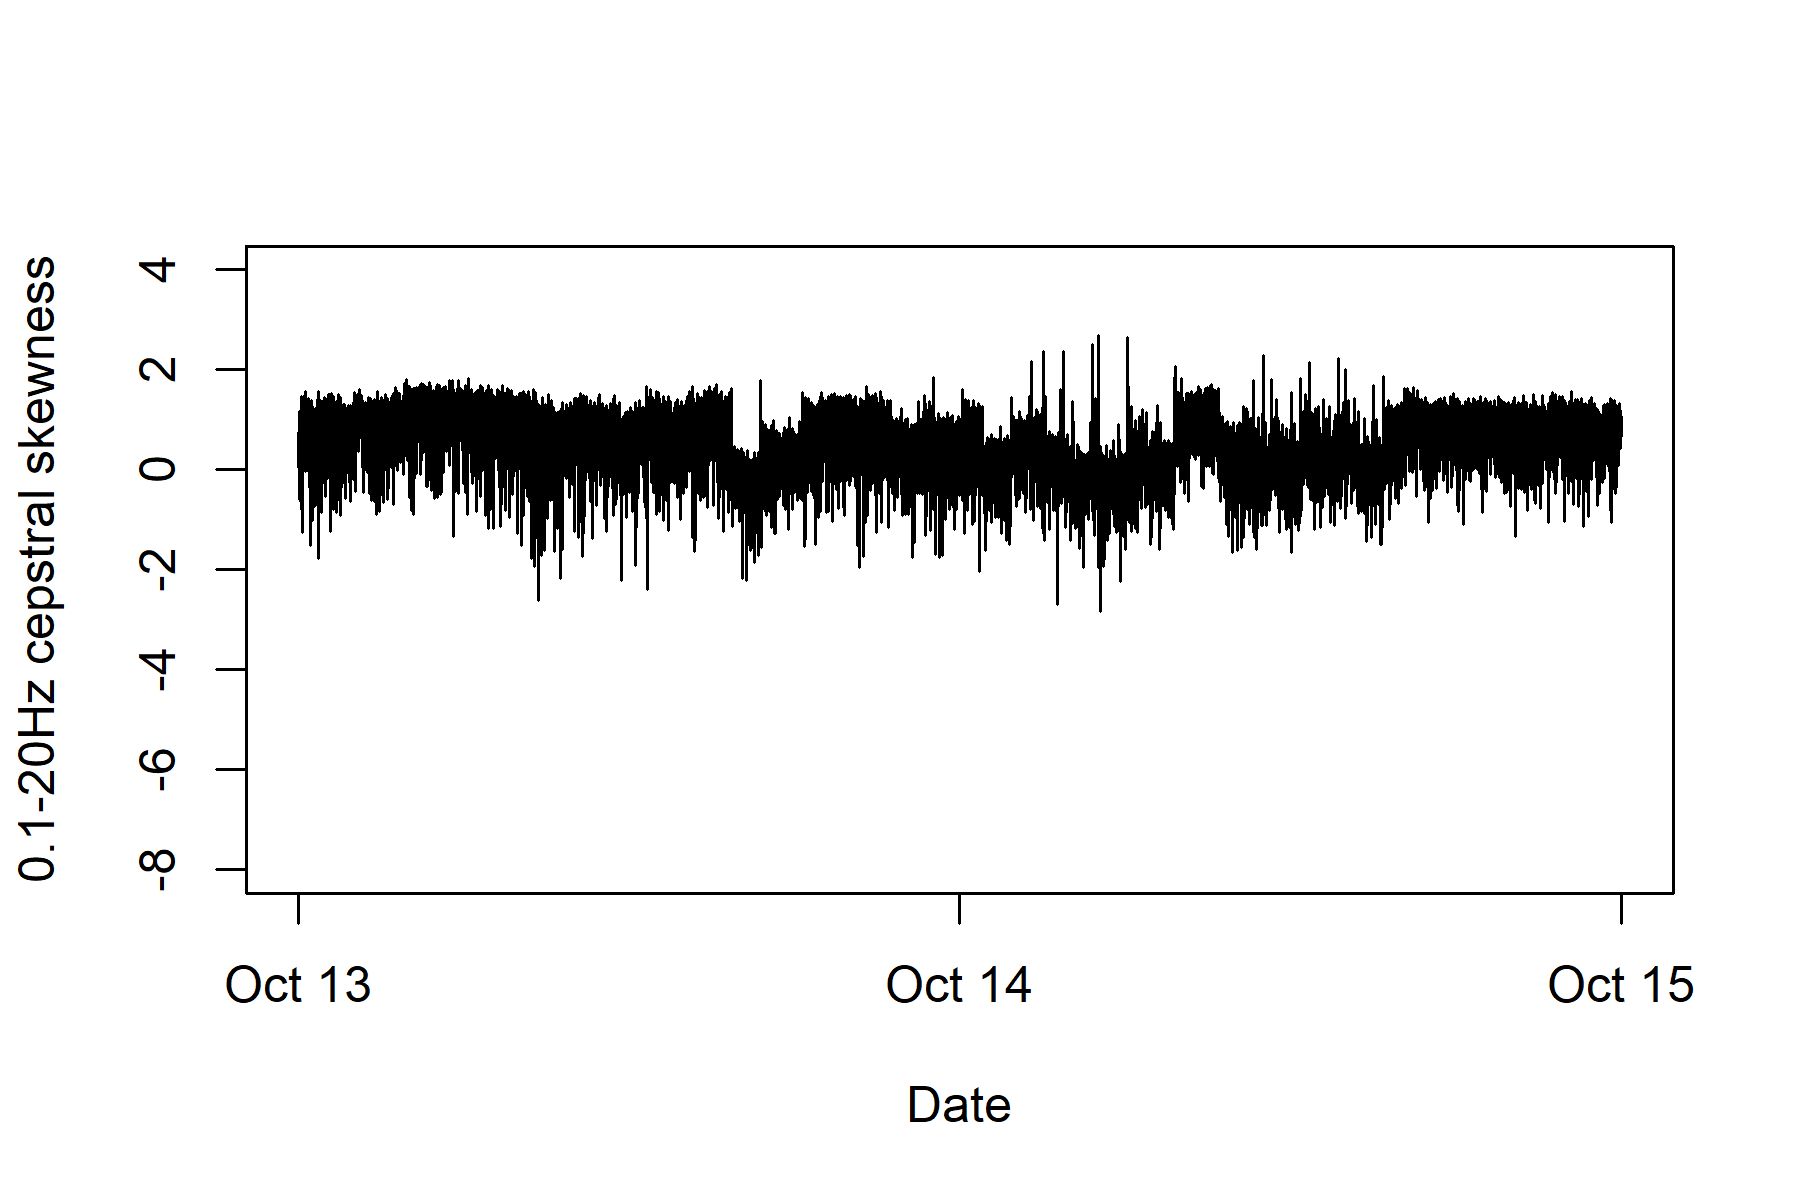}
}
\subfloat[Zoomed in]{\includegraphics[width=3.5in,valign=t]{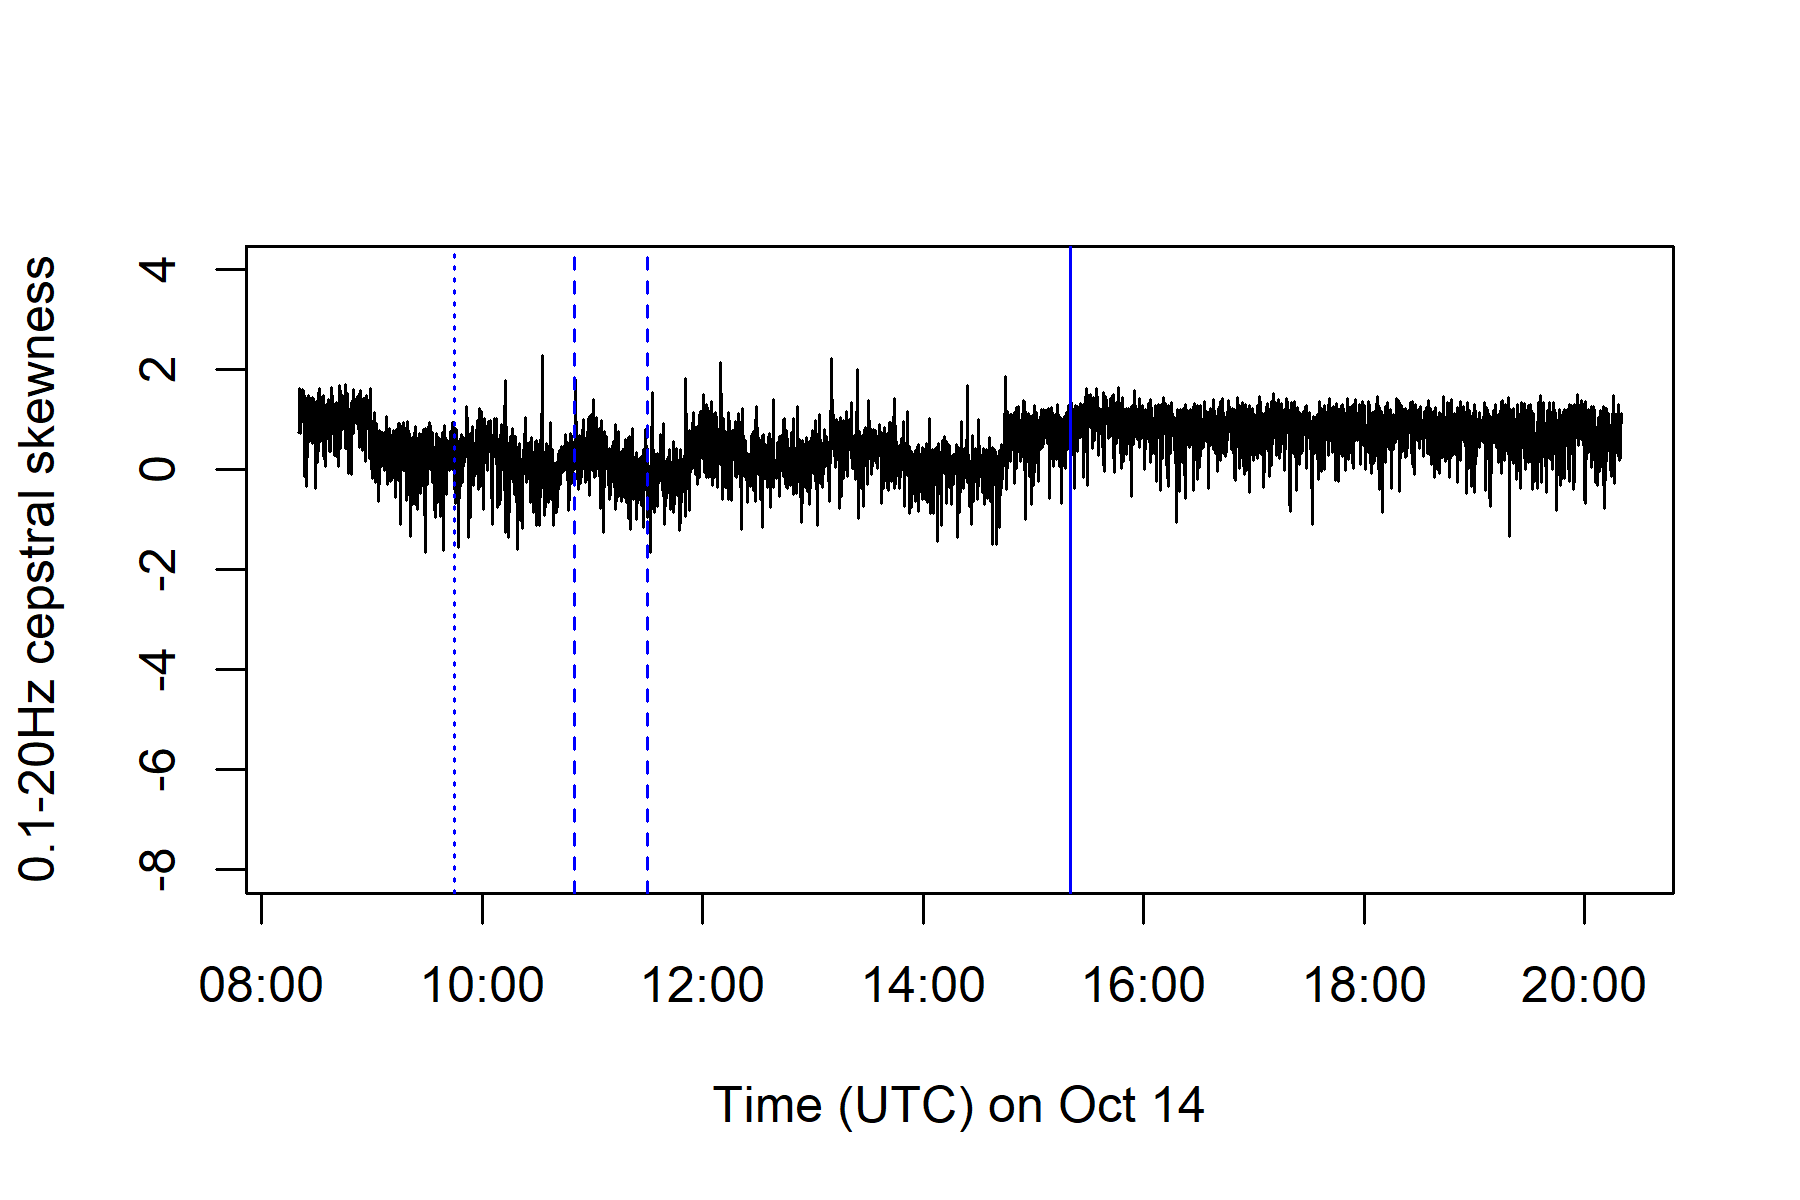}
}
\\
\subfloat[High pass 0.01Hz energy]{\includegraphics[width=3.5in,valign=t]{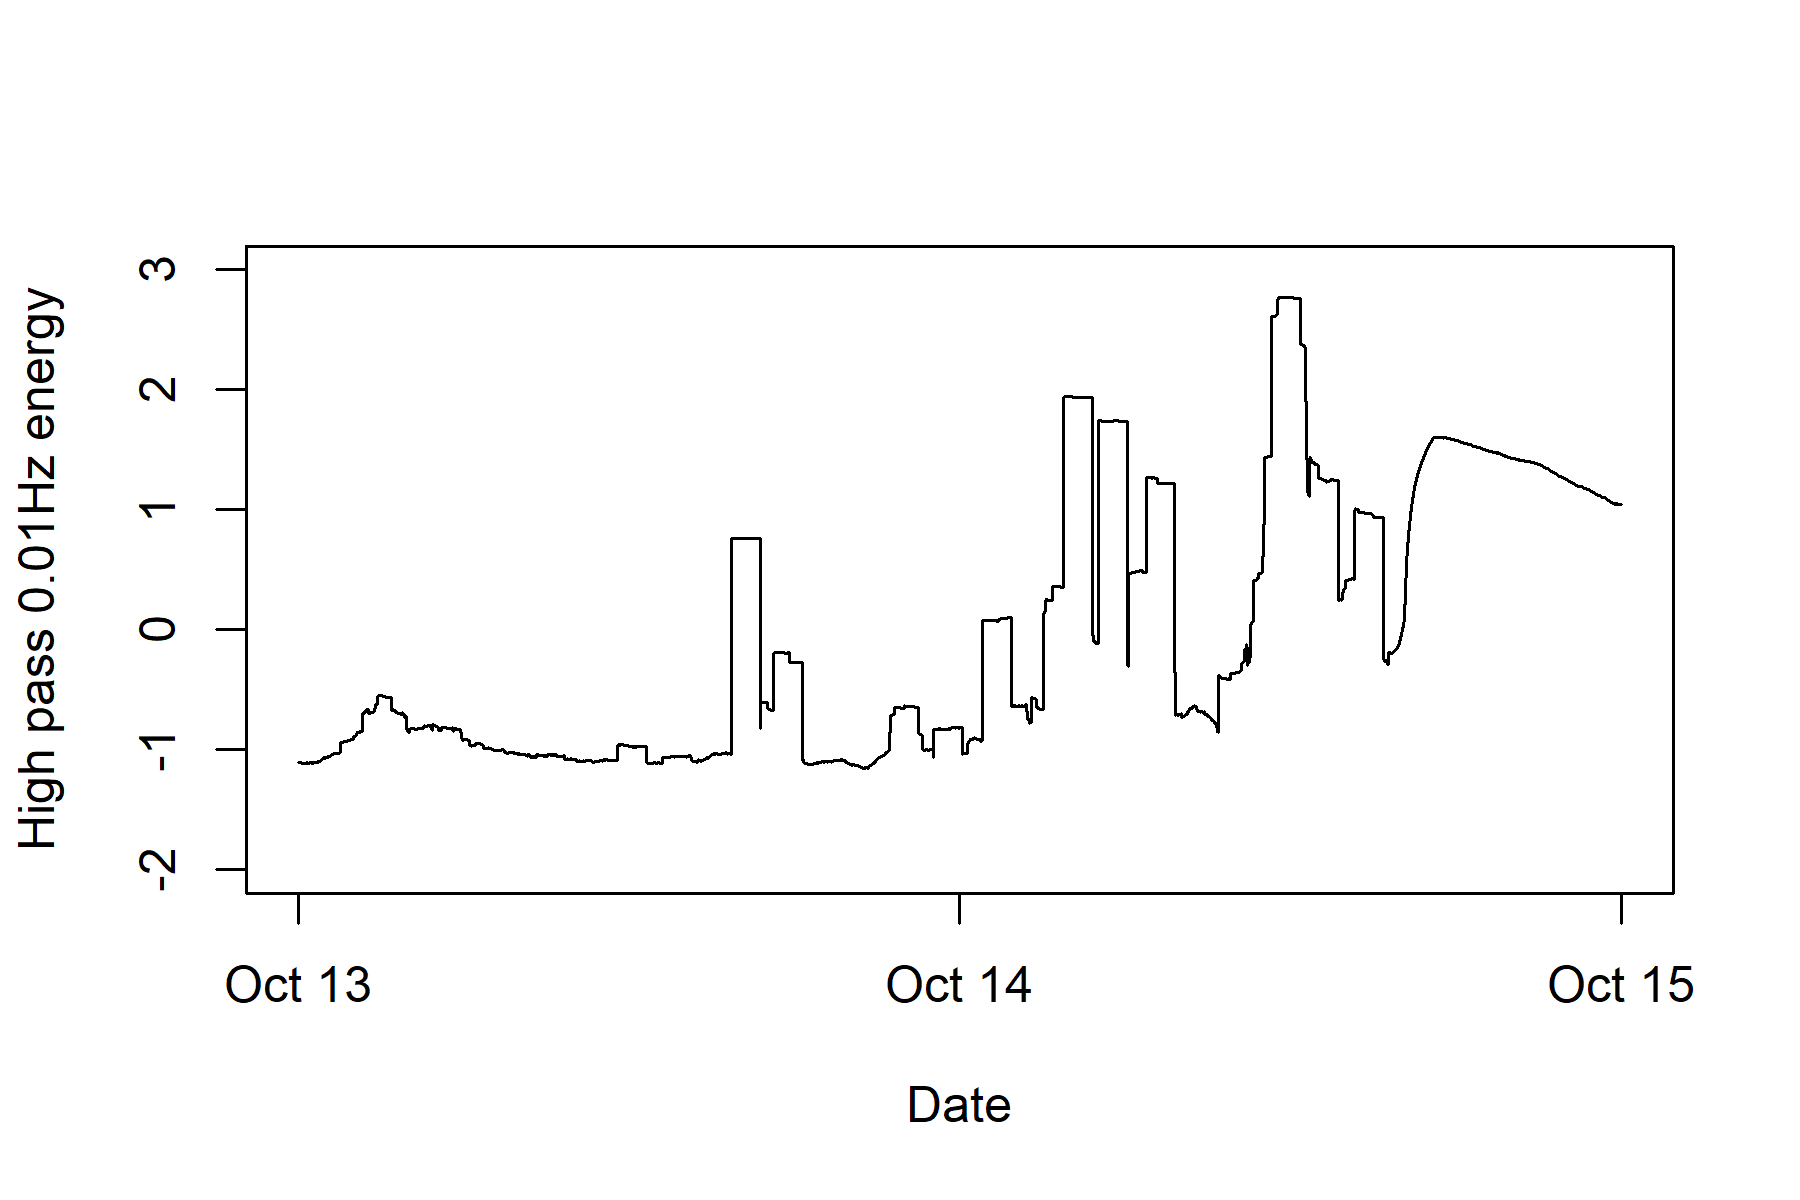}
}
\subfloat[Zoomed in]{\includegraphics[width=3.5in,valign=t]{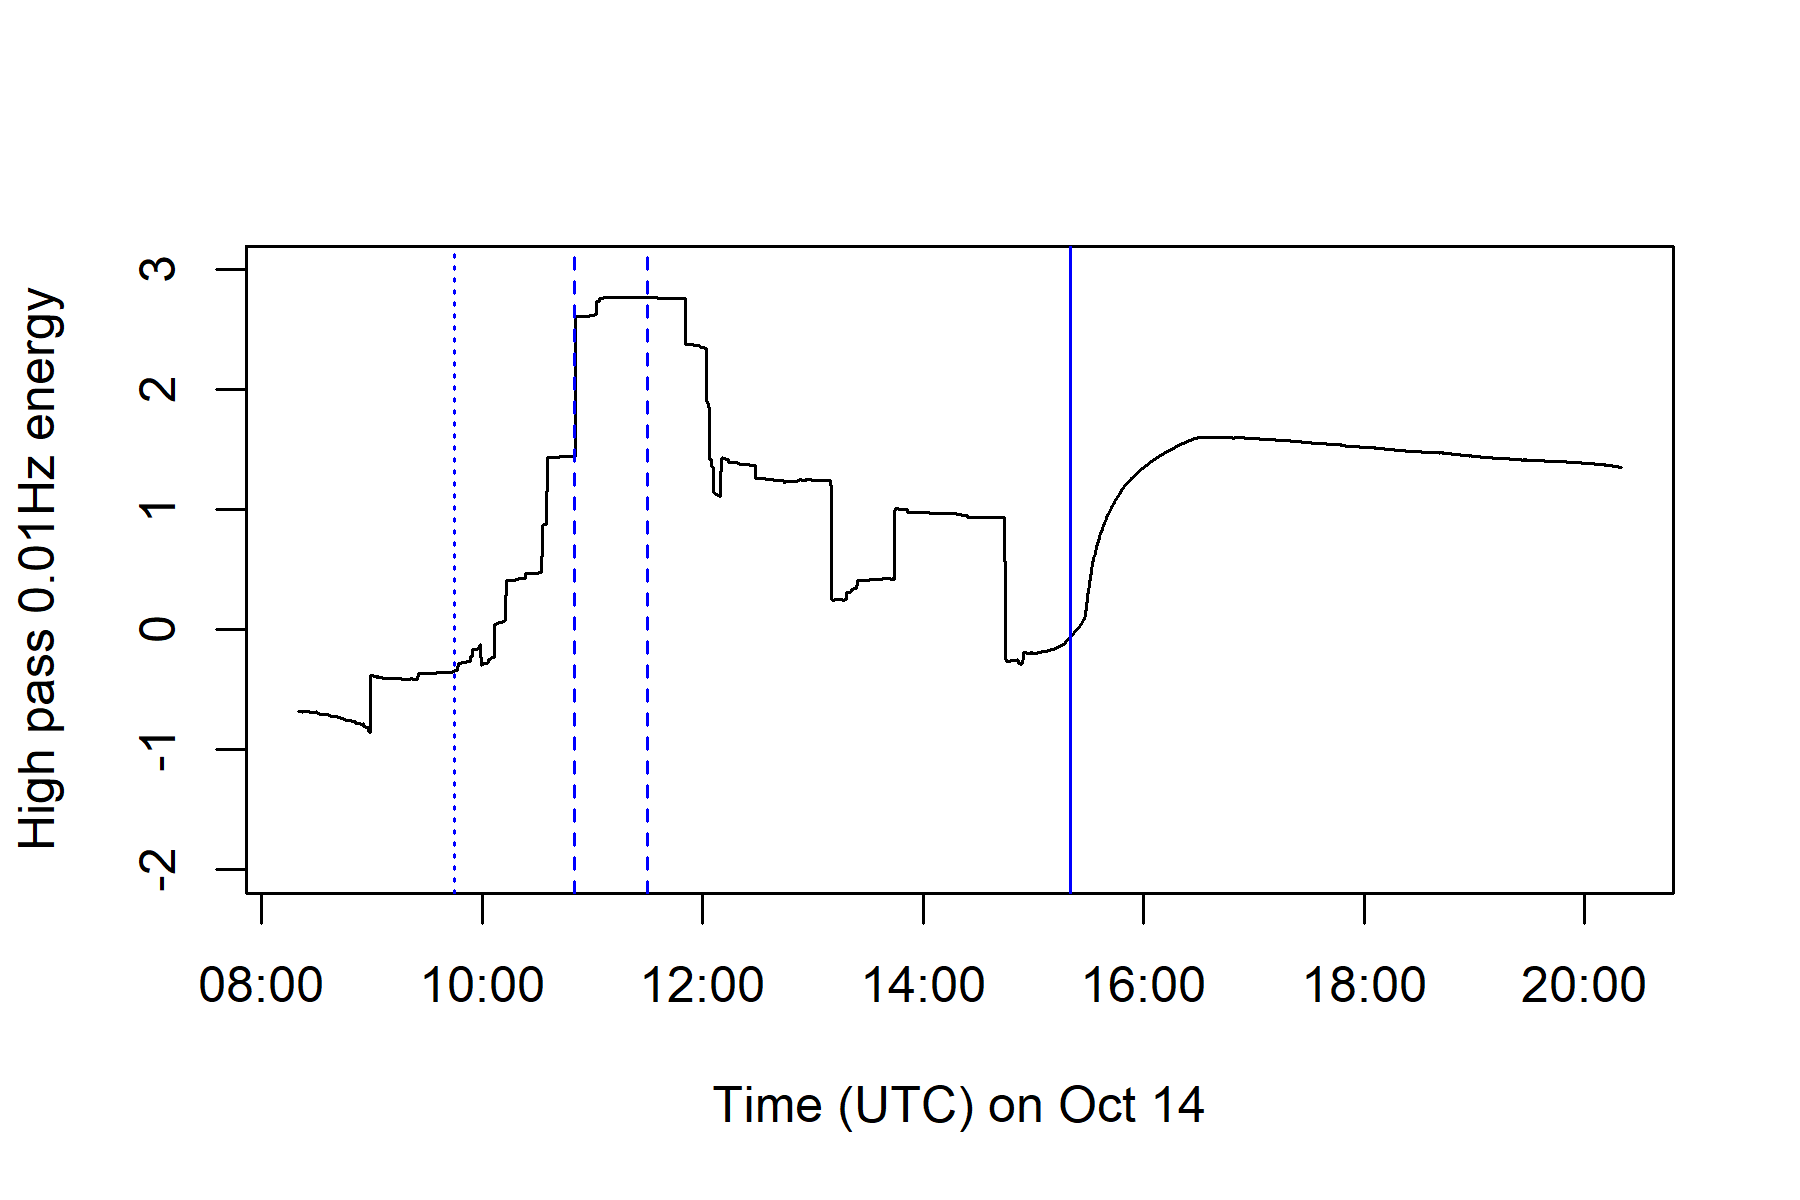}
}
\caption{Test event: Time series plots of the three major covariates in the logistic regression.}
\label{fig_test_covar}
\end{figure*}

\section{Results for the 5-15Hz envelope}

Similar results for the dynamic extreme value model were obtained for the 5-15Hz envelope. Figure \ref{fig:training_515} shows the one-hour ahead threshold exceedance forecasts for the three training events using the lowest threshold estimated across events for the 5-15Hz envelope index. Figure \ref{fig:test_515} shows that while sensible spikes in forecast probabilities in line with the eruption activity were observed for the test event, probability estimates remained low throughout the three non-events.

\begin{figure*}[!t]
\centering
\subfloat[Training event 1]{\includegraphics[width=3.5in,valign=t]{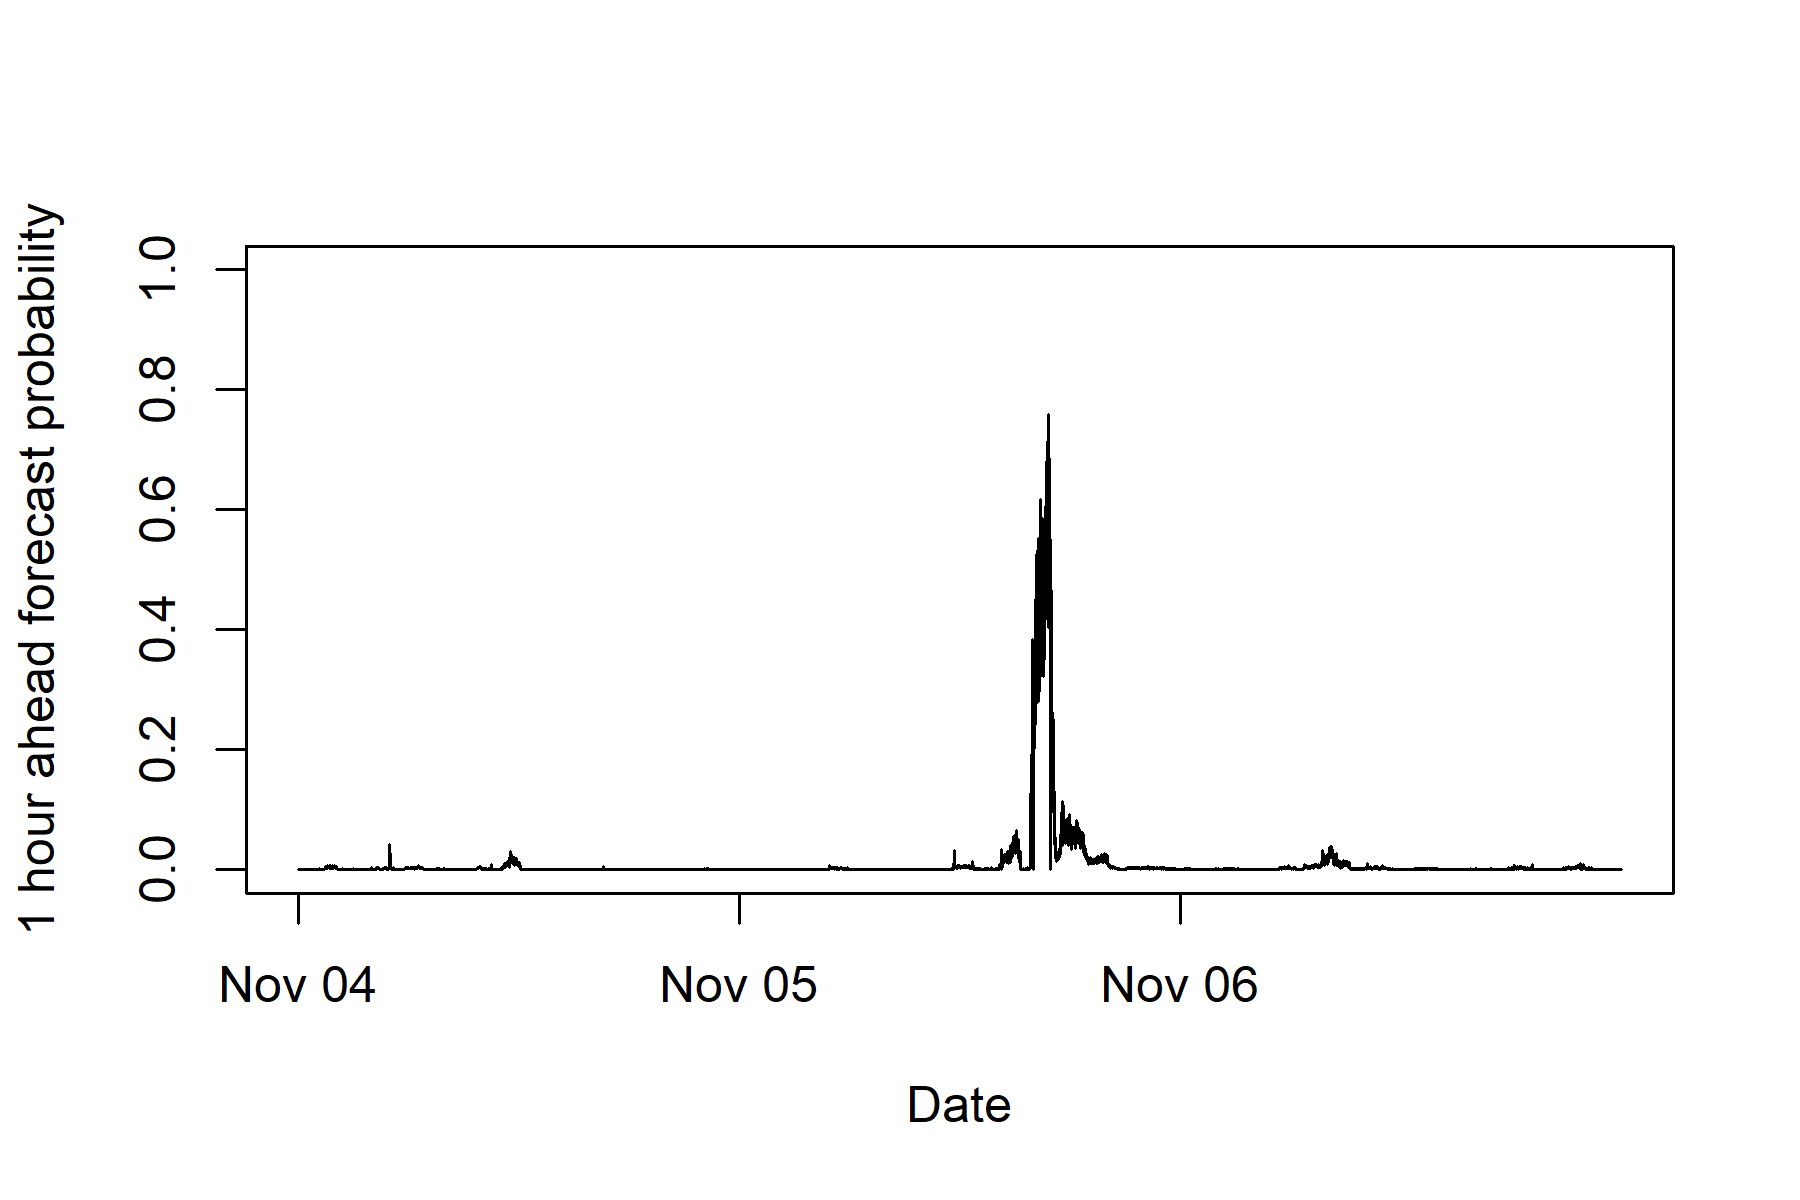}}
\subfloat[Zoomed in]{\includegraphics[width=3.5in,valign=t]{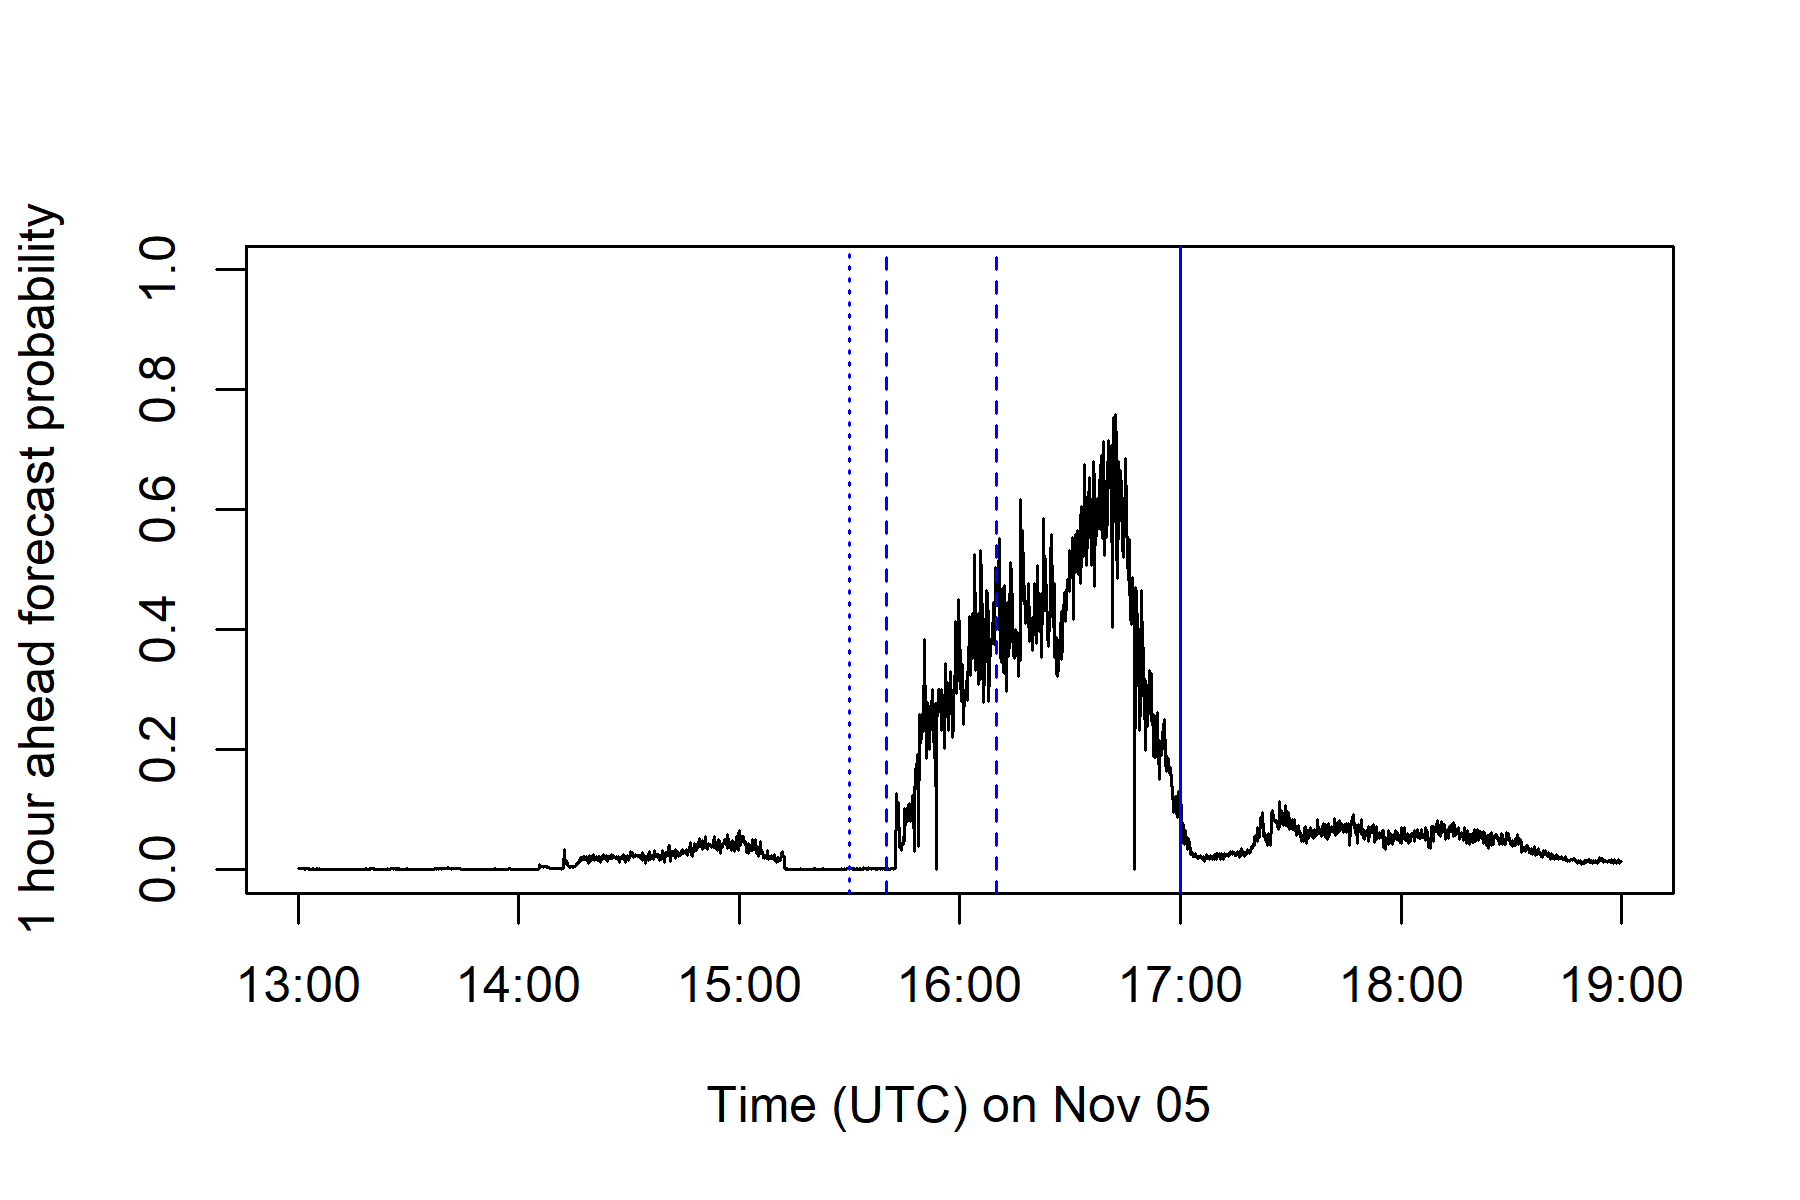}
}
\\
\subfloat[Training event 2]{\includegraphics[width=3.5in,valign=t]{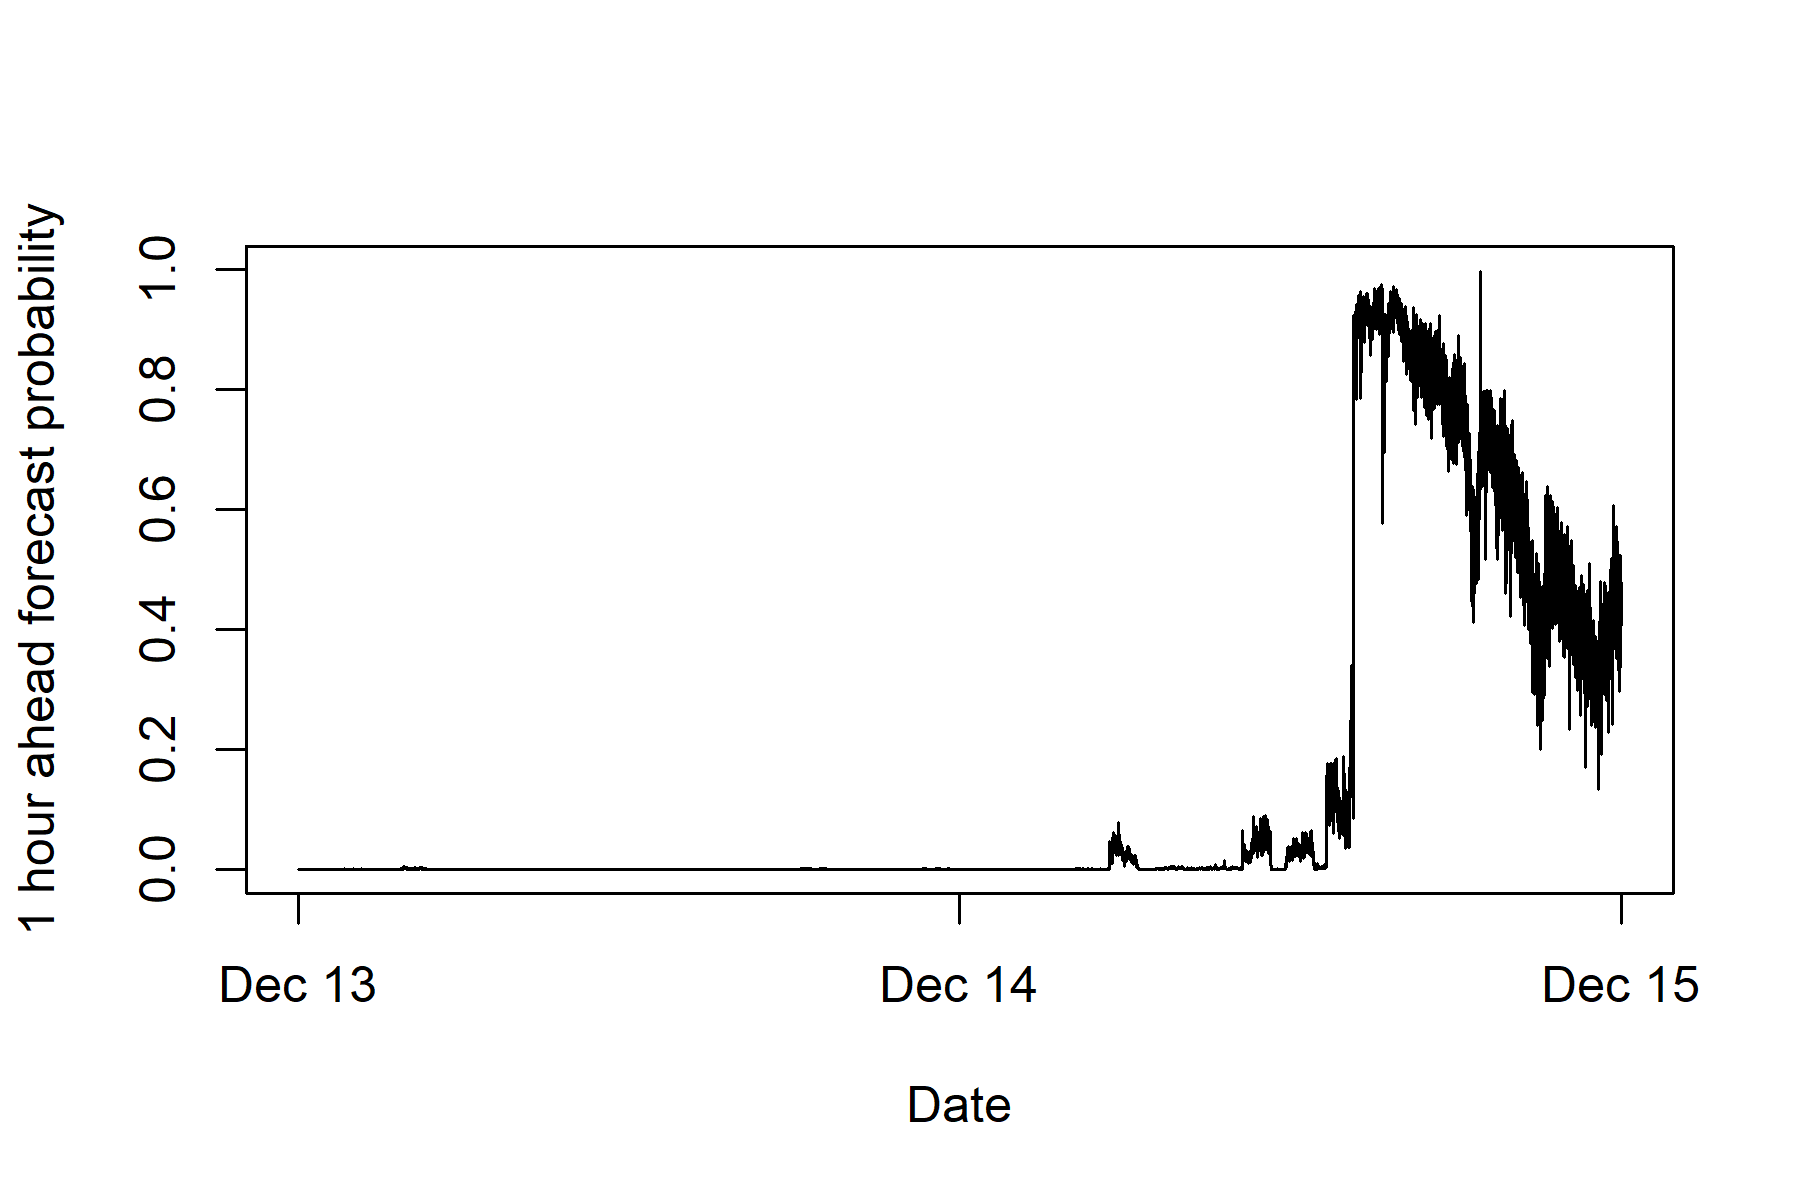}}
\subfloat[Zoomed in]{\includegraphics[width=3.5in,valign=t]{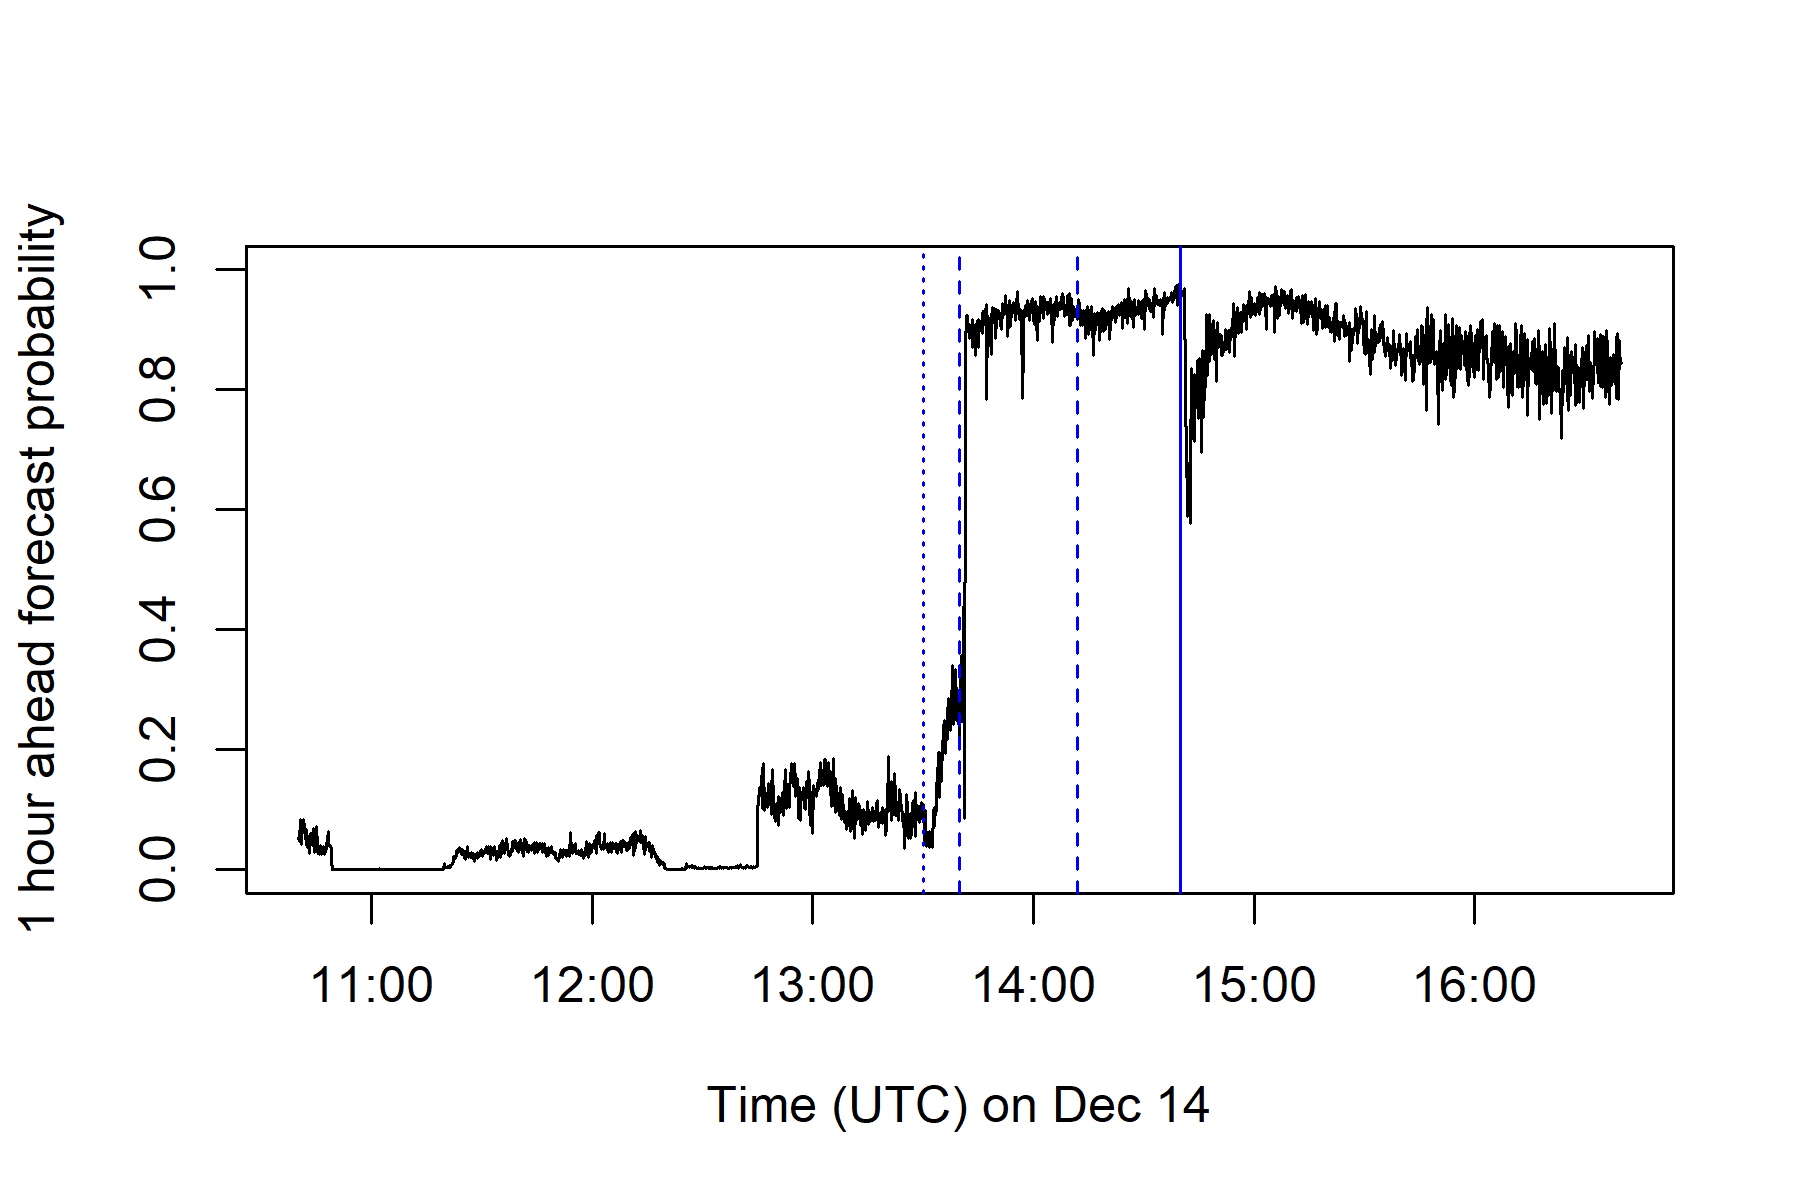}}
\\
\subfloat[Training event 3]{\includegraphics[width=3.5in,valign=t]{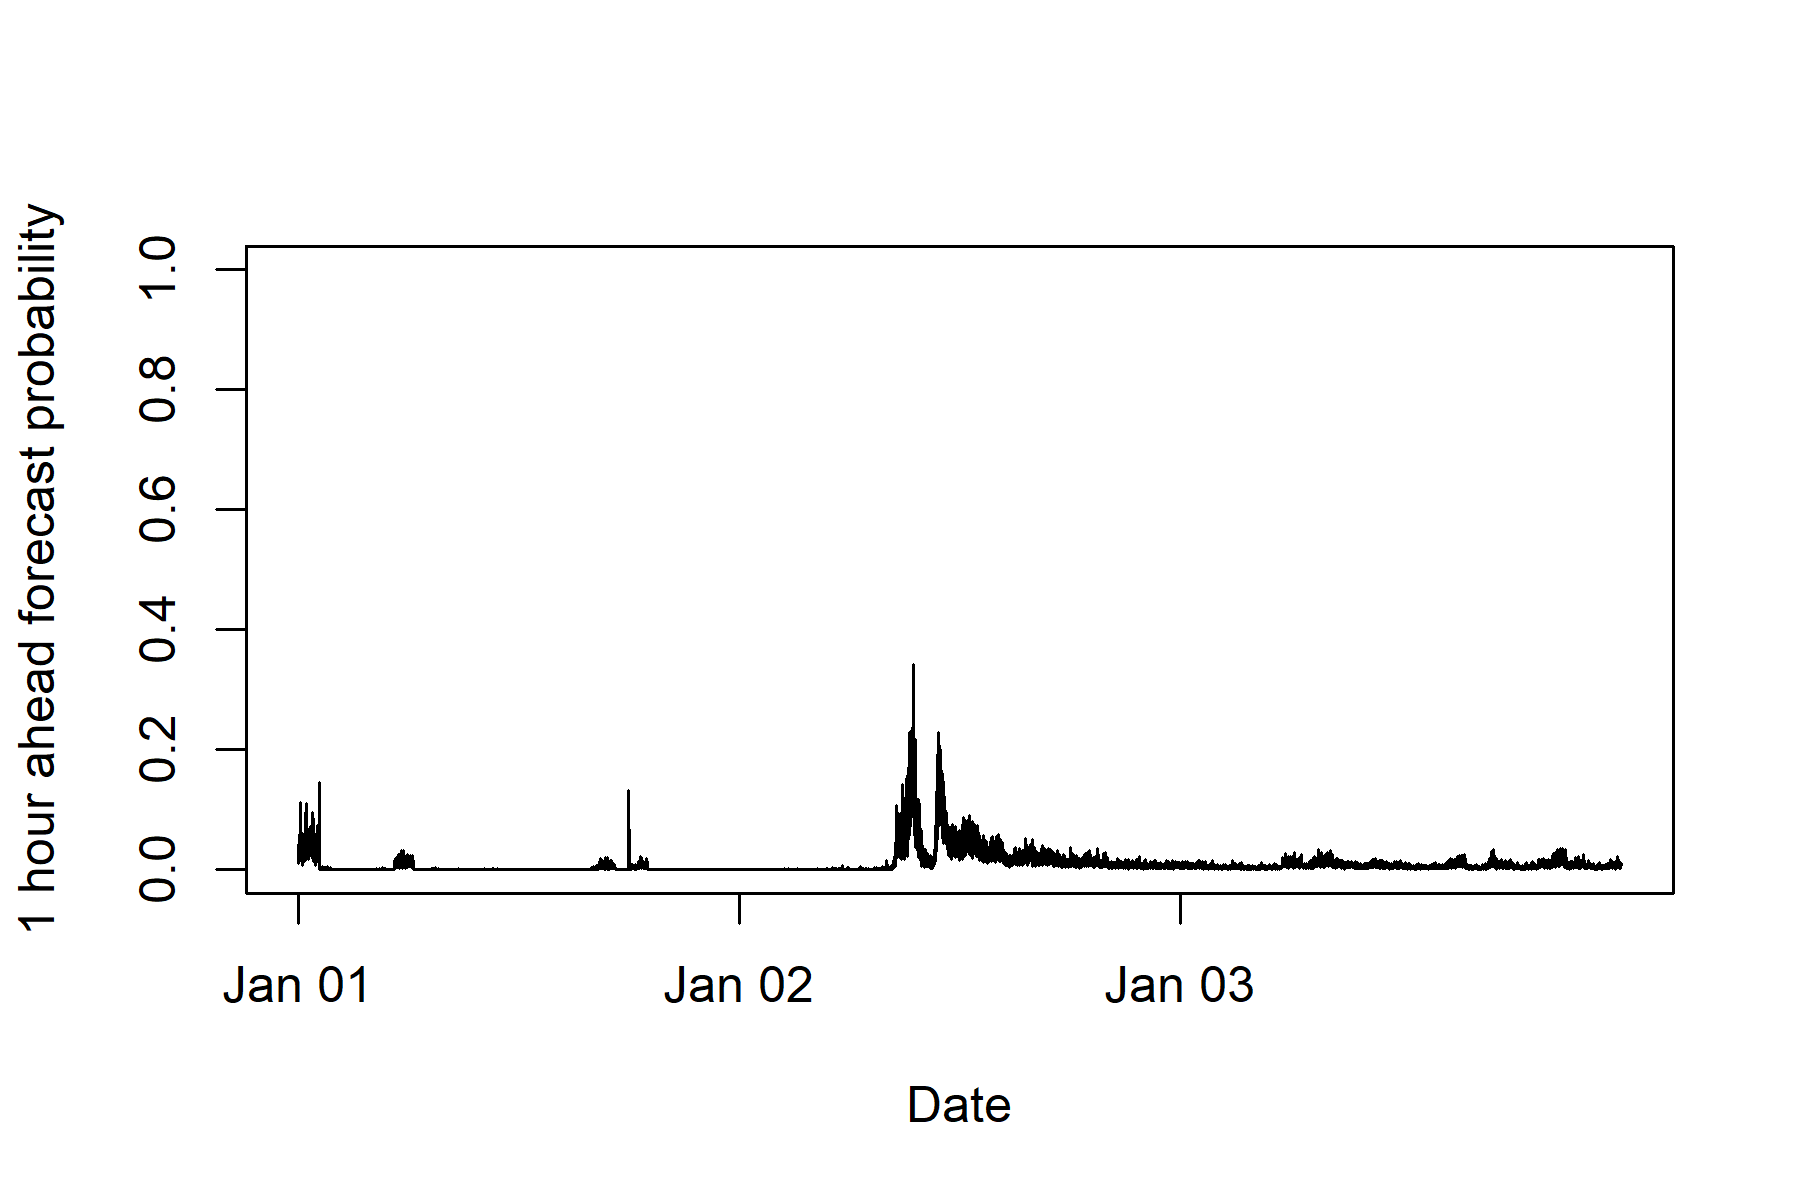}}
\subfloat[Zoomed in]{\includegraphics[width=3.5in,valign=t]{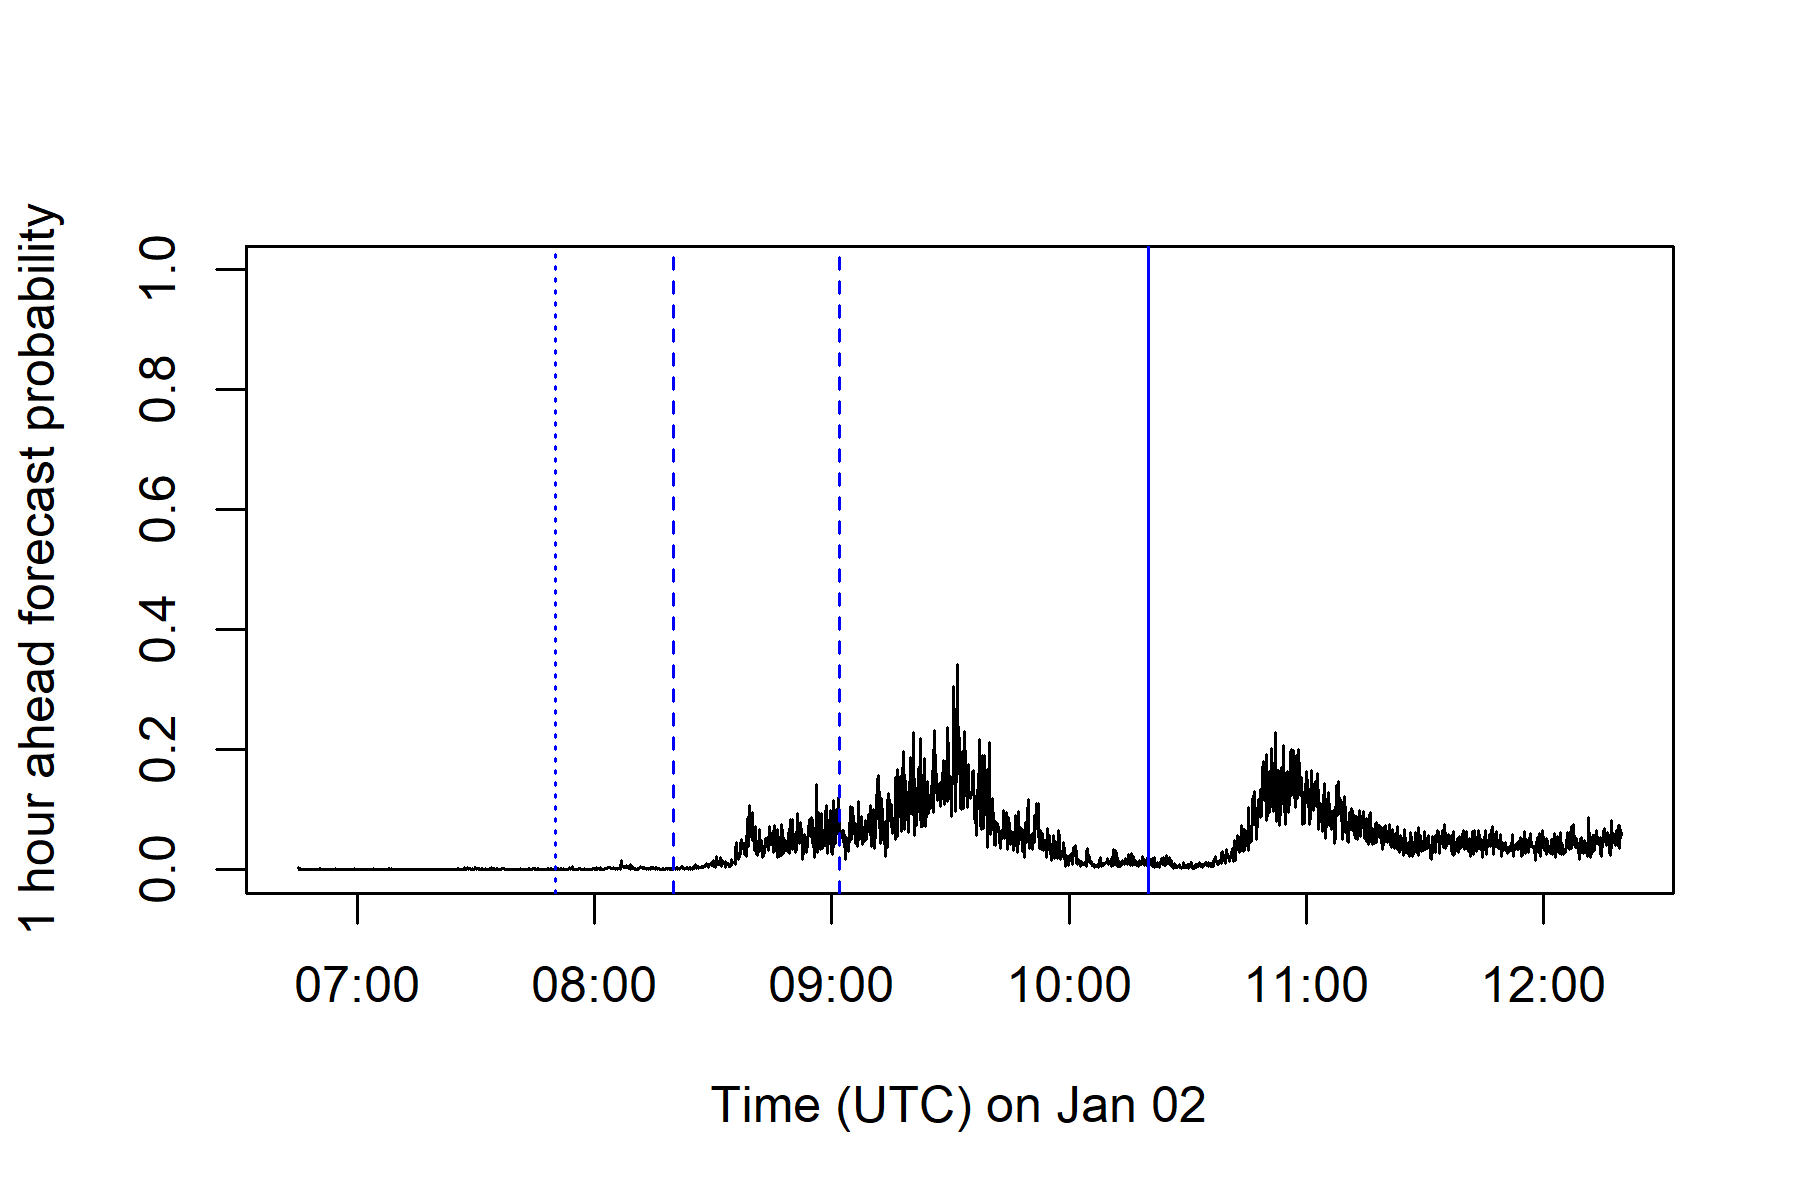}}

\caption{5-15Hz envelope index: One-hour ahead threshold exceedance forecasts for the three training events using the lowest threshold estimated across events. The dotted, dashed and bold blue vertical lines denote the times of the seismic crises, start and end of the seismic swarms and the eruption onset respectively.}
\label{fig:training_515}
\end{figure*}

\begin{figure*}[!t]
\centering
\subfloat[Test event]{\includegraphics[width=3.5in,valign=t]{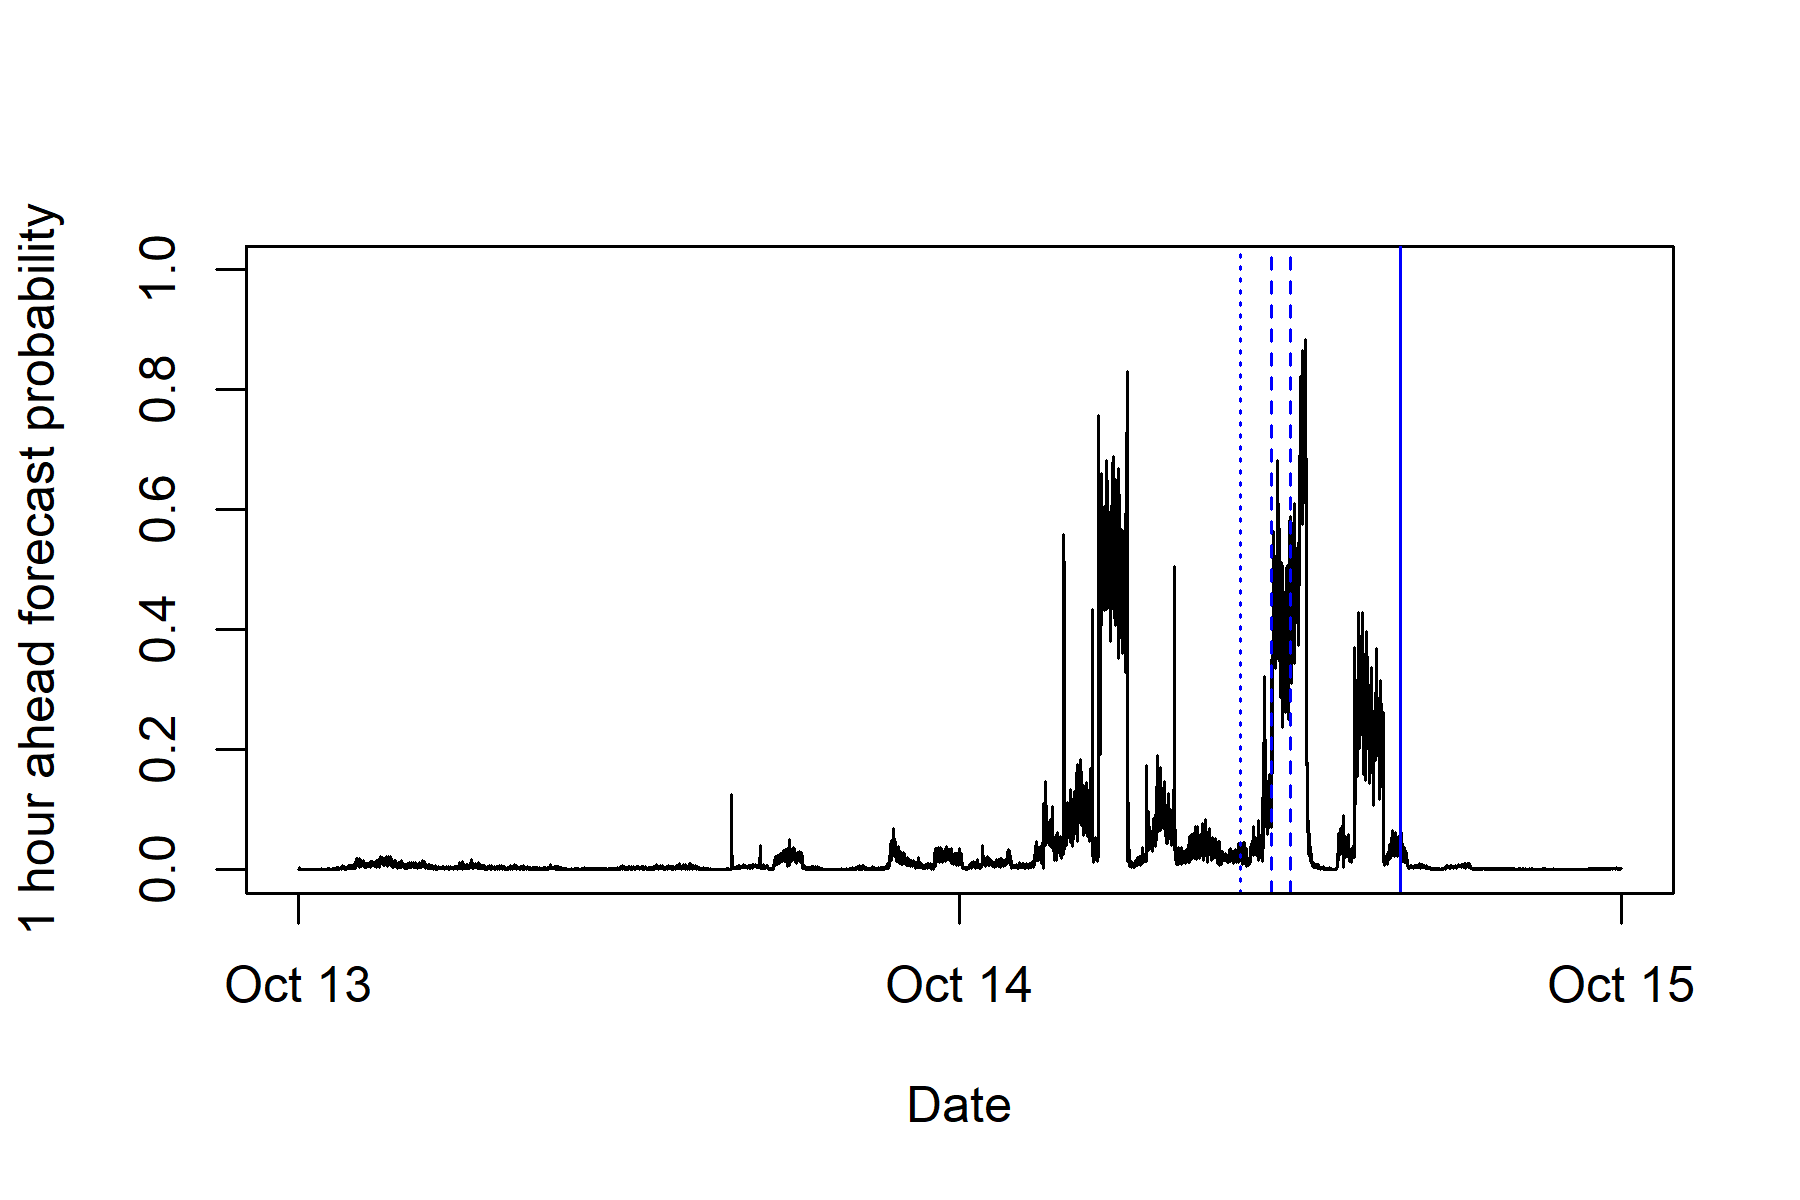}}
\subfloat[Test non-event 1]{\includegraphics[width=3.5in,valign=t]{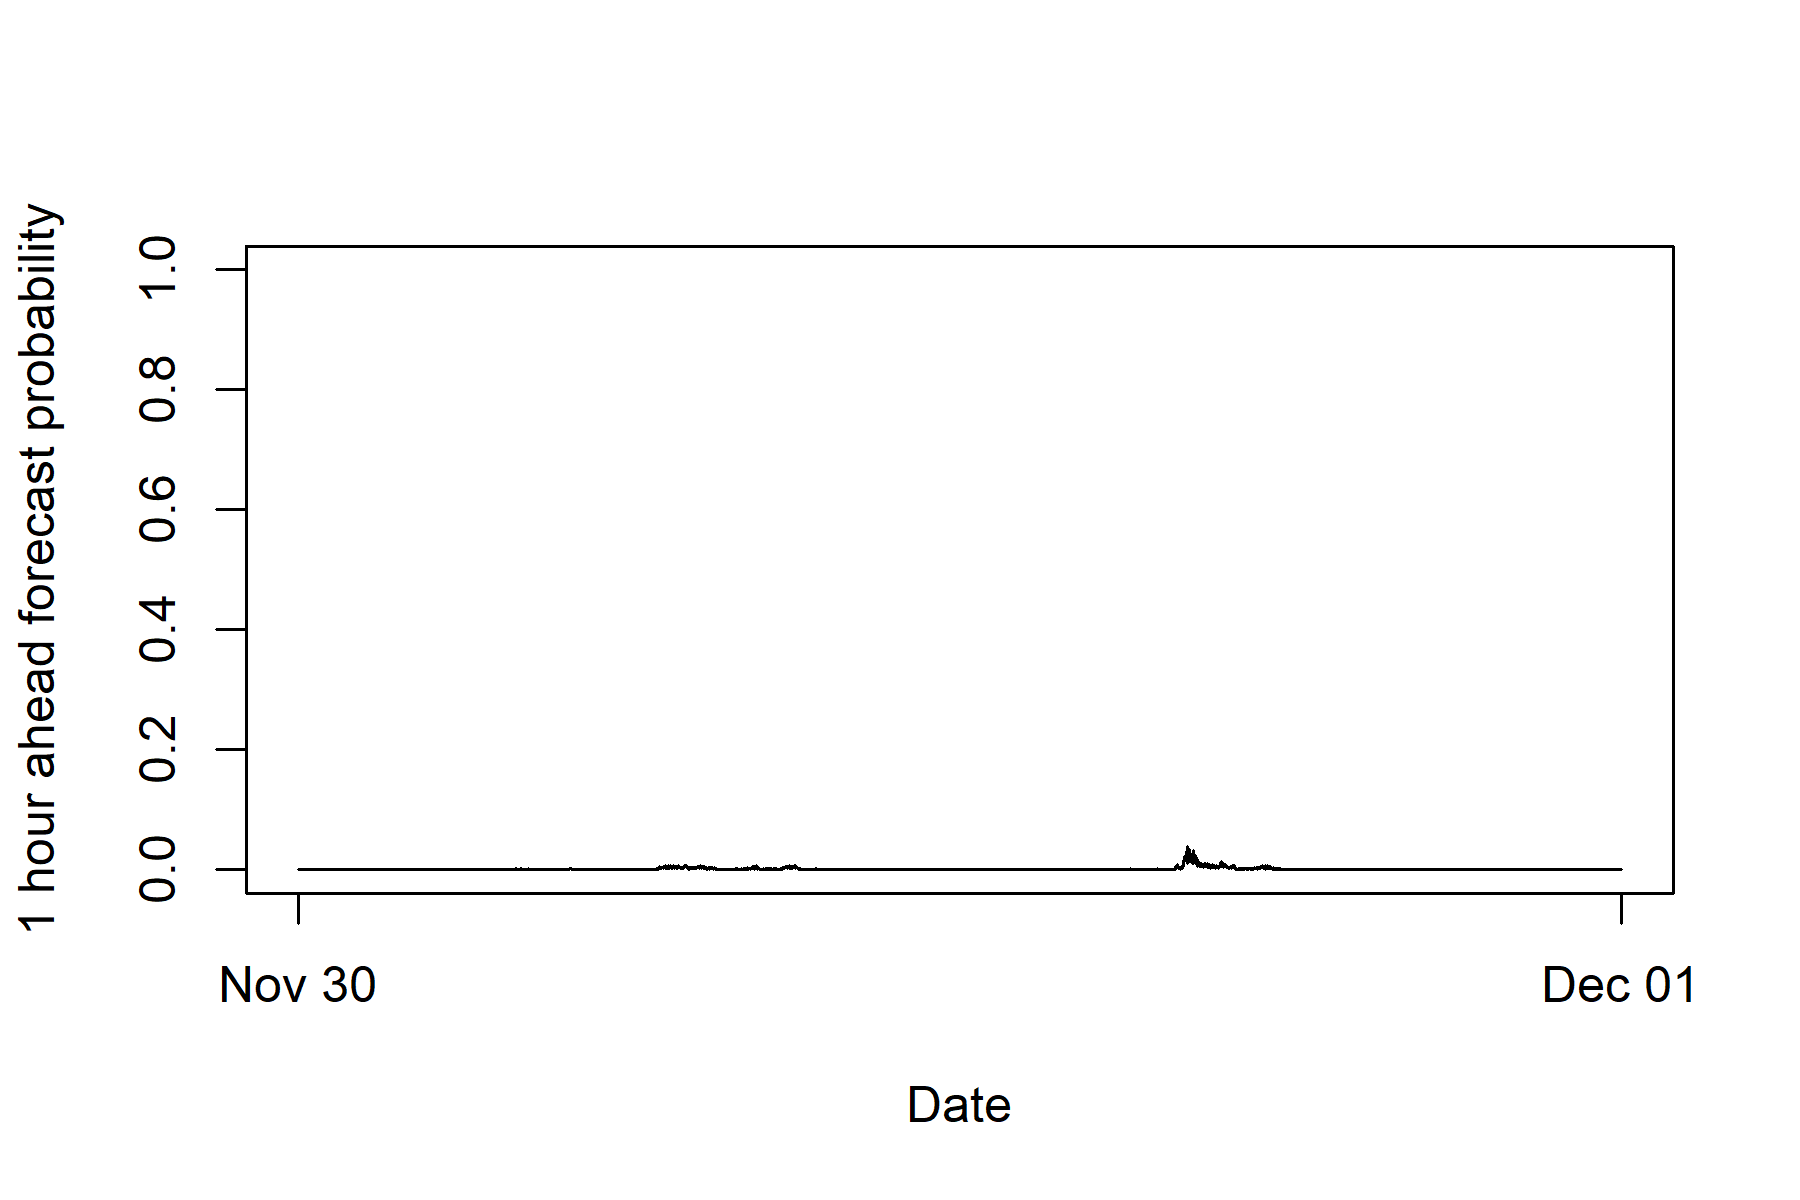}}
\\
\subfloat[Test non-event 2]{\includegraphics[width=3.5in,valign=t]{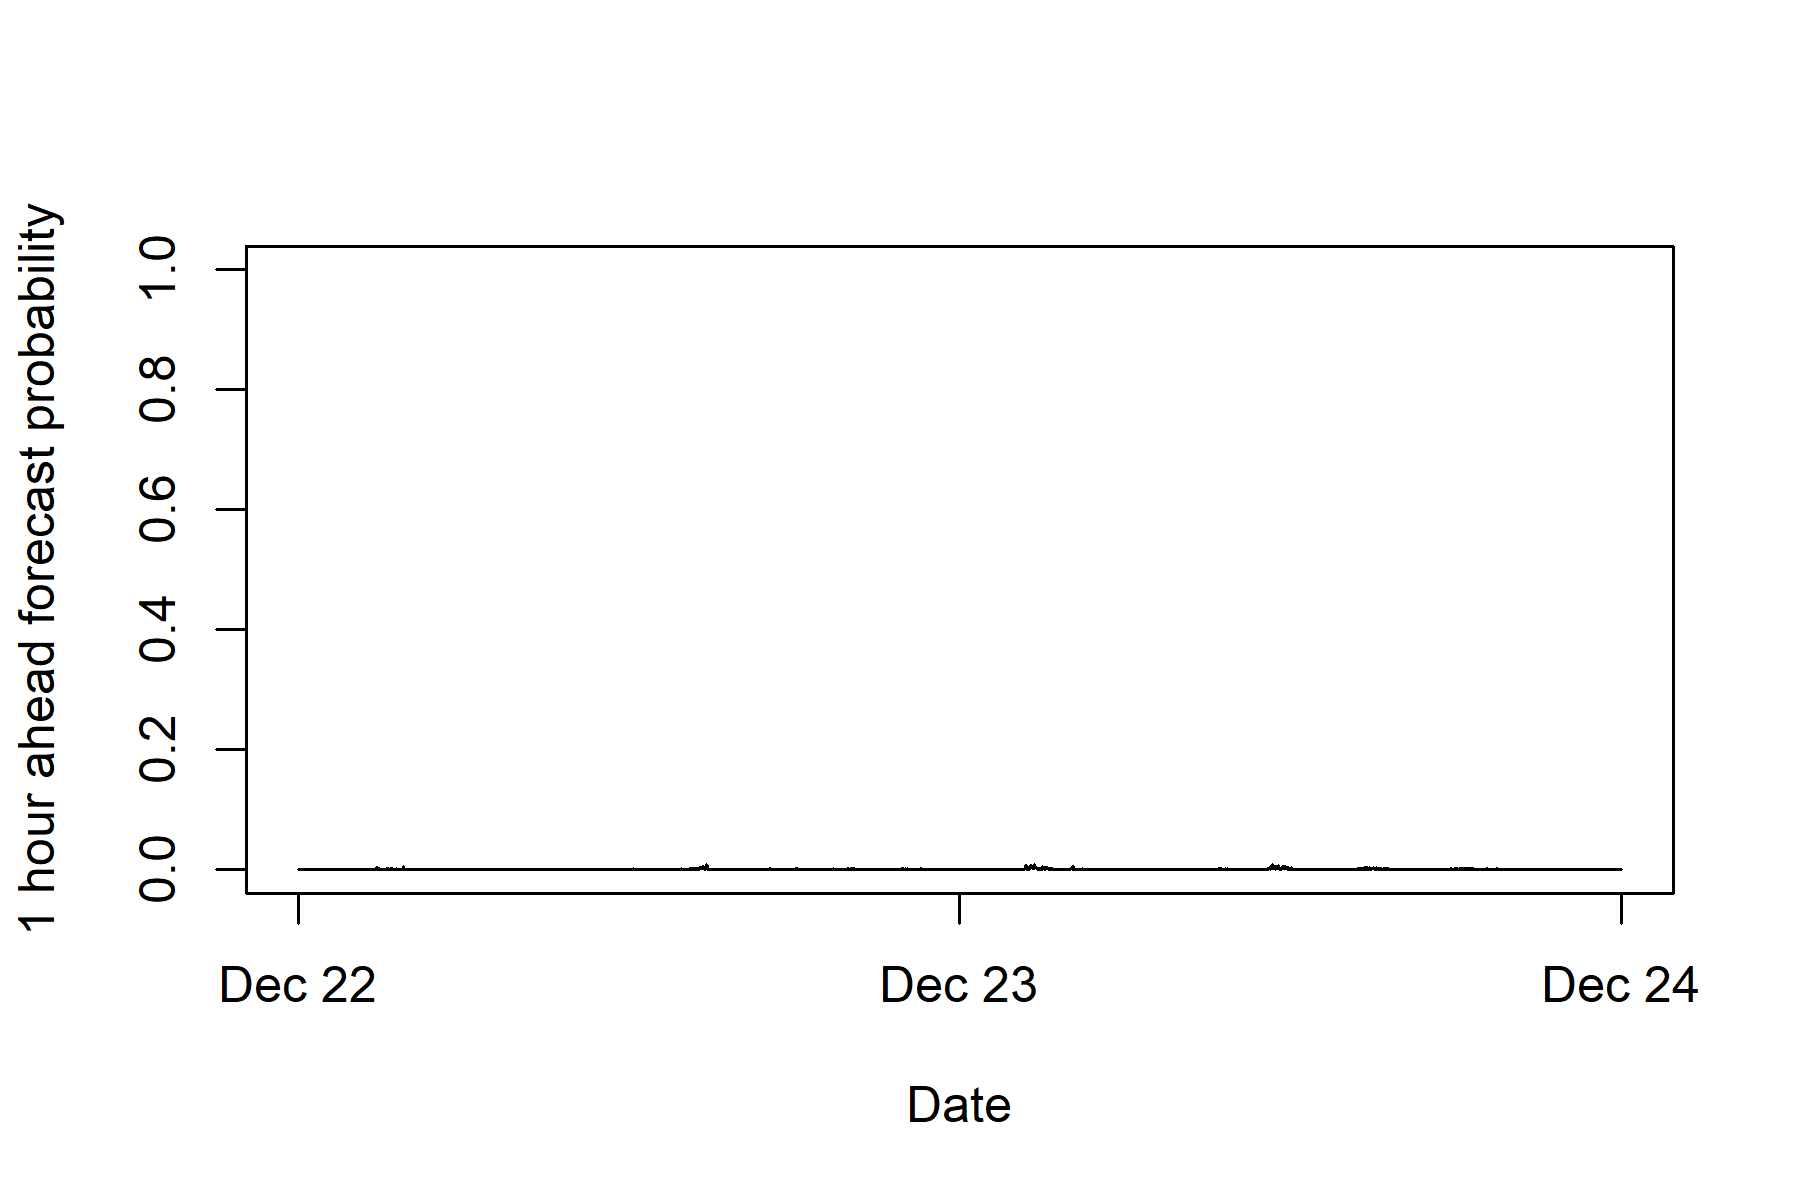}}
\subfloat[Test non-event 3]{\includegraphics[width=3.5in,valign=t]{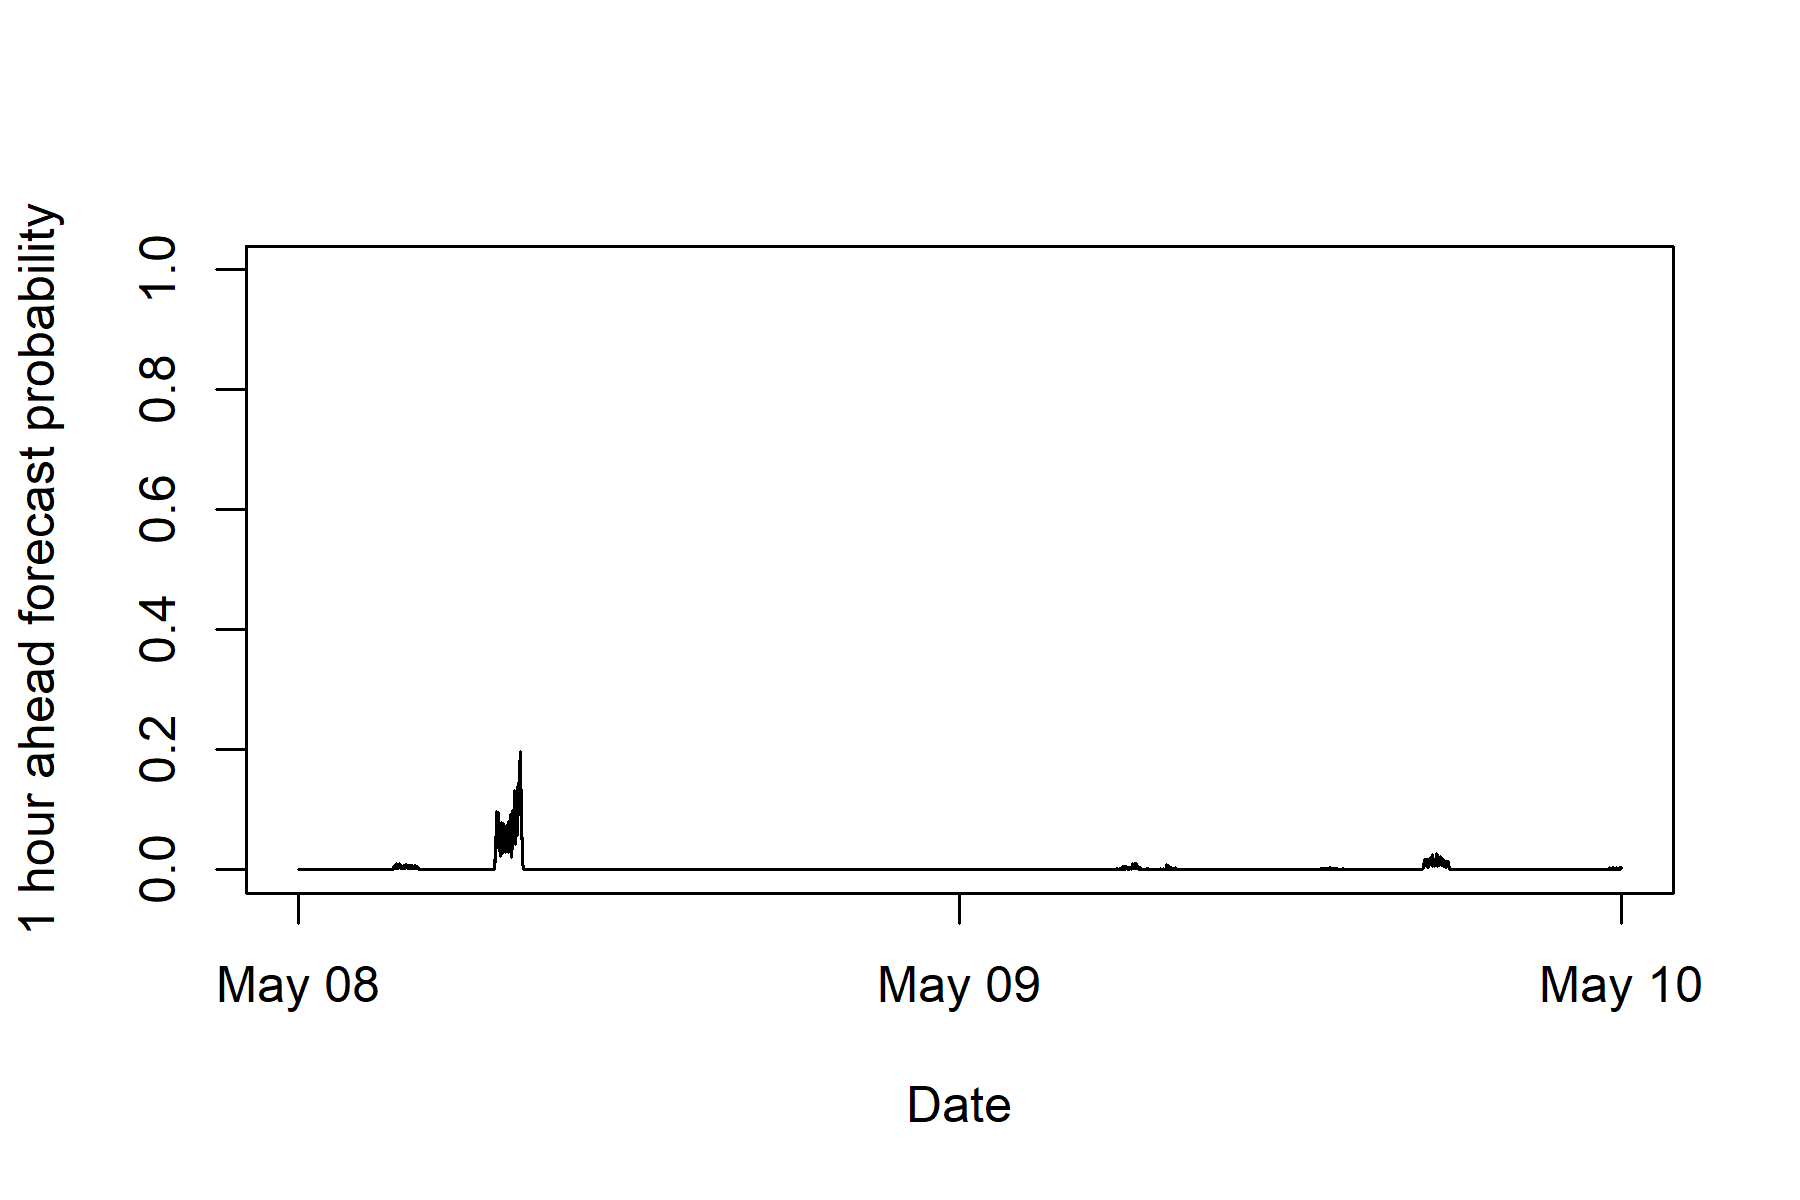}}
\caption{5-15Hz envelope index: One-hour ahead threshold exceedance forecasts using the lowest threshold estimated across events for: (a) the test event, (b)-(d) the test non-events. The dotted, dashed and bold blue vertical lines in Plot (a) denote the times of the seismic crisis, seismic swarm and the eruption onset respectively.}
\label{fig:test_515}
\end{figure*}

% Can use something like this to put references on a page
% by themselves when using endfloat and the captionsoff option.
\ifCLASSOPTIONcaptionsoff
  \newpage
\fi

% trigger a \newpage just before the given reference
% number - used to balance the columns on the last page
% adjust value as needed - may need to be readjusted if
% the document is modified later
%\IEEEtriggeratref{8}
% The "triggered" command can be changed if desired:
%\IEEEtriggercmd{\enlargethispage{-5in}}

% references section

% can use a bibliography generated by BibTeX as a .bbl file
% BibTeX documentation can be easily obtained at:
% http://mirror.ctan.org/biblio/bibtex/contrib/doc/
% The IEEEtran BibTeX style support page is at:
% http://www.michaelshell.org/tex/ieeetran/bibtex/
\bibliographystyle{IEEEtran}
% argument is your BibTeX string definitions and bibliography database(s)
\bibliography{references}
\end{document}
